# Supplementary material for: Bayesian Instrumented Directed Graphical Models for Cyclic Causal Discovery with Unmeasured Confounding
Source: arXiv:2510.09991 source file (2026-11-25)
Supplement: Supplementary file 1 [file Supplementary.tex]

\documentclass[11pt]{article}

% --- Packages ---
\usepackage[margin=1in]{geometry}
\usepackage{amsmath, amssymb, amsfonts, bm}
\usepackage{graphicx}
\usepackage{float}
\usepackage{natbib}
\usepackage{booktabs}
\usepackage{siunitx}
\usepackage{caption}
\usepackage{subcaption}
\usepackage{multirow}
\usepackage{hyperref}
\usepackage{placeins}
% --- theorem + proof support ---
\usepackage{amsthm}

% --- operators ---
\DeclareMathOperator{\vect}{vec}
\DeclareMathOperator{\diag}{diag}
\DeclareMathOperator{\supp}{supp}
\DeclareMathOperator{\rank}{rank}

% --- theorem environments ---
\theoremstyle{plain}

\newtheorem{lemma}{Lemma}

\theoremstyle{definition}
\newtheorem{example}{Example}

\theoremstyle{remark}
\newtheorem{remark}{Remark}

% \usepackage{lineno}
% \linenumbers        % turn on line numbering

\usepackage{authblk} % put in the preamble

\title{Supplementary Material: Multivariable Bidirectional Mendelian Randomization via Bayesian Directed Cyclic Graphical Model with Correlated Errors}
\author[1]{Bitan Sarkar}
\author[1]{Yuchao Jiang}
\author[2]{Tian Ge}
\author[3]{Yang Ni}
\affil[1]{Department of Statistics, Texas A\&M University, College Station, TX, USA}
\affil[2]{Psychiatric and Neurodevelopmental Genetics Unit, Center for Genomic Medicine, Massachusetts General Hospital, Boston, MA, USA}
\affil[3]{Department of Statistics and Data Sciences, University of Texas at Austin, Austin, TX, USA}
\date{}  % or \date{\today}

% --- Hyperref setup ---
\hypersetup{
  colorlinks=true,
  linkcolor=red,
  citecolor=red,
  urlcolor=red
}

% % --- Paths & handy macros ---
% \newcommand{\suppfigpath}{Plots} % change to your figures folder
% \newcommand{\supptablepath}{Tables} % change to your tables folder
\newcommand{\nsizes}{\(n \in \{500, 1000, 10{,}000, 30{,}000\}\)}

\title{Supplementary Material: Multivariable Bidirectional Mendelian Randomization via Bayesian Directed Cyclic Graphical Model with Correlated Errors}
\date{}

\begin{document}
\maketitle

\section{Conditional Likelihood in terms of Summary-Level Data}
\label{sec:likelihood}

We rewrite the conditional Gaussian likelihood entirely in terms of the empirical second–moment matrices
$\mathbf{S_{yy}},\mathbf{S_{yx}},\mathbf{S_{yu}},\mathbf{S_{xx}},\mathbf{S_{xu}},\mathbf{S_{uu}}$ so that inference can be performed from summary-level data (and per-iteration work no longer scales with sample size). Thus, expanding the quadratic form, and converting sums to traces yields:

\begin{align*}
    \begin{split}
        & p\left(\{\mathbf{Y_i}\}_{i=1}^n|\{\mathbf{X_i}\}_{i=1}^n, \{\mathbf{U_i}\}_{i=1}^n, \mathbf{A, B, C, \Sigma^{*}}\right)\\
        = & \prod_{i=1}^n\text{N}(\mathbf{Y_i|(I_p-A)^{-1}BX_i + (I_p-A)^{-1}CU_i,(I_p-A)^{-1} \Sigma^{*} (I_p - A)^{-T}})\\
        = & \prod_{i=1}^n\text{N}(\mathbf{(I_p - A)Y_i - BX_i - CU_i | 0, \Sigma^{*}).|\text{det}(I_p - A)|}\\
        = & \prod_{i = 1}^n (2\pi)^{-p/2}\mathbf{\text{det}(\Sigma^*)^{-1/2}|\text{det}(I_p - A)|} \exp(-\frac{1}{2}\mathbf{[(I_p - A)Y_i - BX_i - CU_i]^{T}}\\
        & \quad\quad\quad\quad\quad\quad \mathbf{{\Sigma^{*}}^{-1}[(I_p - A)Y_i - BX_i - CU_i])}\\
        = & (2\pi)^{-\frac{np}{2}}.\mathbf{\text{det}(\Sigma^*)^{-\frac{n}{2}}.|\text{det}(I_p - A)|^n}.\exp(-\frac{1}{2}\sum_{i = 1}^n \mathbf{[(I_p - A)Y_i - BX_i - CU_i]^{T}}\\
        & \quad\quad\quad\quad\quad\quad \mathbf{{\Sigma^*}^{-1}[(I_p - A)Y_i - BX_i - CU_i])}\\
        = & (2\pi)^{-\frac{np}{2}}.\mathbf{\text{det}(\Sigma^*)^{-\frac{n}{2}}.|\text{det}(I_p - A)|^n}.\exp(-\frac{1}{2}\sum_{i = 1}^n \mathbf{[Y_i^{T}(I_p - A)^{T}{\Sigma^*}^{-1}(I_p - A)Y_i} \\
        & \quad\quad\quad\quad\quad\quad - 2\mathbf{X_i^{T}B^{T}{\Sigma^*}^{-1}(I_p - A)Y_i + X_i^{T}B^{T}{\Sigma^*}^{-1}BX_i - 2U_i^{T}C^{T}{\Sigma^*}^{-1}(I_p - A)Y_i}\\
        & \quad\quad\quad\quad\quad\quad + 2\mathbf{U_i^{T}C^{T}{\Sigma^*}^{-1}BX_i + U_i^{T}C^{T}{\Sigma^*}^{-1}CU_i])}
    \end{split}
\end{align*}
% Break the equation and continue on the next page or after text
\begin{align*}
    \begin{split}
         = & (2\pi)^{-\frac{np}{2}}.\mathbf{\text{det}(\Sigma^*)^{-\frac{n}{2}}.|\text{det}(I_p - A)|^n}.\exp(-\frac{1}{2}\sum_{i = 1}^n \mathbf{[\text{tr}(Y_i^{T}(I_p - A)^{T}{\Sigma^*}^{-1}(I_p - A)Y_i)} \\
        & \quad\quad\quad\quad\quad\quad - 2\mathbf{\text{tr}(X_i^{T}B^{T}\Sigma^{-1}(I_p - A)Y_i) + \text{tr}(X_i^{T}B^{T}\Sigma^{-1}BX_i) -2\text{tr}(U_i^{T}C^{T}{\Sigma^*}^{-1}(I_p - A)Y_i)}\\
        & \quad\quad\quad\quad\quad\quad +2\text{tr}\mathbf{(U_i^{T}C^{T}{\Sigma^*}^{-1}BX_i) + \text{tr}(U_i^{T}C^{T}{\Sigma^*}^{-1}CU_i)]})\\
    % &p\left(\{\mathbf{y_i}\}_{i=1}^n|\{\mathbf{x_i}\}_{i=1}^n, \{\mathbf{u_i}\}_{i=1}^n, \mathbf{A, B, C, \Sigma^{*}}\right)\\
        = & (2\pi)^{-\frac{np}{2}}.\mathbf{\text{det}(\Sigma^*)^{-\frac{n}{2}}.|\text{det}(I_p - A)|^n}.\exp(-\frac{1}{2}\sum_{i = 1}^n \mathbf{[\text{tr}(Y_iY_i^{T}(I_p - A)^{T}{\Sigma^*}^{-1}(I_p - A))} \\
        & \quad\quad\quad\quad\quad\quad - 2\mathbf{\text{tr}(Y_iX_i^{T}B^{T}\Sigma^{-1}(I_p - A)) + \text{tr}(X_iX_i^{T}B^{T}\Sigma^{-1}B) -2\text{tr}(Y_iU_i^{T}C^{T}{\Sigma^*}^{-1}(I_p - A))}\\
        & \quad\quad\quad\quad\quad\quad +2\text{tr}\mathbf{(X_iU_i^{T}C^{T}{\Sigma^*}^{-1}B) + \text{tr}(U_iU_i^{T}C^{T}{\Sigma^*}^{-1}C)]})\\
        = & (2\pi)^{-\frac{np}{2}}.\mathbf{\text{det}(\Sigma^*)^{-\frac{n}{2}}.|\text{det}(I_p - A)|^n}.\exp(-\frac{1}{2} \mathbf{[\text{tr}(\sum_{i = 1}^nY_iY_i^{T}(I_p - A)^{T}{\Sigma^*}^{-1}(I_p - A))} \\
        & \quad\quad\quad\quad\quad\quad - 2\mathbf{\text{tr}(\sum_{i = 1}^n Y_iX_i^{T}B^{T}\Sigma^{-1}(I_p - A)) + \text{tr}(\sum_{i = 1}^n X_iX_i^{T}B^{T}\Sigma^{-1}B)}\\
        & \quad\quad\quad\quad\quad\quad -2\text{tr}\mathbf{(\sum_{i = 1}^n Y_iU_i^{T}C^{T}{\Sigma^*}^{-1}(I_p - A))+2\text{tr}(\sum_{i = 1}^n X_iU_i^{T}C^{T}{\Sigma^*}^{-1}B)}\\
        & \quad\quad\quad\quad\quad\quad + \text{tr}\mathbf{(\sum_{i = 1}^n U_iU_i^{T}C^{T}{\Sigma^*}^{-1}C)]})\\
        = & (2\pi)^{-\frac{np}{2}}.\mathbf{\text{det}(\Sigma^*)^{-\frac{n}{2}}.|\text{det}(I_p - A)|^n}.\exp(-\frac{1}{2} \mathbf{[\text{tr}(nS_{yy}(I_p - A)^{T}{\Sigma^*}^{-1}(I_p - A))} \\
        & \quad\quad\quad\quad\quad\quad - 2\mathbf{\text{tr}(nS_{yx}B^{T}{\Sigma^*}^{-1}(I_p - A)) + \text{tr}(nS_{xx}B^{T}{\Sigma^*}^{-1}B)}\\
        & \quad\quad\quad\quad\quad\quad -2\text{tr}\mathbf{(nS_{yu}C^{T}{\Sigma^*}^{-1}(I_p - A))+2\text{tr}(nS_{xu}C^{T}{\Sigma^*}^{-1}B)}\\
        & \quad\quad\quad\quad\quad\quad + \text{tr}\mathbf{(nS_{uu}C^{T}{\Sigma^*}^{-1}C)]})\\
        = & (2\pi)^{-\frac{np}{2}}.\mathbf{\text{det}(\Sigma^*)^{-\frac{n}{2}}.|\text{det}(I_p - A)|^n}.\exp(-\frac{1}{2} n.\mathbf{[\text{tr}(S_{yy}(I_p - A)^{T}{\Sigma^*}^{-1}(I_p - A))} \\
        & \quad\quad\quad\quad\quad\quad - 2n.\mathbf{\text{tr}(S_{yx}B^{T}{\Sigma^*}^{-1}(I_p - A)) + n.\text{tr}(S_{xx}B^{T}{\Sigma^*}^{-1}B)}\\
        & \quad\quad\quad\quad\quad\quad -2n.\text{tr}\mathbf{(S_{yu}C^{T}{\Sigma^*}^{-1}(I_p - A))+2n.\text{tr}(S_{xu}C^{T}{\Sigma^*}^{-1}B)}\\
        & \quad\quad\quad\quad\quad\quad + n.\text{tr}\mathbf{(S_{uu}C^{T}{\Sigma^*}^{-1}C)]})
    \end{split}
\end{align*}

\section{Detailed Prior Specifications}
\label{subsec:supp_priors}
This section provides the full prior specifications for all model components in \texttt{MR.RGM}, including the causal effect matrix $\mathbf{A}$, the instrument–trait matrix $\mathbf{B}$, the covariate effect matrix $\mathbf{C}$, and the residual covariance matrix $\mathbf{\Sigma^{*}}$.

\paragraph{Priors on the causal effect matrix \(\mathbf{A}\).}
We place a spike-and-slab prior on each off-diagonal entry \( a_{jh} \) of the matrix \(\mathbf{A}\). The presence of a directed edge from $Y_h$ to $Y_j$ is governed by a binary inclusion variable \(\gamma_{jh}\), and the effect size $a_{jh}$ is conditionally modeled as:
\begin{align*}
    a_{jh} &\sim \gamma_{jh} \cdot \text{N}(0, \tau_{jh}) + (1 - \gamma_{jh}) \cdot \text{N}(0, \nu_1 \cdot \tau_{jh}),\\
    \gamma_{jh} &\sim \text{Bernoulli}(\rho_{jh}) \\
    \rho_{jh} &\sim \text{Beta}(a_\rho, b_\rho) \\
    \sqrt{\tau_{jh}} &\sim \mathcal{C}^+(0, 1),
\end{align*}
where $\mathcal{C}^+(0, 1)$ is the standard half-Cauchy distribution. 
Here, we fix \(\nu_1 \ll 1\) to ensure good separation between signals and noises. 
%The half-Cauchy prior on \(\sqrt{\tau_{jh}}\) is motivated by the horseshoe shrinkage framework, encouraging sparsity while allowing for large coefficients. 
Following \cite{makalic2016simple},  half-Cauchy distribution can be reparameterized as:
\[
x \sim \mathcal{C}^+(0, 1) \implies x^2 \mid a \sim \text{IG}(1/2, 1/a), \quad a \sim \text{IG}(1/2, 1),
\]
where \(\text{IG}(\cdot, \cdot)\) denotes the inverse-gamma distribution. This allows a closed-form Gibbs update. 

\paragraph{Priors on the instrument effect matrix \(\mathbf{B}\).}
When there may be horizontal pleiotropy (the violation of the exclusion restriction assumption) or weak instruments (the violation of the relevance assumption), we do not impose fixed structural zeros in  $\mathbf{B}$ but instead adopt a spike-and-slab prior for each entry of \(\mathbf{B}\):
\begin{align*}
    b_{jh} &\sim \phi_{jh} \cdot \text{N}(0, \eta_{jh}) + (1 - \phi_{jh}) \cdot \text{N}(0, \nu_2 \cdot \eta_{jh}), \\
    \phi_{jh} &\sim \text{Bernoulli}(\psi_{jh}), \\
    \psi_{jh} &\sim \text{Beta}(a_\psi, b_\psi), \\
    \sqrt{\eta_{jh}} &\sim \mathcal{C}^+(0, 1),
\end{align*}
where $\nu_2\ll 1$ and $\phi_{jh}$ indicates whether $X_h$ is a (significant) instrument for $Y_j$. This prior formulation encourages sparsity in \(\mathbf{B}\), facilitating automatic selection of valid and relevant instruments. Under the InSIDE assumption \cite{bowden2015mendelian,yuan2020testing} that the instrument effects are independent of each other, we obtain unbiased causal effect estimation. We call \texttt{MR.RGM} with selection on instruments \texttt{MR.RGM+}. 
Otherwise, simple normal priors are placed on the non-zero entries of $\mathbf{B}$. 
% Otherwise, pre-specified structural zeros are imposed on $\mathbf{B}$, and the same spike-and-slab prior is placed on the remaining entries.
\paragraph{Prior on the covariate effect matrix \(\mathbf{C}\).}
We assume a conjugate matrix-normal prior on \(\mathbf{C} \in \mathbb{R}^{p \times l}\):
\[
\mathbf{C} \sim \text{MN}_{p \times l}(\mathbf{0},\, \mathbf{\Sigma}^*,\, \tau \mathbf{I}_l).
\]
% This formulation induces a dependence between \(\mathbf{C}\) and the residual structure through \(\mathbf{\Sigma}^*\), enabling a unified modeling of the variance structure. The rows of \(\mathbf{C}\) are correlated according to \(\mathbf{\Sigma}^*\), while the columns are a priori independent with scale parameter \(\tau\).

\paragraph{Prior on the error covariance matrix \(\mathbf{\Sigma^*}\).}

The error covariance matrix \(\mathbf{\Sigma}^* = \mathbf{D}\mathbf{D}^T + \mathbf{\Sigma}\) combines unmeasured confounding (via \(\mathbf{D}\)) and measurement noise (via \(\mathbf{\Sigma}\)). Since we do not know \textit{a priori} the number $t$ of unmeasured confounders, we directly model \(\mathbf{\Sigma}^*\) instead of modeling $\mathbf{D}$ and $\mathbf{\Sigma}$. We introduce a binary indicator matrix \(\mathbf{Z} = (z_{jh}) \in \{0,1\}^{p \times p}\) that encodes whether the off-diagonal entry \(\sigma^*_{jh}\) is nonzero. The priors are specified as follows:
\begin{align*}
   & \sigma^*_{jh}  \sim z_{jh} \cdot \text{N}(0, \omega_1^2) + (1 - z_{jh}) \cdot \text{N}(0, \omega_2^2), \quad j < h, \\
   & z_{jh} \sim \text{Bernoulli}(\pi), \\
   & \sigma^*_{jj}\sim \text{Exp}\left(\frac{\lambda}{2}\right),
\end{align*}
% This hierarchical spike-and-slab prior allows flexible inference of partial correlations among the trait variables, accounting for latent confounding. The indicator matrix \(\mathbf{Z}\) is updated during MCMC to perform joint inference and structure learning over the covariance graph.
subject to the positive-definiteness of the resulting $\mathbf{\Sigma^*}$.
The hyperparameters \(\omega_1, \omega_2, \pi\) and \(\lambda\) control the sparsity and scale of the inferred error covariance. Following \cite{wang2015}, we recommend setting \(\omega_2 \geq 0.01\) and \(\omega_1/\omega_2 \leq 1000\) to ensure numerical stability and encourage separation between signals and noises. The parameter \(\pi\) lies between $0$ and $1$, with smaller values favoring sparser structures. For the exponential prior, \(\lambda\) may be set to moderately large values such as $5$ or $10$.

\section{Detailed Posterior Inference Procedure}

Our MCMC consists of the following $11$ updates at each iteration.
\begin{enumerate}
    \item Update $\psi_{jh}$ by a Gibbs transition probability. Draw $\psi_{jh} \sim \text{Beta}(\phi_{jh} + a_{\psi}, 1 - \phi_{jh} + b_{\psi})$.
    
    \item Update $\eta_{jh}$ by a Gibbs transition probability. Draw $\epsilon \sim \text{IG}(1, 1 + 1 / \eta_{jh})$ and then draw $\eta_{jh} \sim \text{IG}(1, b_{jh}^2 / 2 + 1 / \epsilon)$ (if $\phi_{jh} = 1$) or draw  $\eta_{jh} \sim \text{IG}(1, b_{jh}^2 / (2 \times \nu_2) + 1 / \epsilon)$ (if $\phi_{jh} = 0$).
    
    \item Update $\phi_{jh}$ by a Gibbs transition probability. Draw $\phi_{jh} \sim Ber(p_\phi)$ where,
    \begin{align*}
        p_\phi = \frac{\exp{(- b_{jh}^2 / (2 \times \eta_{jh}))} \times \psi_{jh}}{\exp{(- b_{jh}^2 / (2 \times \eta_{jh}))} \times \psi_{jh} + \exp{(- b_{jh}^2 / (2 \times \nu_2 \times \eta_{jh}))} \times (1 - \psi_{jh}) / \sqrt{\nu_2}}.
    \end{align*}
    
    \item Update $b_{jh}$ by a random-walk  Metropolis-Hastings (M-H) transition probability. Propose $\tilde{b}_{jh} \sim N(b_{jh}, \xi_b)$ where $\xi_b$ is the proposal variance and create $\mathbf{\tilde{B}}$ from $\mathbf{B}$ by substituting $b_{jh}$ by $\tilde{b}_{jh}$. Accept $\tilde{b}_{jh}$ with probability min$(\alpha, 1)$ where,
    \begin{align*}
        \alpha = \frac{p\left(\{\mathbf{y_i}\}_{i=1}^n|\{\mathbf{x_i}\}_{i=1}^n, \{\mathbf{u_i}\}_{i=1}^n, \mathbf{A, \tilde{B}, C, \Sigma^{*}}\right)p(\tilde{b}_{jh}|\phi_{jh}, \eta_{jh})}{p\left(\{\mathbf{y_i}\}_{i=1}^n|\{\mathbf{x_i}\}_{i=1}^n, \{\mathbf{u_i}\}_{i=1}^n, \mathbf{A, B, C, \Sigma^{*}}\right)p(b_{jh}|\phi_{jh}, \eta_{jh})}.
    \end{align*}
    
    \item Update $\rho_{jh}$ by a Gibbs transition probability. Draw $\rho_{jh} \sim \text{Beta}(\gamma_{jh} + a_{\rho}, 1 - \gamma_{jh} + b_{\rho})$.
    
    \item Update $\tau_{jh}$ by a Gibbs transition probability. Draw $\epsilon \sim \text{IG}(1, 1 + 1 / \tau_{jh})$ and then draw $\tau_{jh} \sim \text{IG}(1, a_{jh}^2 / 2 + 1 / \epsilon)$ (if $\gamma_{jh} = 1$) or draw  $\tau_{jh} \sim \text{IG}(1, a_{jh}^2 / (2 \times \nu_1) + 1 / \epsilon)$ (if $\gamma_{jh} = 0$).
    
    \item Update $\gamma_{jh}$ by a Gibbs transition probability. Draw $\gamma_{jh} \sim Ber(p_\gamma)$ where
    \begin{align*}
        p_\gamma = \frac{\exp{(- a_{jh}^2 / (2 \times \tau_{jh}))} \times \rho_{jh}}{\exp{(- a_{jh}^2 / (2 \times \tau_{jh}))} \times \rho_{jh} + \exp{(- a_{jh}^2 / (2 \times \nu_1 \times \tau_{jh}))} \times (1 - \rho_{jh}) / \sqrt{\nu_1}}.
    \end{align*}
    
    \item Update $a_{jh}$ by a random walk  Metropolis-Hastings (M-H) transition probability. Propose $\tilde{a}_{jh} \sim N(a_{jh}, \xi_a)$ where $\xi_a$ is the proposal variance and create $\mathbf{\tilde{A}}$ from $\mathbf{A}$ by substituting $a_{jh}$ by $\tilde{a}_{jh}$. Accept $\tilde{a}_{jh}$ with probability min$(\alpha, 1)$ where,
    \begin{align*}
        \alpha = \frac{p\left(\{\mathbf{y_i}\}_{i=1}^n|\{\mathbf{x_i}\}_{i=1}^n, \{\mathbf{u_i}\}_{i=1}^n, \mathbf{\tilde{A}, B, C, \Sigma^{*}}\right)p(\tilde{a}_{jh}|\gamma_{jh}, \tau_{jh}, \nu_1)}{p\left(\{\mathbf{y_i}\}_{i=1}^n|\{\mathbf{x_i}\}_{i=1}^n, \{\mathbf{u_i}\}_{i=1}^n, \mathbf{A, B, C, \Sigma^{*}}\right)p(a_{jh}|\gamma_{jh}, \tau_{jh}, \nu_1)}.
    \end{align*}

    \item Update $\mathbf{C}$ by a Gibbs transition probability:
    \[
    \mathbf{C} \sim \text{MN}_{p \times l} \left( \left[n (\mathbf{I}_p - \mathbf{A}) \mathbf{S}_{yu} - n\mathbf{B}\mathbf{S}_{xu} \right] (n \mathbf{S}_{uu} + \tau^{-1} \mathbf{I}_l)^{-1}, \; \mathbf{\Sigma}^*, \; (n \mathbf{S}_{uu} + \tau^{-1} \mathbf{I}_l)^{-1} \right)
    \].

    \item 
    %\textbf{Update } $\mathbf{Z}$: For each off-diagonal element $\sigma^*_{jh}$, 
    Update $z_{jh}$ for $j<h$ by a Gibbs transition probability:
    \[
    z_{jh} \sim \text{Bernoulli}(p_z), \quad \text{where } 
    p_z = \frac{\frac{1}{\omega_1}\exp\left(- \frac{(\sigma^*_{jh})^2}{2 \omega_1^2} \right) \cdot \pi}{\frac{1}{\omega_1}\exp\left(- \frac{(\sigma^*_{jh})^2}{2 \omega_1^2} \right) \cdot \pi + \frac{1}{\omega_2}\exp\left(- \frac{(\sigma^*_{jh})^2}{2 \omega_2^2} \right) \cdot (1 - \pi)}.
    \]

    \item Update $\mathbf{\Sigma}^*$ by a blocked Gibbs step following \cite{wang2015}. We define $\mathbf{S}$ as:
    \begin{align*}
        \mathbf{S} = & n \{(\mathbf{I}_p - \mathbf{A})\mathbf{S_{yy}}(\mathbf{I}_p - \mathbf{A})^{\text{T}} - (\mathbf{I}_p - \mathbf{A})\mathbf{S_{yx}}\mathbf{B}^{\text{T}} -  \mathbf{B}\mathbf{S_{yx}}^{\text{T}}(\mathbf{I}_p - \mathbf{A})^{\text{T}} + \mathbf{B}\mathbf{S_{xx}}\mathbf{B}^{\text{T}} + \mathbf{C}\mathbf{S_{uu}}\mathbf{C}^{\text{T}}\\
        & - (\mathbf{I}_p - \mathbf{A})\mathbf{S_{yu}}\mathbf{C}^{\text{T}} - \mathbf{C}\mathbf{S_{yu}}^{\text{T}}(\mathbf{I}_p - \mathbf{A})^{\text{T}} + \mathbf{B}\mathbf{S_{xu}}\mathbf{C}^{\text{T}} + \mathbf{C}\mathbf{S_{xu}}^{\text{T}}\mathbf{B}^{\text{T}}\} + \mathbf{C} \mathbf{C}^{\text{T}}/\tau.
    \end{align*}
     For each column \(j = 1, \dots, p\), partition \(\mathbf{\Sigma}^*, \mathbf{S}\), and \(\mathbf{Z}\) as:
    \[
    \mathbf{\Sigma}^* = \begin{bmatrix}
    \mathbf{\Sigma}_{11} & \sigma_{12} \\
    \sigma_{12}^\top & \sigma_{22}
    \end{bmatrix}, \quad 
    \mathbf{S} = \begin{bmatrix}
    \mathbf{S}_{11} & s_{12} \\
    s_{12}^\top & s_{22}
    \end{bmatrix},  \quad 
    \mathbf{Z} = \begin{bmatrix}
    \mathbf{Z}_{11} & z_{12} \\
    z_{12}^\top & z_{22}
    \end{bmatrix}.
    \]
    Let \( u = \sigma_{12} \), and define \( v = \sigma_{22} - \sigma_{12}^\top \mathbf{\Sigma}_{11}^{-1} \sigma_{12} \). Then the full conditionals are:
    \begin{align*}
        u \mid \cdot &\sim \text{N}((\mathbf{\Omega} + \text{diag}(v_{12}^{-1}))^{-1} w, \; (\mathbf{\Omega} + \text{diag}(v_{12}^{-1}))^{-1}), \\
        v \mid \cdot &\sim \text{GIG}\left(1 - \frac{n}{2}, \lambda, u^\top \mathbf{\Sigma}_{11}^{-1} \mathbf{S}_{11} \mathbf{\Sigma}_{11}^{-1} u - 2 s_{12}^\top \mathbf{\Sigma}_{11}^{-1} u + s_{22} \right),
    \end{align*}
    where \( w = \mathbf{\Sigma}_{11}^{-1} s_{12} v^{-1} \) and \( \mathbf{\Omega} = \mathbf{\Sigma}_{11}^{-1} \mathbf{S}_{11} \mathbf{\Sigma}_{11}^{-1} v^{-1} + \lambda \mathbf{\Sigma}_{11}^{-1} \). %Hence, we will update $\mathbf{\Sigma}^*$ column by column and we will have to do it $p$ many times at each iteration, where $\mathbf{Z}$ and $\mathbf{S}$ will be fixed for that iteration. 
\end{enumerate}

After MCMC, we summarize model parameters as follows:
\paragraph{Selection and Estimation of \(\mathbf{A}\) (Causal Effects):}
% We monitor the posterior samples of the binary inclusion indicator matrix \(\mathbf{\Gamma} = (\gamma_{ij})\), where \(\gamma_{ij}\) encodes the presence or absence of a causal edge from trait \(j\) to trait \(i\). 
We compute the posterior mean of each \(\gamma_{jh}\) for $j\neq h$, which is an estimate of the marginal inclusion probability for a causal edge from trait \(h\) to trait \(j\). 
To obtain a sparse causal graph, we can apply a threshold (e.g., $0.5$) to marginal inclusion probabilities, which yields a binary adjacency matrix. The causal effect matrix $\mathbf{A}$ is computed as the element-wise (Hadamard) product of the posterior mean of \(\mathbf{A}\) and the binary adjacency matrix, preserving effect sizes only for edges with sufficient posterior support.

\paragraph{Selection and Estimation of \(\mathbf{B}\) (Instrumental Effects):}
Similarly, 
%for the instrument-trait matrix \(\mathbf{B}\), we track the inclusion indicator matrix \(\mathbf{\Phi} = (\phi_{il})\), where \(\phi_{il}\) indicates whether instrument \(l\) affects trait \(i\). The 
we compute the posterior mean of each \(\phi_{il}\), which is the inclusion probability for each instrument-trait pair. We threshold it and multiply it element-wise with the posterior mean of \(\mathbf{B}\) to retain only those instrumental effects that are well-supported by the data. 
%This filtered matrix provides a clear summary of the relevant genetic instruments and whether there is horizontal pleiotropy.

\paragraph{Selection and Estimation of \(\mathbf{\Sigma^*}\) (Residual Covariance and Confounding Structure):}
% The matrix \(\mathbf{\Sigma^*}\) is the residual variance-covariance after accounting for the effects of instruments and covariates. To assess which off-diagonal covariance terms are statistically supported, 
We compute the posterior mean of each \(z_{jh} = 1\) for $j\neq h$, which is the inclusion probability for confounding between traits \(j\) and \(h\). We threshold it and multiply it element-wise with the posterior mean of \(\mathbf{\Sigma^*}\). This results in a sparse estimate of the residual covariance matrix, identifying significant confounding effects that are supported by the data. 

\section{Identifiability of \texttt{MR.RGM+} Under Instrument Diversity and Sparsity}
\label{suppsec:identifiability_proof}

Consider the SEM:
\begin{equation*}
\mathbf{Y} = \mathbf{A}\mathbf{Y} + \mathbf{B}\mathbf{X} + \mathbf{E}^*, 
\end{equation*}
where $\mathbf{Y} \in \mathbb{R}^p$, $\mathbf{X} \in \mathbb{R}^k$, $\mathbf{A} \in \mathbb{R}^{p \times p}$ with $\diag(\mathbf{A}) = \mathbf{0}$, $\mathbf{B} \in \mathbb{R}^{p \times k}$, and $\mathbf{E}^* \sim N_p(\mathbf{0}, \boldsymbol{\Sigma}^*)$.
We assume $\mathbf{X} \sim (\mathbf{0}, \boldsymbol{\Sigma}_{XX})$ with $\boldsymbol{\Sigma}_{XX} \succ 0$, $\mathbf{X} \perp \mathbf{E}^*$, and $(\mathbf{I}_p - \mathbf{A})$ is invertible.
The reduced form is:
\begin{equation*}
\mathbf{Y} = \boldsymbol{\Pi}\mathbf{X} + \boldsymbol{\eta}, \quad \boldsymbol{\eta} \sim N_p(\mathbf{0}, \boldsymbol{\Omega}), 
\end{equation*}
where:
\begin{align}
\boldsymbol{\Pi} &= (\mathbf{I}_p - \mathbf{A})^{-1}\mathbf{B} \nonumber\\
\boldsymbol{\Omega} &= (\mathbf{I}_p - \mathbf{A})^{-1}\boldsymbol{\Sigma}^*(\mathbf{I}_p - \mathbf{A})^{-\top} \label{eq:Omega}
\end{align}

From observations, we can identify:
\begin{align*}
\boldsymbol{\Pi} &= \text{Cov}(\mathbf{Y}, \mathbf{X})\boldsymbol{\Sigma}_{XX}^{-1} \\
\boldsymbol{\Omega} &= \text{Var}(\mathbf{Y}) - \boldsymbol{\Pi}\boldsymbol{\Sigma}_{XX}\boldsymbol{\Pi}^\top
\end{align*}

Vectorize $\mathbf{B} = (\mathbf{I}_p - \mathbf{A})\boldsymbol{\Pi}$ by stacking its rows:
\begin{equation*}
\vect(\mathbf{B}) = \vect(\boldsymbol{\Pi}) - \mathbf{M}\mathbf{a} 
\end{equation*}
where $\mathbf{a} = (a_{12}, a_{13}, \ldots, a_{1p}, a_{21}, a_{23}, \ldots, a_{p,p-1})^\top \in \mathbb{R}^{p(p-1)}$ is the vector of off-diagonal elements of $\mathbf{A}$, and $\mathbf{M} \in \mathbb{R}^{pk \times p(p-1)}$ is a block diagonal matrix:
\begin{equation*}
\mathbf{M} = \diag(\boldsymbol{\Phi}_1, \boldsymbol{\Phi}_2, \ldots, \boldsymbol{\Phi}_p), 
\end{equation*}
where each block $\boldsymbol{\Phi}_j \in \mathbb{R}^{k \times (p-1)}$ corresponds to trait $j$ and is given by:
\begin{equation*}
\boldsymbol{\Phi}_j = \boldsymbol{\Pi}_{-j}^\top.
\end{equation*}
Here $\boldsymbol{\Pi}_{-j} \in \mathbb{R}^{(p-1) \times k}$ denotes $\boldsymbol{\Pi}$ with row $j$ removed.

The block diagonal structure of $\mathbf{M}$ implies that the identification problem can be decomposed into $p$ independent subproblems, one for each trait $j$. The causal effects $\{a_{ji}\}_{i \neq j}$ can be determined independently from the zero constraints on row $j$ of $\mathbf{B}$.

\begin{lemma}[Rank of constraint submatrix]
\label{lem:rank_refined}
Suppose Instrument Diversity holds. For any support $S:=\supp(\mathbf{B}) \subseteq \{1, \ldots, p\} \times \{1, \ldots, k\}$ with per-trait supports $S_j=\supp(\mathbf{B}_{j,:}) = \{h : (j,h) \in S\}$ satisfying:
\begin{equation*}
|S_j^c| \geq p - 1 \quad \text{for all } j \in \{1, \ldots, p\},
\end{equation*}
we have:
\begin{equation*}
\rank([\mathbf{M}]_{S^c, :}) = p(p-1)
\end{equation*}
where $[\mathbf{M}]_{S^c, :}$ is defined as
\begin{equation*}
[\mathbf{M}]_{S^c, :} = \diag\left([\boldsymbol{\Phi}_1]_{S_1^c, :}, [\boldsymbol{\Phi}_2]_{S_2^c, :}, \ldots, [\boldsymbol{\Phi}_p]_{S_p^c, :}\right)
\end{equation*}
\end{lemma}

\begin{proof}
For a block diagonal matrix, the rank is the sum of the ranks of the diagonal blocks:
\begin{equation*}
\rank([\mathbf{M}]_{S^c, :}) = \sum_{j=1}^{p} \rank([\boldsymbol{\Phi}_j]_{S_j^c, :})
\end{equation*}

We now show that $\rank([\boldsymbol{\Phi}_j]_{S_j^c, :}) = p - 1$ for each $j$.

Recall that $\boldsymbol{\Phi}_j = \boldsymbol{\Pi}_{-j}^\top \in \mathbb{R}^{k \times (p-1)}$. Thus:
\[
[\boldsymbol{\Phi}_j]_{S_j^c, :} = [\boldsymbol{\Pi}_{-j}^\top]_{S_j^c, :} = (\boldsymbol{\Pi}_{-j, S_j^c})^\top
\]
where $\boldsymbol{\Pi}_{-j, S_j^c} \in \mathbb{R}^{(p-1) \times |S_j^c|}$ is $\boldsymbol{\Pi}_{-j}$ restricted to columns in $S_j^c$.

Since $|S_j^c| \geq p - 1$ by assumption, the matrix $\boldsymbol{\Pi}_{-j, S_j^c}$ has at least $p-1$ columns. By Instrument Diversity, any $(p-1)$ columns of $\boldsymbol{\Pi}_{-j}$ are linearly independent, so:
\[
\rank(\boldsymbol{\Pi}_{-j, S_j^c}) = p - 1
\]

Therefore $\rank([\boldsymbol{\Phi}_j]_{S_j^c, :}) = \rank((\boldsymbol{\Pi}_{-j, S_j^c})^\top) = p - 1$.

Summing over all traits:
\[
\rank([\mathbf{M}]_{S^c, :}) = \sum_{j=1}^{p} (p-1) = p(p-1)
\]
\end{proof}

\subsection*{Proof of the Identifiability Theorem}

For each trait $j$, define:
\begin{itemize}
    \item $\mathbf{a}_{j,-j} \in \mathbb{R}^{p-1}$: the off-diagonal entries $(a_{j1}, \ldots, a_{j,j-1}, a_{j,j+1}, \ldots, a_{jp})^\top$
    \item $\mathbf{b}_j\in \mathbb{R}^k$: row $j$ of $\mathbf{B}$
     \item $\boldsymbol{\pi}_j\in \mathbb{R}^k$: row $j$ of $\mathbf{\Pi}$
    \item $S_j \subseteq \{1, \ldots, k\}$: the support of row $j$ of $\mathbf{B}$, i.e., $S_j:=\supp(\mathbf{b}_j)$
    \item $S_j^c = \{1, \ldots, k\} \setminus S_j$: instruments where $b_{jh} = 0$
    \item $s_j:=\|\mathbf{b}_j\|_{0}=|S_j|$: the number of nonzero entries in $\mathbf{b}_j$
\end{itemize}

The constraint for trait $j$ is:
\begin{equation*}
\mathbf{b}_j = \boldsymbol{\pi}_j - \boldsymbol{\Phi}_j \mathbf{a}_{j,-j} 
\end{equation*}

The zero constraints (for $h \in S_j^c$) give:
\begin{equation*}
[\boldsymbol{\pi}_j]_{S_j^c} = [\boldsymbol{\Phi}_j]_{S_j^c, :} \mathbf{a}_{j,-j} 
\end{equation*}

This is a system of $|S_j^c| = k - s_j$ linear equations in $p - 1$ unknowns. For a fixed support $S_j$ with $|S_j| = s_j$, this system  has $k - s_j$ equations in $p - 1$ unknowns. For it to have at most one solution, we need it to be overdetermined or just-determined, i.e., $k - s_j \geq p - 1$ and hence $s_j \leq k - p + 1$.
Under Instrument Diversity and $|S_j^c| = k - s_j \geq p - 1$, Lemma \ref{lem:rank_refined} guarantees full column rank $\rank([\boldsymbol{\Phi}_j]_{S_j^c, :}) = p - 1$.
Thus, for each trait $j$ with $s_j \leq k - p + 1$, there exists at most one $\mathbf{a}_{j,-j}$ satisfying the constraints for support $S_j$.

Since a priori we do not know the support $S_j$, we need to prove the uniqueness of the solution across all possible supports. Suppose for contradiction that two solutions exist, $(\mathbf{A}, \mathbf{B})$ and $(\mathbf{A}', \mathbf{B}')$ with $\mathbf{A}  \neq \mathbf{A}'$, $|S_j| \leq s_j$, and $|S_j'| \leq s_j$ for all $j$. 
Since $\mathbf{A}  \neq \mathbf{A}'$, there exists at least one trait $j^*$ such that $\mathbf{a}_{j^*,-j^*}  \neq \mathbf{a}_{j^*,-j^*}'$.
For this trait, both $\mathbf{a}_{j^*,-j^*}$ and $\mathbf{a}_{j^*,-j^*}'$ must satisfy zero constraints on their respective supports.

\emph{Zero constraints for $(\mathbf{A}, \mathbf{B})$:} For every $h \in (S_{j^*} )^c$, we have $b_{j^*h}  = 0$, which means:
\begin{equation*}
\pi_{j^*h} = \sum_{i \neq j^*} a_{j^*i}  \pi_{ih} \quad \text{for all } h \in (S_{j^*} )^c
\end{equation*}

\emph{Zero constraints for $(\mathbf{A}', \mathbf{B}')$:} For every $h \in (S_{j^*}')^c$, we have $b_{j^*h}' = 0$, which means:
\begin{equation*}
\pi_{j^*h} = \sum_{i \neq j^*} a_{j^*i}' \pi_{ih} \quad \text{for all } h \in (S_{j^*}')^c
\end{equation*}

\emph{Constraints on the intersection:} Define:
\[
(S_{j^*} )^c \cap (S_{j^*}')^c = (S_{j^*}  \cup S_{j^*}')^c
\]

This is the set of instruments where \emph{both} $\mathbf{B} $ and $\mathbf{B}'$ have zeros in row $j^*$. On this intersection, \emph{both} $\mathbf{a}_{j^*,-j^*} $ and $\mathbf{a}_{j^*,-j^*}'$ must satisfy the \emph{same} linear constraints:
\begin{equation}
[\boldsymbol{\pi}_{j^*}]_{(S_{j^*}  \cup S_{j^*}')^c} = [\boldsymbol{\Phi}_{j^*}]_{(S_{j^*}  \cup S_{j^*}')^c, :} \mathbf{a}_{j^*,-j^*} \label{eq:shared_constraints}
\end{equation}

By inclusion-exclusion:
\[
|S_{j^*}  \cup S_{j^*}'| \leq |S_{j^*} | + |S_{j^*}'| \leq s_{j^*} + s_{j^*} = 2s_{j^*}
\]

Therefore:
\[
|(S_{j^*}  \cup S_{j^*}')^c| = k - |S_{j^*}  \cup S_{j^*}'| \geq k - 2s_{j^*}
\]

 For the system \eqref{eq:shared_constraints} to have at most one solution, we need it to be overdetermined or just-determined:
\[
|(S_{j^*}  \cup S_{j^*}')^c| \geq p - 1
\]
\[
k - 2s_{j^*} \geq p - 1
\]
\[
s_{j^*} \leq \frac{k - p + 1}{2}
\]

Under Instrument Diversity, if $|(S_{j^*}  \cup S_{j^*}')^c| \geq p - 1$, then Lemma \ref{lem:rank_refined} guarantees:
\[
\rank([\boldsymbol{\Phi}_{j^*}]_{(S_{j^*}  \cup S_{j^*}')^c, :}) = p - 1
\]
Therefore, the system has at most one solution. Since both $\mathbf{a}_{j^*,-j^*} $ and $\mathbf{a}_{j^*,-j^*}'$ satisfy the system, $\mathbf{a}_{j^*,-j^*}  = \mathbf{a}_{j^*,-j^*}'$, which contradicts our assumption that $\mathbf{a}_{j^*,-j^*}  \neq \mathbf{a}_{j^*,-j^*}'$.
Since the argument must hold for any trait $j^*$ where $\mathbf{A} $ and $\mathbf{A}'$ differ, we require:
\[
s_j \leq \frac{k - p + 1}{2} \quad \text{for all } j \in \{1, \ldots, p\}
\]
or equivalently,
\[
\max_{j} s_j \leq \frac{k - p + 1}{2},
\]
which is our sparsity assumption.

Once $\mathbf{A}$ is identified, $\boldsymbol{\Sigma}^*$ is uniquely determined:
\[
\boldsymbol{\Sigma}^* = (\mathbf{I}_p - \mathbf{A})\boldsymbol{\Omega}(\mathbf{I}_p - \mathbf{A})^\top
\]
where $\boldsymbol{\Omega}$ is identified from the data via \eqref{eq:Omega}.

This completes the proof.

\begin{remark}[Tightness of the bound]
The per-trait bound is tight in the following sense: if $s_j > (k - p + 1)/2$ for some trait $j$, one can construct examples where two distinct supports yield feasible solutions with different $\mathbf{A}$ matrices.

For example, consider $p = 2$ traits and $k = 3$ instruments with:
\[
\boldsymbol{\Pi} = \begin{pmatrix} 1 & 2 & 3 \\ 1 & 1 & 1 \end{pmatrix}
\]
This satisfies Instrument Diversity (all entries non-zero). The per-trait bound requires $s_j \leq (k-p+1)/2 = 1$.

We construct two distinct solutions, both with $s_1 = 2 > 1$. Recall that $b_{1h} = \pi_{1h} - a_{12}\pi_{2h}$.

\textit{Solution 1:} Support $S_1 = \{1, 2\}$ with zero constraint $b_{13} = 0$:
\[
\pi_{13} = a_{12} \cdot \pi_{23} \implies a_{12} = 3
\]
Verification: $b_{11} = 1 - 3\times 1 = -2$, $b_{12} = 2 - 3\times 1 = -1$, $b_{13} = 0$. Thus $s_1 = 2$. 

\textit{Solution 2:} Support $S_1' = \{2, 3\}$ with zero constraint $b_{11}' = 0$:
\[
\pi_{11} = a_{12}' \cdot \pi_{21} \implies a_{12}' = 1
\]
Verification: $b_{11}' = 0$, $b_{12}' = 2 - 1\times1 = 1$, $b_{13}' = 3 - 1\times1 = 2$. Thus $s_1' = 2$. 

Both solutions satisfy the same reduced form and sparsity level, but yield different causal effects ($a_{12} = 3 \neq 1 = a_{12}'$). The key observation is that $(S_1 \cup S_1')^c = \emptyset$---there are no shared zero constraints to enforce uniqueness. This demonstrates that the bound $s_j \leq (k-p+1)/2$ is tight.
\end{remark}

\subsection*{Examples of Instrument Diversity}

\begin{example}[Failure of Instrument Diversity: Block diagonal $\boldsymbol{\Pi}$]
\label{ex:block_diagonal}
Consider $p = 2$ traits, $k = 4$ instruments, with block diagonal structure:
\[
\boldsymbol{\Pi} = \begin{pmatrix} \pi_{11} & \pi_{12} & 0 & 0 \\ 0 & 0 & \pi_{23} & \pi_{24} \end{pmatrix}
\]

Instrument Diversity fails because:
\begin{itemize}
    \item For $j = 1$: $\boldsymbol{\Pi}_{-1} = (0, 0, \pi_{23}, \pi_{24})$. Any $1 \times 1$ submatrix from columns 1 or 2 is zero.
    \item For $j = 2$: $\boldsymbol{\Pi}_{-2} = (\pi_{11}, \pi_{12}, 0, 0)$. Any $1 \times 1$ submatrix from columns 3 or 4 is zero.
\end{itemize}
Instruments 1--2 affect only trait 1; instruments 3--4 affect only trait 2. There is no ``cross-trait'' variation to identify the causal effects $a_{12}$ and $a_{21}$.
\end{example}

\begin{example}[Failure of Instrument Diversity: Insufficient instruments for one trait]
\label{ex:insufficient}
Consider $p = 2$ traits, $k = 4$ instruments:
\[
\boldsymbol{\Pi} = \begin{pmatrix} \pi_{11} & 0 & 0 & 0 \\ 0 & \pi_{22} & \pi_{23} & \pi_{24} \end{pmatrix}
\]

Instrument Diversity fails because:
\begin{itemize}
    \item For $j = 1$: $\boldsymbol{\Pi}_{-1} = (0, \pi_{22}, \pi_{23}, \pi_{24})$. Column 1 is zero, so any $1 \times 1$ submatrix using column 1 fails.
    \item For $j = 2$: $\boldsymbol{\Pi}_{-2} = (\pi_{11}, 0, 0, 0)$. Columns 2, 3, 4 are zero.
\end{itemize}
Trait 1 has only one instrument (column 1), and this instrument does not affect trait 2 in the reduced form. There is no information to identify $a_{12}$ (the causal effect of trait 2 on trait 1).
\end{example}

\begin{example}[Instrument Diversity satisfied]
\label{ex:satisfied}
Consider $p = 2$ traits, $k = 4$ instruments with dense $\boldsymbol{\Pi}$:
\[
\boldsymbol{\Pi} = \begin{pmatrix} 1 & 2 & 3 & 4 \\ 5 & 6 & 7 & 8 \end{pmatrix}
\]

Instrument Diversity holds because:
\begin{itemize}
    \item For $j = 1$: $\boldsymbol{\Pi}_{-1} = (5, 6, 7, 8)$. All $1 \times 1$ submatrices are non-zero.
    \item For $j = 2$: $\boldsymbol{\Pi}_{-2} = (1, 2, 3, 4)$. All $1 \times 1$ submatrices are non-zero.
\end{itemize}
With the per-trait bound $s_j \leq (4 - 2 + 1)/2 = 1.5$, each trait can have at most 1 direct instrument effect. 
\end{example}

\section{Additional Simulation Results}
We provide all figures for network size \(p{=}5\) and all tables for \(p\in\{5,10\}\) under three settings:
(1) scale-free network with feedback loops and unmeasured confounding;
(2) small-world network with feedback loops and unmeasured confounding; and
(3) small-world network with feedback loops, unmeasured confounding, and horizontal pleiotropy. The only exceptions are the graph recovery performance table and the causal effect estimation table for the scale-free setting with \(p{=}10\), which are included in the main manuscript.
Unless noted otherwise, all figures report results across \nsizes.
For each combination of scenario, sample size, and network size, every method is evaluated over $20$ independent replicates; figures and tables summarize these replicates.

\subsection{Case \texorpdfstring{$1$}{1}: Scale-free network with feedback loops and unmeasured confounding}

\noindent\textit{Overview.} Figure (\ref{fig:sf_auc_p5}) reports graph-recovery AUC (boxplots) by method across sample sizes for network size $p=5$. Tables (\ref{tab:feedback_graph_structure_scalefree_90_p=5}) summarize graph-recovery metrics (AUC, TPR, FDR, MCC; mean $\pm$ sd) for $p=5$. Figure (\ref{fig:sf_mad_p5}) shows causal-effect estimation error (MeanAbsDev; boxplots) by method across sample sizes for $p=5$, while Tables (\ref{tab:feedback_causal_effect_scalefree_90_p=5}) report effect-estimation error metrics (MaxAbsDev, MeanAbsDev, MeanSqDev; mean $\pm$ sd) for $p=5$. Finally, Figure (\ref{fig:sf_conf_p5}) presents confounding-structure recovery AUC (boxplots) for $p=5$ using \texttt{MR.RGM}, and Table (\ref{tab:feedback_conf_auc_scalefree_A}) compiles confounding-structure recovery metrics (AUC, TPR, FDR, MCC; mean $\pm$ sd) for $p\in\{5,10\}$ using \texttt{MR.RGM} across all sample sizes.

\begin{figure}[htb]
    \centering
    \includegraphics[width=.7\textwidth]{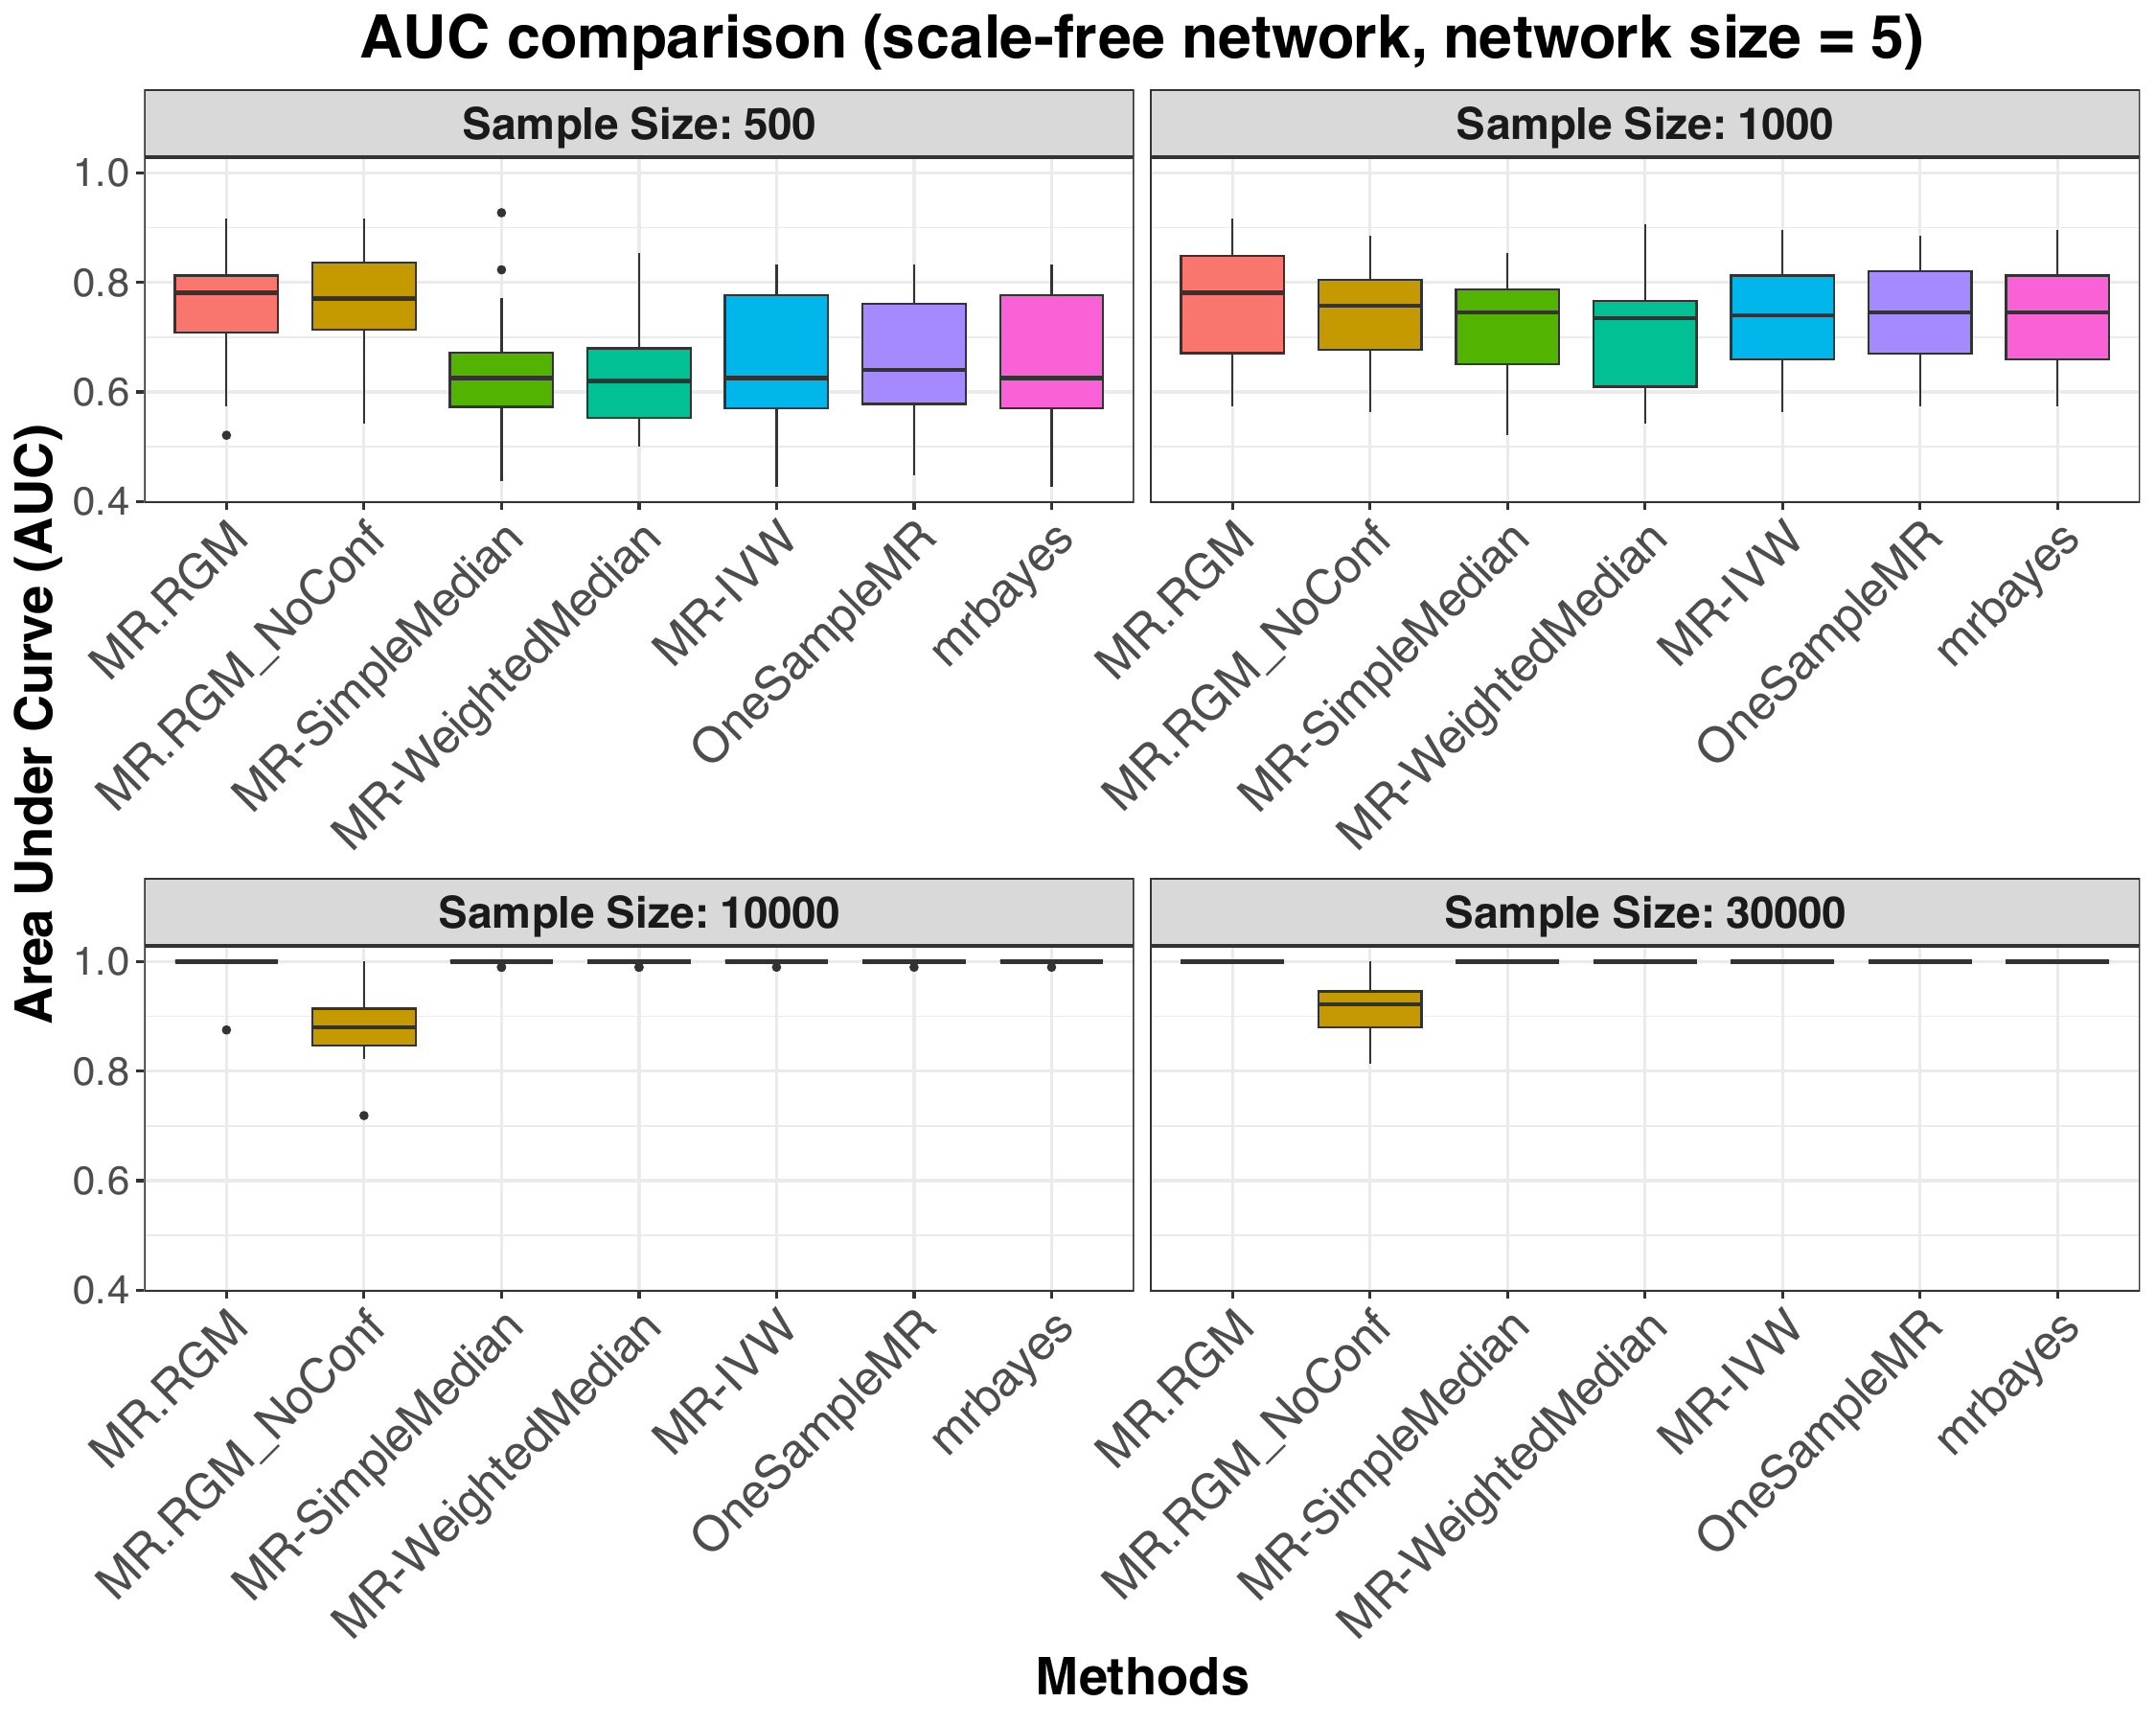}
    \caption{Graph recovery performance in a scale-free network with feedback loops and unmeasured confounding, with network size \(p{=}5\). Boxplots of AUC by method (x-axis) and sample size (facets; $n \in \{500,1000,10000,30000\}$).}
    \label{fig:sf_auc_p5}
\end{figure}

\begin{table}[htb]
\centering
\tiny
\caption{Graph recovery performance in a scale-free network with feedback loops and unmeasured confounding, with network size \(p{=}5\).}
\label{tab:feedback_graph_structure_scalefree_90_p=5}
\begin{tabular}{|c|c|c|c|c|c|}
\hline
\textbf{Setting} & \textbf{Method} & \textbf{AUC} & \textbf{TPR} & \textbf{FDR} & \textbf{MCC} \\
\hline
% \multicolumn{6}{|c|}{\textbf{p = 5, Variance Explained = 90\%}} \\
\hline
n = 500     & \texttt{MR.RGM}           & 0.754 (0.097) & 0.500 (0.125) & 0.298 (0.179) & 0.381 (0.208) \\
            & \texttt{MR.RGM\_NoConf}   & 0.756 (0.097) & 0.556 (0.092) & 0.338 (0.157) & 0.361 (0.164) \\
            % & \texttt{GRIVET}        & 0.500 (0.000) & 0.000 (0.000) & 0.000 (0.000) & 0.000 (0.000) \\
            & \texttt{MR-SimpleMedian}  & 0.641 (0.117) & 0.056 (0.075) & 0.231 (0.389) & 0.055 (0.174) \\
            & \texttt{MR-WeightedMedian}& 0.630 (0.098) & 0.069 (0.095) & 0.287 (0.388) & 0.045 (0.180) \\
            & \texttt{MR-IVW}           & 0.653 (0.122) & 0.174 (0.119) & 0.213 (0.247) & 0.203 (0.193) \\
            % & \texttt{MR-Egger}      & 0.551 (0.061) & 0.049 (0.103) & 0.361 (0.466) & 0.008 (0.201) \\
            % & \texttt{MR-Intercept}  & 0.577 (0.062) & 0.035 (0.056) & 0.278 (0.448) & 0.026 (0.176) \\
            & \texttt{OneSampleMR}      & 0.661 (0.108) & 0.174 (0.119) & 0.199 (0.238) & 0.207 (0.180) \\
            & \texttt{mrbayes}          & 0.654 (0.121) & 0.174 (0.119) & 0.222 (0.261) & 0.197 (0.200) \\
\hline
n = 1000    & \texttt{MR.RGM}           & 0.771 (0.111) & 0.549 (0.187) & 0.235 (0.141) & 0.468 (0.182) \\
            & \texttt{MR.RGM\_NoConf}   & 0.749 (0.101) & 0.605 (0.173) & 0.308 (0.158) & 0.426 (0.213) \\
            % & \texttt{GRIVET}        & 0.500 (0.000) & 0.000 (0.000) & 0.000 (0.000) & 0.000 (0.000) \\
            & \texttt{MR-SimpleMedian}  & 0.721 (0.099) & 0.132 (0.088) & 0.194 (0.231) & 0.160 (0.135) \\
            & \texttt{MR-WeightedMedian}& 0.703 (0.099) & 0.174 (0.133) & 0.349 (0.359) & 0.160 (0.208) \\
            & \texttt{MR-IVW}           & 0.742 (0.093) & 0.278 (0.142) & 0.299 (0.274) & 0.260 (0.206) \\
            % & \texttt{MR-Egger}      & 0.595 (0.089) & 0.035 (0.070) & 0.296 (0.410) & -0.015 (0.140) \\
            % & \texttt{MR-Intercept}  & 0.591 (0.098) & 0.021 (0.047) & 0.333 (0.441) & -0.038 (0.132) \\
            & \texttt{OneSampleMR}      & 0.744 (0.090) & 0.264 (0.155) & 0.298 (0.281) & 0.243 (0.224) \\
            & \texttt{mrbayes}          & 0.742 (0.093) & 0.264 (0.155) & 0.307 (0.285) & 0.236 (0.226) \\
\hline
n = 10000   & \texttt{MR.RGM}           & 0.993 (0.029) & 0.965 (0.056) & 0.000 (0.000) & 0.972 (0.045) \\
            & \texttt{MR.RGM\_NoConf}   & 0.884 (0.066) & 0.831 (0.154) & 0.336 (0.078) & 0.538 (0.105) \\
            % & \texttt{GRIVET}        & 0.500 (0.000) & 0.000 (0.000) & 0.000 (0.000) & 0.000 (0.000) \\
            & \texttt{MR-SimpleMedian}  & 0.999 (0.003) & 0.972 (0.052) & 0.044 (0.055) & 0.939 (0.060) \\
            & \texttt{MR-WeightedMedian}& 0.999 (0.003) & 0.972 (0.052) & 0.044 (0.055) & 0.939 (0.060) \\
            & \texttt{MR-IVW}           & 0.999 (0.002) & 0.993 (0.029) & 0.037 (0.052) & 0.962 (0.048) \\
            % & \texttt{MR-Egger}      & 0.604 (0.085) & 0.049 (0.094) & 0.133 (0.320) & 0.055 (0.147) \\
            % & \texttt{MR-Intercept}  & 0.593 (0.087) & 0.042 (0.072) & 0.139 (0.325) & 0.047 (0.141) \\
            & \texttt{OneSampleMR}      & 0.999 (0.002) & 0.993 (0.029) & 0.043 (0.054) & 0.957 (0.049) \\
            & \texttt{mrbayes}          & 1.000 (0.001) & 0.993 (0.029) & 0.037 (0.052) & 0.962 (0.048) \\
\hline
n = 30000   & \texttt{MR.RGM}           & 1.000 (0.000) & 1.000 (0.000) & 0.000 (0.000) & 1.000 (0.000) \\
            & \texttt{MR.RGM\_NoConf}   & 0.910 (0.051) & 0.888 (0.142) & 0.273 (0.124) & 0.640 (0.095) \\
            % & \texttt{GRIVET}        & 0.500 (0.000) & 0.000 (0.000) & 0.000 (0.000) & 0.000 (0.000) \\
            & \texttt{MR-SimpleMedian}  & 1.000 (0.000) & 1.000 (0.000) & 0.087 (0.081) & 0.922 (0.075) \\
            & \texttt{MR-WeightedMedian}& 1.000 (0.000) & 1.000 (0.000) & 0.087 (0.081) & 0.922 (0.075) \\
            & \texttt{MR-IVW}           & 1.000 (0.000) & 1.000 (0.000) & 0.111 (0.097) & 0.898 (0.092) \\
            % & \texttt{MR-Egger}      & 0.570 (0.096) & 0.021 (0.052) & 0.481 (0.458) & -0.073 (0.106) \\
            % & \texttt{MR-Intercept}  & 0.578 (0.091) & 0.028 (0.052) & 0.426 (0.452) & -0.047 (0.129) \\
            & \texttt{OneSampleMR}      & 1.000 (0.000) & 1.000 (0.000) & 0.111 (0.097) & 0.898 (0.092) \\
            & \texttt{mrbayes}          & 1.000 (0.000) & 1.000 (0.000) & 0.111 (0.097) & 0.898 (0.092) \\
\hline
\end{tabular}
\end{table}

\begin{figure}[htb]
    \centering
    \includegraphics[width=.7\textwidth]{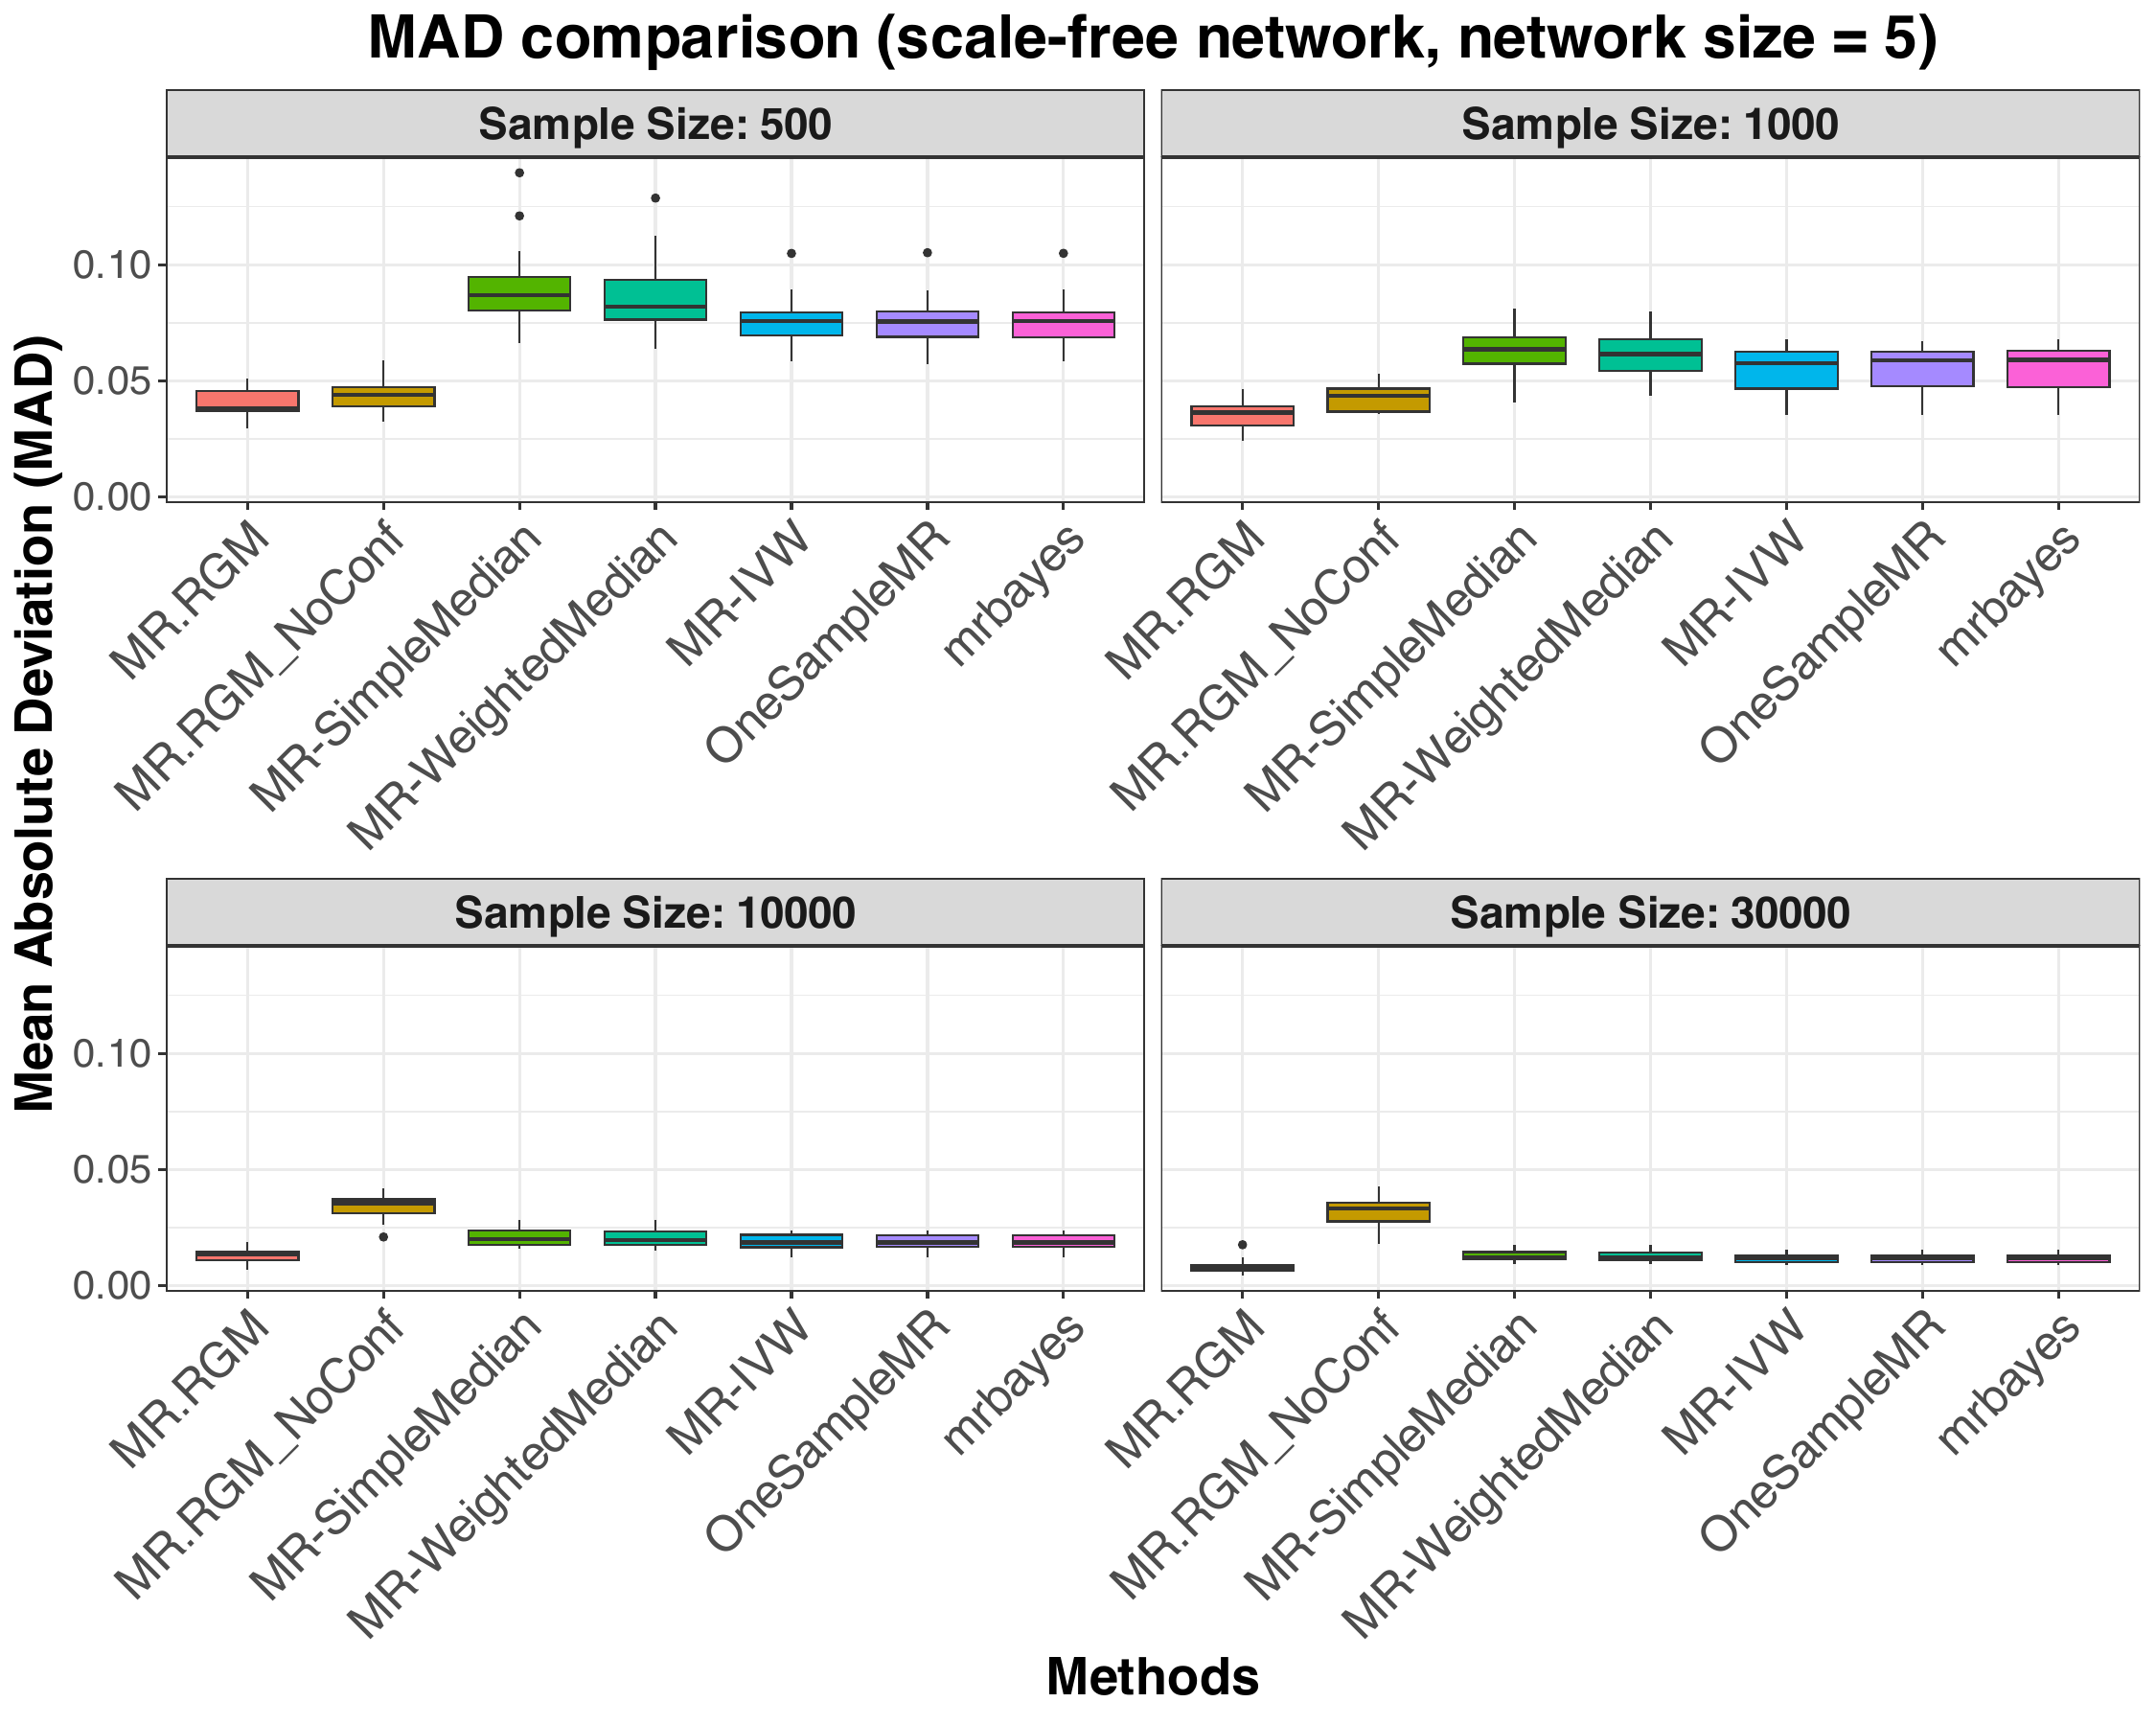}
    \caption{Causal effect estimation performance in a scale-free network with feedback loops and unmeasured confounding, with network size $p = 5$. Boxplots of mean absolute deviation (MAD) by method (x-axis) and sample size (facets; \(n \in \{500,1000,10000,30000\}\)). 
    % Each box summarizes 20 replicates; lower values indicate smaller estimation error.
    }
    \label{fig:sf_mad_p5}
\end{figure}

\begin{table}[htb]
\centering
\tiny
\caption{Causal effect estimation performance in a scale-free network with feedback loops and unmeasured confounding, with network size $p = 5$.}
\label{tab:feedback_causal_effect_scalefree_90_p=5}
\begin{tabular}{|c|c|c|c|c|}
\hline
\textbf{Setting} & \textbf{Method} & \textbf{MaxAbsDev} & \textbf{MeanAbsDev} & \textbf{MeanSqDev} \\
\hline
% \multicolumn{5}{|c|}{\textbf{p = 5, Variance Explained = 90\%}} \\
\hline
n = 500     & \texttt{MR.RGM}            & 0.119 (0.018) & 0.040 (0.006) & 0.003 (0.001) \\
            & \texttt{MR.RGM\_NoConf}    & 0.130 (0.021) & 0.045 (0.007) & 0.003 (0.001) \\
            % & \texttt{GRIVET}        & 0.100 (0.000) & 0.040 (0.000) & 0.004 (0.000) \\
            & \texttt{MR-SimpleMedian}   & 0.253 (0.052) & 0.090 (0.017) & 0.013 (0.004) \\
            & \texttt{MR-WeightedMedian} & 0.242 (0.051) & 0.086 (0.016) & 0.012 (0.004) \\
            & \texttt{MR-IVW}            & 0.210 (0.053) & 0.076 (0.010) & 0.009 (0.002) \\
            % & \texttt{MR-Egger}       & 4.256 (2.195) & 0.979 (0.272) & 2.450 (1.866) \\
            % & \texttt{MR-Intercept}   & 4.100 (2.096) & 0.983 (0.271) & 2.377 (1.798) \\
            & \texttt{OneSampleMR}       & 0.209 (0.054) & 0.075 (0.010) & 0.009 (0.002) \\
            & \texttt{mrbayes}           & 0.210 (0.054) & 0.076 (0.010) & 0.009 (0.002) \\
\hline
n = 1000    & \texttt{MR.RGM}            & 0.101 (0.015) & 0.036 (0.006) & 0.002 (0.001) \\
            & \texttt{MR.RGM\_NoConf}    & 0.118 (0.020) & 0.042 (0.006) & 0.003 (0.001) \\
            % & \texttt{GRIVET}        & 0.100 (0.000) & 0.040 (0.000) & 0.004 (0.000) \\
            & \texttt{MR-SimpleMedian}   & 0.175 (0.037) & 0.062 (0.010) & 0.006 (0.002) \\
            & \texttt{MR-WeightedMedian} & 0.174 (0.036) & 0.061 (0.010) & 0.006 (0.002) \\
            & \texttt{MR-IVW}            & 0.164 (0.035) & 0.055 (0.010) & 0.005 (0.001) \\
            % & \texttt{MR-Egger}       & 3.439 (1.508) & 0.923 (0.322) & 1.850 (1.365) \\
            % & \texttt{MR-Intercept}   & 3.425 (1.463) & 0.912 (0.336) & 1.829 (1.375) \\
            & \texttt{OneSampleMR}       & 0.165 (0.035) & 0.055 (0.009) & 0.005 (0.001) \\
            & \texttt{mrbayes}           & 0.165 (0.035) & 0.056 (0.010) & 0.005 (0.001) \\
\hline
n = 10000   & \texttt{MR.RGM}            & 0.046 (0.019) & 0.013 (0.003) & 0.0003 (0.0002) \\
            & \texttt{MR.RGM\_NoConf}    & 0.087 (0.013) & 0.034 (0.005) & 0.002 (0.0004) \\
            % & \texttt{GRIVET}        & 0.100 (0.000) & 0.040 (0.000) & 0.004 (0.000) \\
            & \texttt{MR-SimpleMedian}   & 0.059 (0.014) & 0.021 (0.004) & 0.001 (0.000) \\
            & \texttt{MR-WeightedMedian} & 0.058 (0.014) & 0.021 (0.004) & 0.001 (0.000) \\
            & \texttt{MR-IVW}            & 0.049 (0.010) & 0.019 (0.003) & 0.001 (0.000) \\
            % & \texttt{MR-Egger}       & 3.741 (2.160) & 0.964 (0.337) & 2.268 (2.354) \\
            % & \texttt{MR-Intercept}   & 3.781 (2.209) & 0.969 (0.345) & 2.307 (2.424) \\
            & \texttt{OneSampleMR}       & 0.049 (0.010) & 0.019 (0.003) & 0.001 (0.000) \\
            & \texttt{mrbayes}           & 0.049 (0.010) & 0.019 (0.003) & 0.001 (0.000) \\
\hline
n = 30000   & \texttt{MR.RGM}            & 0.030 (0.025) & 0.008 (0.003) & 0.0002 (0.0003) \\
            & \texttt{MR.RGM\_NoConf}    & 0.081 (0.012) & 0.032 (0.006) & 0.002 (0.0004) \\
            % & \texttt{GRIVET}        & 0.100 (0.000) & 0.040 (0.000) & 0.004 (0.000) \\
            & \texttt{MR-SimpleMedian}   & 0.035 (0.009) & 0.013 (0.002) & 0.0003 (0.0001) \\
            & \texttt{MR-WeightedMedian} & 0.035 (0.009) & 0.013 (0.002) & 0.0003 (0.0001) \\
            & \texttt{MR-IVW}            & 0.031 (0.005) & 0.012 (0.002) & 0.0002 (0.0001) \\
            % & \texttt{MR-Egger}       & 5.185 (8.200) & 1.117 (0.893) & 7.183 (23.790) \\
            % & \texttt{MR-Intercept}   & 5.185 (8.260) & 1.122 (0.892) & 7.249 (24.110) \\
            & \texttt{OneSampleMR}       & 0.031 (0.005) & 0.012 (0.002) & 0.0002 (0.0001) \\
            & \texttt{mrbayes}           & 0.031 (0.005) & 0.012 (0.002) & 0.0002 (0.0001) \\
\hline
\end{tabular}
\end{table}

\begin{figure}[htb]
    \centering
    \includegraphics[width=.7\textwidth]{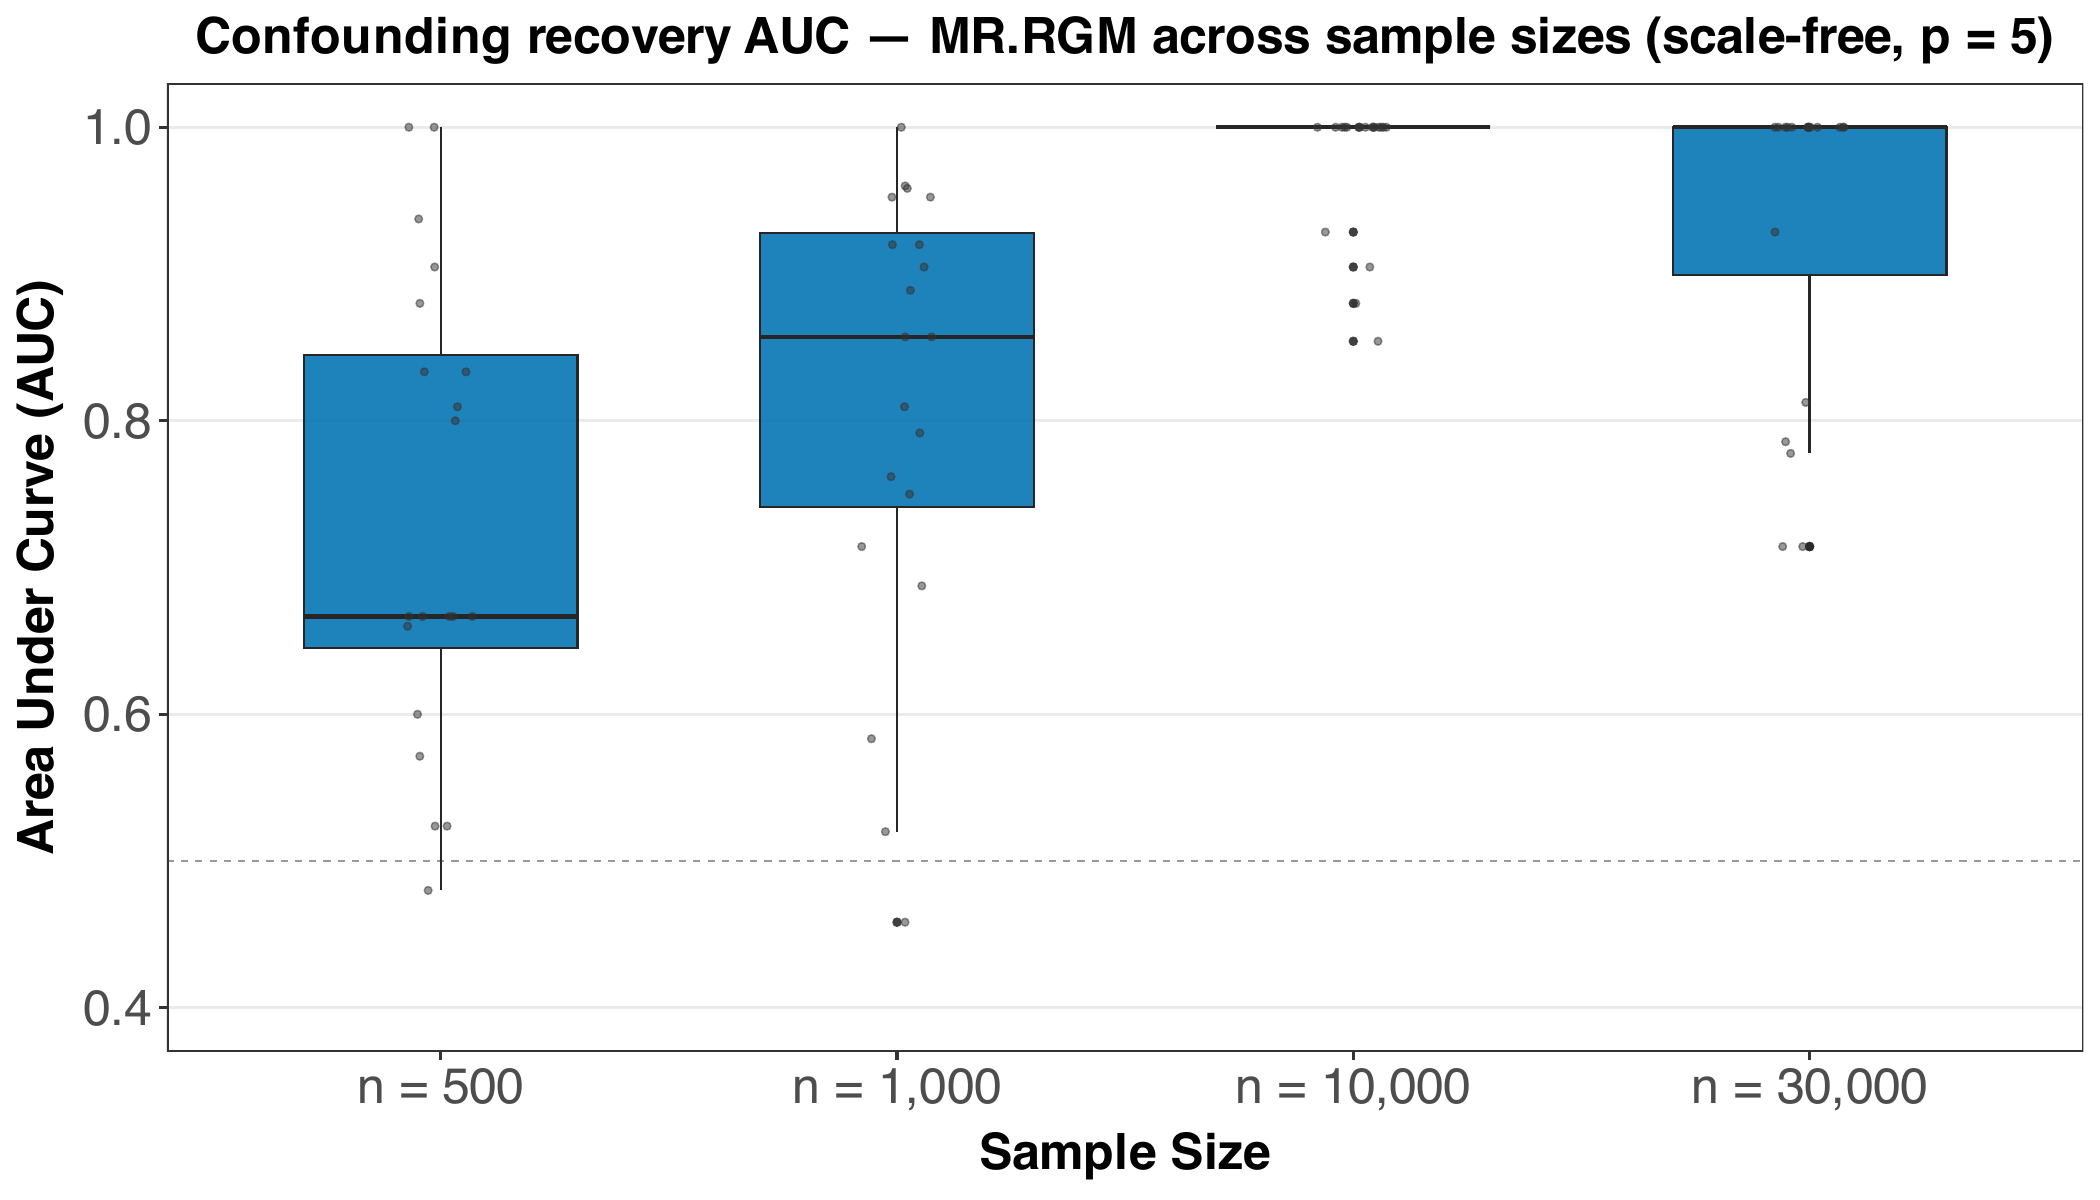}
    \caption{Confounding structure recovery performance using \texttt{MR.RGM} in a scale-free network with feedback loops and unmeasured confounding, with network size \(p=5\).
    Boxplots of AUC across sample sizes (\(n\in\{500,1000,10000,30000\}\)).}
    \label{fig:sf_conf_p5}
\end{figure}

\begin{table}[htb]
\centering
\small
\caption{Confounding structure recovery performance using \texttt{MR.RGM} in a scale-free network with feedback loops and unmeasured confounding, across network sizes \(p\in\{5,10\}\).}
% \caption{Confounding structure recovery performance with \texttt{MR.RGM} in a scale-free network with feedback loops and unmeasured confounding, with network size $p \in \{5, 10\}$. based on estimated posterior inclusion probabilities in \( \widehat{\mathbf{Z}} \) and the ground truth residual covariance structure \( \mathbf{DD}^T + \mathbf{\Sigma} \), when \texttt{MR.RGM} is applied using the true IV-trait indicator matrix.}
\label{tab:feedback_conf_auc_scalefree_A}
\begin{tabular}{|c|c|c|c|c|c|c|}
\hline
\textbf{Setting} & \textbf{Sample Size} & \textbf{AUC} & \textbf{TPR} & \textbf{FDR} & \textbf{MCC} \\
\hline
% \hline
% \multirow{4}{*}{p = 5, Var = 97\%} 
%     & 500  & 0.714 & 0.291 & 0.703 & -0.147 \\
%     & 1000 & 0.642 & 0.249 & 0.629 & -0.109 \\
%     & 10000 & 0.737 & 0.360 & 0.635 & -0.040 \\
%     & 30000 & 0.792 & 0.586 & 0.562 & 0.112 \\
\hline
\multirow{4}{*}{p = 5} 
    & 500 & 0.735 (0.156) & 0.307 (0.193) & 0.242 (0.296) & 0.219 (0.264) \\
    & 1000 & 0.812 (0.151) & 0.464 (0.214) & 0.255 (0.340) & 0.332 (0.342) \\
    & 10000 & 0.978 (0.045) & 0.952 (0.076) & 0.185 (0.283) & 0.728 (0.308) \\
    & 30000 & 0.937 (0.105) & 1.000 (0.000) & 0.203 (0.280) & 0.709 (0.378) \\
% \hline
% \multirow{4}{*}{p = 10, Var = 97\%} 
%     & 500  & 0.582 & 0.206 & 0.591 & -0.183 \\
%     & 1000 & 0.605 & 0.218 & 0.568 & -0.149 \\
%     & 10000 & 0.774 & 0.385 & 0.537 & -0.077 \\
%     & 30000 & 0.847 & 0.482 & 0.519 & -0.006 \\
\hline
\multirow{4}{*}{p = 10} 
    & 500 & 0.709 (0.081) & 0.242 (0.070) & 0.150 (0.115) & 0.210 (0.114) \\
    & 1000 & 0.804 (0.085) & 0.335 (0.076) & 0.110 (0.086) & 0.290 (0.148) \\
    & 10000 & 0.984 (0.018) & 0.886 (0.064) & 0.016 (0.027) & 0.839 (0.091) \\
    & 30000 & 0.996 (0.011) & 0.995 (0.013) & 0.007 (0.013) & 0.982 (0.029) \\
\hline
\end{tabular}
\end{table}

\subsection{Case \texorpdfstring{$2$}{2}: Small-world network with feedback loops and unmeasured confounding}

\noindent\textit{Overview.} Figure (\ref{fig:sw_auc_p5}) reports graph-recovery AUC (boxplots) by method across sample sizes for network size $p=5$. Tables (\ref{tab:feedback_graph_structure_smallworld_90_p=5}) and (\ref{tab:feedback_graph_structure_smallworld_90_p=10}) summarize graph-recovery metrics (AUC, TPR, FDR, MCC; mean $\pm$ sd) for $p\in\{5,10\}$. Figure (\ref{fig:sw_mad_p5}) shows causal-effect estimation error (MeanAbsDev; boxplots) by method across sample sizes for $p=5$, while Tables (\ref{tab:feedback_causal_effect_smallworld_90_p=5}) and (\ref{tab:feedback_causal_effect_smallworld_90_p=10}) report effect-estimation error metrics (MaxAbsDev, MeanAbsDev, MeanSqDev; mean $\pm$ sd) for $p\in\{5,10\}$. Finally, Figure (\ref{fig:sw_conf_p5}) presents confounding-structure recovery AUC (boxplots) for $p=5$ using \texttt{MR.RGM}, and Table (\ref{tab:feedback_conf_auc_smallworld_A}) compiles confounding-structure recovery metrics (AUC, TPR, FDR, MCC; mean $\pm$ sd) for $p\in\{5,10\}$ using \texttt{MR.RGM} across all sample sizes.

\begin{figure}[htb]
    \centering
    \includegraphics[width=.7\textwidth]{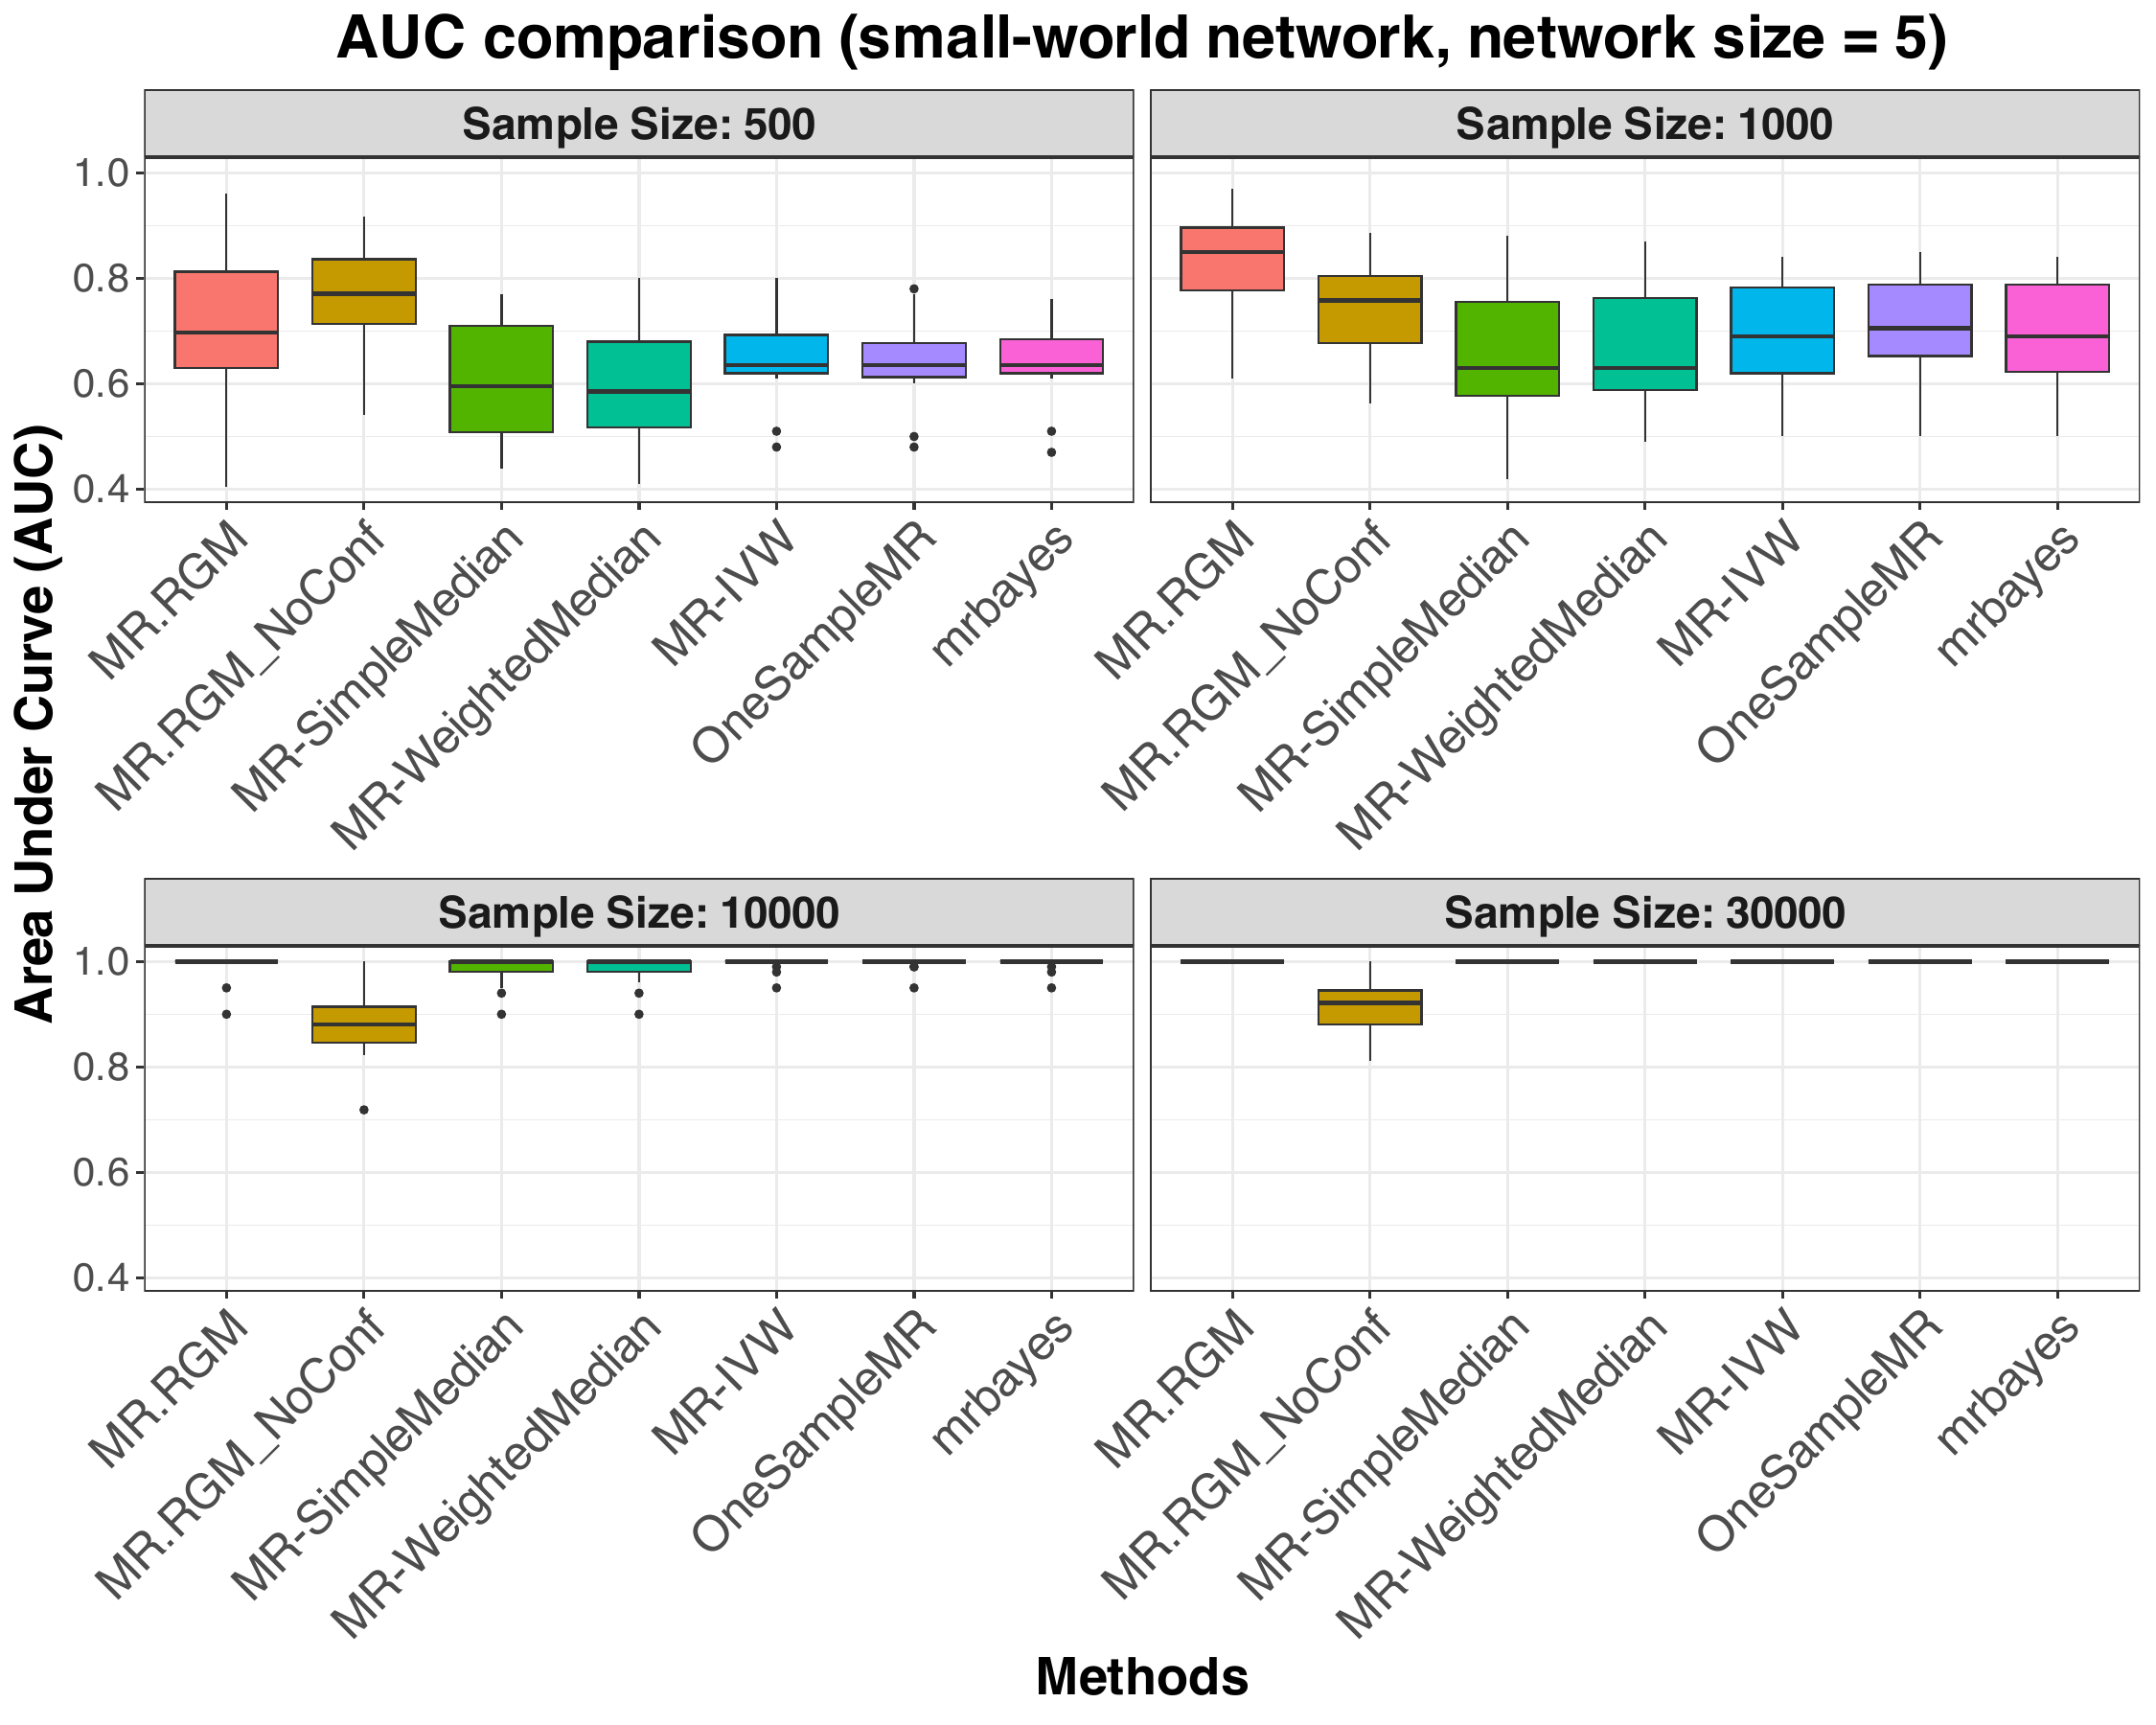}
    \caption{Graph recovery performance in a small-world network with feedback loops and unmeasured confounding, with network size \(p{=}5\). Boxplots of AUC by method (x-axis) and sample size (facets; \(n \in \{500,1000,10000,30000\}\)).}
    \label{fig:sw_auc_p5}
\end{figure}

\begin{table}[htb]
\centering
\tiny
\caption{Graph recovery performance in a small-world network with feedback loops and unmeasured confounding, with network size \(p{=}5\).}
\label{tab:feedback_graph_structure_smallworld_90_p=5}
\begin{tabular}{|c|c|c|c|c|c|}
\hline
\textbf{Setting} & \textbf{Method} & \textbf{AUC} & \textbf{TPR} & \textbf{FDR} & \textbf{MCC} \\
\hline
% \multicolumn{6}{|c|}{\textbf{p = 5, Variance Explained = 90\%}} \\
\hline
n = 500     & \texttt{MR.RGM}           & 0.712 (0.142) & 0.467 (0.183) & 0.282 (0.165) & 0.309 (0.219) \\
            & \texttt{MR.RGM\_NoConf}   & 0.763 (0.100) & 0.569 (0.086) & 0.352 (0.143) & 0.358 (0.168) \\
            % & \texttt{GRIVET}        & 0.500 (0.000) & 0.000 (0.000) & 0.000 (0.000) & 0.000 (0.000) \\
            & \texttt{MR-SimpleMedian}  & 0.607 (0.112) & 0.100 (0.089) & 0.179 (0.319) & 0.121 (0.174) \\
            & \texttt{MR-WeightedMedian}& 0.606 (0.111) & 0.135 (0.101) & 0.192 (0.326) & 0.161 (0.221) \\
            & \texttt{MR-IVW}           & 0.652 (0.075) & 0.195 (0.107) & 0.221 (0.315) & 0.214 (0.198) \\
            % & \texttt{MR-Egger}       & 0.576 (0.102) & 0.050 (0.067) & 0.192 (0.285) & 0.024 (0.106) \\
            % & \texttt{MR-Intercept}   & 0.605 (0.101) & 0.040 (0.058) & 0.167 (0.279) & 0.018 (0.092) \\
            & \texttt{OneSampleMR}      & 0.647 (0.078) & 0.200 (0.120) & 0.213 (0.331) & 0.224 (0.217) \\
            & \texttt{mrbayes}          & 0.646 (0.071) & 0.189 (0.110) & 0.213 (0.331) & 0.216 (0.208) \\
\hline
n = 1000    & \texttt{MR.RGM}           & 0.832 (0.087) & 0.561 (0.146) & 0.130 (0.105) & 0.513 (0.167) \\
            & \texttt{MR.RGM\_NoConf}   & 0.738 (0.099) & 0.594 (0.168) & 0.315 (0.165) & 0.411 (0.220) \\
            % & \texttt{GRIVET}        & 0.500 (0.000) & 0.000 (0.000) & 0.000 (0.000) & 0.000 (0.000) \\
            & \texttt{MR-SimpleMedian}  & 0.656 (0.121) & 0.160 (0.086) & 0.025 (0.109) & 0.260 (0.126) \\
            & \texttt{MR-WeightedMedian}& 0.668 (0.118) & 0.160 (0.097) & 0.067 (0.162) & 0.238 (0.144) \\
            & \texttt{MR-IVW}           & 0.699 (0.099) & 0.295 (0.156) & 0.128 (0.171) & 0.314 (0.175) \\
            % & \texttt{MR-Egger}       & 0.610 (0.095) & 0.035 (0.057) & 0.325 (0.455) & -0.017 (0.193) \\
            % & \texttt{MR-Intercept}   & 0.621 (0.085) & 0.035 (0.057) & 0.325 (0.430) & -0.028 (0.159) \\
            & \texttt{OneSampleMR}      & 0.712 (0.097) & 0.322 (0.155) & 0.091 (0.142) & 0.363 (0.155) \\
            & \texttt{mrbayes}          & 0.702 (0.098) & 0.317 (0.154) & 0.142 (0.174) & 0.323 (0.185) \\
\hline
n = 10000   & \texttt{MR.RGM}           & 0.992 (0.025) & 0.950 (0.060) & 0.006 (0.025) & 0.946 (0.075) \\
            & \texttt{MR.RGM\_NoConf}   & 0.887 (0.069) & 0.833 (0.161) & 0.331 (0.081) & 0.546 (0.106) \\
            % & \texttt{GRIVET}        & 0.500 (0.000) & 0.000 (0.000) & 0.000 (0.000) & 0.000 (0.000) \\
            & \texttt{MR-SimpleMedian}  & 0.984 (0.026) & 0.925 (0.062) & 0.041 (0.071) & 0.885 (0.101) \\
            & \texttt{MR-WeightedMedian}& 0.985 (0.025) & 0.935 (0.065) & 0.041 (0.071) & 0.894 (0.106) \\
            & \texttt{MR-IVW}           & 0.996 (0.012) & 0.990 (0.030) & 0.075 (0.083) & 0.908 (0.098) \\
            % & \texttt{MR-Egger}       & 0.589 (0.118) & 0.055 (0.097) & 0.375 (0.444) & -0.021 (0.196) \\
            % & \texttt{MR-Intercept}   & 0.587 (0.121) & 0.060 (0.102) & 0.350 (0.421) & -0.009 (0.192) \\
            & \texttt{OneSampleMR}      & 0.996 (0.012) & 0.989 (0.031) & 0.070 (0.077) & 0.912 (0.092) \\
            & \texttt{mrbayes}          & 0.996 (0.012) & 0.989 (0.031) & 0.065 (0.079) & 0.917 (0.094) \\
\hline
n = 30000   & \texttt{MR.RGM}           & 1.000 (0.000) & 1.000 (0.000) & 0.000 (0.000) & 1.000 (0.000) \\
            & \texttt{MR.RGM\_NoConf}   & 0.913 (0.053) & 0.882 (0.147) & 0.265 (0.126) & 0.645 (0.088) \\
            % & \texttt{GRIVET}        & 0.500 (0.000) & 0.000 (0.000) & 0.000 (0.000) & 0.000 (0.000) \\
            & \texttt{MR-SimpleMedian}  & 1.000 (0.000) & 1.000 (0.000) & 0.058 (0.056) & 0.939 (0.061) \\
            & \texttt{MR-WeightedMedian}& 1.000 (0.000) & 1.000 (0.000) & 0.058 (0.056) & 0.939 (0.061) \\
            & \texttt{MR-IVW}           & 1.000 (0.000) & 1.000 (0.000) & 0.091 (0.062) & 0.902 (0.068) \\
            % & \texttt{MR-Egger}       & 0.591 (0.106) & 0.025 (0.043) & 0.175 (0.363) & 0.001 (0.156) \\
            % & \texttt{MR-Intercept}   & 0.598 (0.105) & 0.020 (0.040) & 0.175 (0.363) & -0.010 (0.147) \\
            & \texttt{OneSampleMR}      & 1.000 (0.000) & 1.000 (0.000) & 0.087 (0.062) & 0.907 (0.068) \\
            & \texttt{mrbayes}          & 1.000 (0.000) & 1.000 (0.000) & 0.087 (0.062) & 0.907 (0.068) \\
\hline
\end{tabular}
\end{table}

\begin{table}[htb]
\centering
\tiny
\caption{Graph recovery performance in a small-world network with feedback loops and unmeasured confounding, with network size \(p{=}10\).}
\label{tab:feedback_graph_structure_smallworld_90_p=10}
\begin{tabular}{|c|c|c|c|c|c|}
\hline
\textbf{Setting} & \textbf{Method} & \textbf{AUC} & \textbf{TPR} & \textbf{FDR} & \textbf{MCC} \\
\hline
% \multicolumn{6}{|c|}{\textbf{p = 10, Variance Explained = 90\%}} \\
\hline
n = 500     & \texttt{MR.RGM}           & 0.737 (0.069) & 0.500 (0.100) & 0.494 (0.083) & 0.360 (0.100) \\
            & \texttt{MR.RGM\_NoConf}   & 0.796 (0.069) & 0.594 (0.107) & 0.544 (0.091) & 0.378 (0.122) \\
            % & \texttt{GRIVET}        & 0.500 (0.000) & 0.000 (0.000) & 0.000 (0.000) & 0.000 (0.000) \\
            & \texttt{MR-SimpleMedian}  & 0.593 (0.081) & 0.065 (0.050) & 0.490 (0.360) & 0.095 (0.121) \\
            & \texttt{MR-WeightedMedian}& 0.602 (0.083) & 0.093 (0.062) & 0.540 (0.297) & 0.111 (0.136) \\
            & \texttt{MR-IVW}           & 0.651 (0.066) & 0.175 (0.068) & 0.479 (0.200) & 0.196 (0.113) \\
            % & \texttt{MR-Egger}       & 0.557 (0.053) & 0.055 (0.055) & 0.683 (0.257) & 0.036 (0.100) \\
            % & \texttt{MR-Intercept}   & 0.561 (0.059) & 0.043 (0.055) & 0.723 (0.309) & 0.008 (0.113) \\
            & \texttt{OneSampleMR}      & 0.654 (0.070) & 0.186 (0.072) & 0.478 (0.199) & 0.202 (0.116) \\
            & \texttt{mrbayes}          & 0.650 (0.069) & 0.175 (0.071) & 0.484 (0.195) & 0.194 (0.111) \\
\hline
n = 1000    & \texttt{MR.RGM}           & 0.813 (0.052) & 0.594 (0.109) & 0.379 (0.078) & 0.498 (0.100) \\
            & \texttt{MR.RGM\_NoConf}   & 0.796 (0.069) & 0.594 (0.107) & 0.544 (0.091) & 0.378 (0.122) \\
            % & \texttt{GRIVET}        & 0.500 (0.000) & 0.000 (0.000) & 0.000 (0.000) & 0.000 (0.000) \\
            & \texttt{MR-SimpleMedian}  & 0.698 (0.093) & 0.218 (0.088) & 0.331 (0.191) & 0.293 (0.125) \\
            & \texttt{MR-WeightedMedian}& 0.712 (0.090) & 0.240 (0.083) & 0.345 (0.132) & 0.303 (0.096) \\
            & \texttt{MR-IVW}           & 0.761 (0.061) & 0.360 (0.116) & 0.316 (0.091) & 0.398 (0.088) \\
            % & \texttt{MR-Egger}       & 0.558 (0.050) & 0.020 (0.033) & 0.830 (0.266) & -0.035 (0.085) \\
            % & \texttt{MR-Intercept}   & 0.562 (0.062) & 0.018 (0.024) & 0.848 (0.240) & -0.044 (0.062) \\
            & \texttt{OneSampleMR}      & 0.758 (0.063) & 0.375 (0.110) & 0.312 (0.075) & 0.411 (0.081) \\
            & \texttt{mrbayes}          & 0.756 (0.062) & 0.367 (0.120) & 0.321 (0.085) & 0.400 (0.090) \\
\hline
n = 10000   & \texttt{MR.RGM}           & 0.994 (0.016) & 0.972 (0.042) & 0.032 (0.031) & 0.961 (0.031) \\
            & \texttt{MR.RGM\_NoConf}   & 0.919 (0.029) & 0.905 (0.077) & 0.491 (0.059) & 0.572 (0.070) \\
            % & \texttt{GRIVET}        & 0.500 (0.000) & 0.000 (0.000) & 0.000 (0.000) & 0.000 (0.000) \\
            & \texttt{MR-SimpleMedian}  & 0.994 (0.007) & 0.955 (0.061) & 0.128 (0.064) & 0.885 (0.066) \\
            & \texttt{MR-WeightedMedian}& 0.994 (0.007) & 0.963 (0.061) & 0.135 (0.062) & 0.885 (0.062) \\
            & \texttt{MR-IVW}           & 0.998 (0.003) & 0.993 (0.024) & 0.156 (0.075) & 0.888 (0.060) \\
            % & \texttt{MR-Egger}       & 0.552 (0.052) & 0.053 (0.046) & 0.717 (0.256) & 0.022 (0.111) \\
            % & \texttt{MR-Intercept}   & 0.543 (0.059) & 0.048 (0.049) & 0.742 (0.253) & 0.004 (0.099) \\
            & \texttt{OneSampleMR}      & 0.998 (0.003) & 0.992 (0.025) & 0.156 (0.082) & 0.887 (0.065) \\
            & \texttt{mrbayes}          & 0.998 (0.003) & 0.992 (0.025) & 0.156 (0.082) & 0.887 (0.065) \\
\hline
n = 30000   & \texttt{MR.RGM}           & 1.000 (0.002) & 0.994 (0.016) & 0.000 (0.000) & 1.000 (0.010) \\
            & \texttt{MR.RGM\_NoConf}   & 0.941 (0.032) & 0.921 (0.054) & 0.455 (0.053) & 0.615 (0.059) \\
            % & \texttt{GRIVET}        & 0.500 (0.000) & 0.000 (0.000) & 0.000 (0.000) & 0.000 (0.000) \\
            & \texttt{MR-SimpleMedian}  & 1.000 (0.000) & 1.000 (0.000) & 0.146 (0.052) & 0.901 (0.036) \\
            & \texttt{MR-WeightedMedian}& 1.000 (0.000) & 1.000 (0.000) & 0.148 (0.049) & 0.899 (0.035) \\
            & \texttt{MR-IVW}           & 1.000 (0.000) & 1.000 (0.000) & 0.183 (0.058) & 0.873 (0.042) \\
            % & \texttt{MR-Egger}       & 0.555 (0.052) & 0.025 (0.030) & 0.777 (0.306) & -0.035 (0.075) \\
            % & \texttt{MR-Intercept}   & 0.557 (0.051) & 0.030 (0.029) & 0.752 (0.297) & -0.024 (0.073) \\
            & \texttt{OneSampleMR}      & 1.000 (0.000) & 1.000 (0.000) & 0.188 (0.066) & 0.870 (0.048) \\
            & \texttt{mrbayes}          & 1.000 (0.000) & 1.000 (0.000) & 0.190 (0.061) & 0.868 (0.045) \\
\hline
\end{tabular}
\end{table}

\begin{figure}[htb]
    \centering
    \includegraphics[width=.7\textwidth]{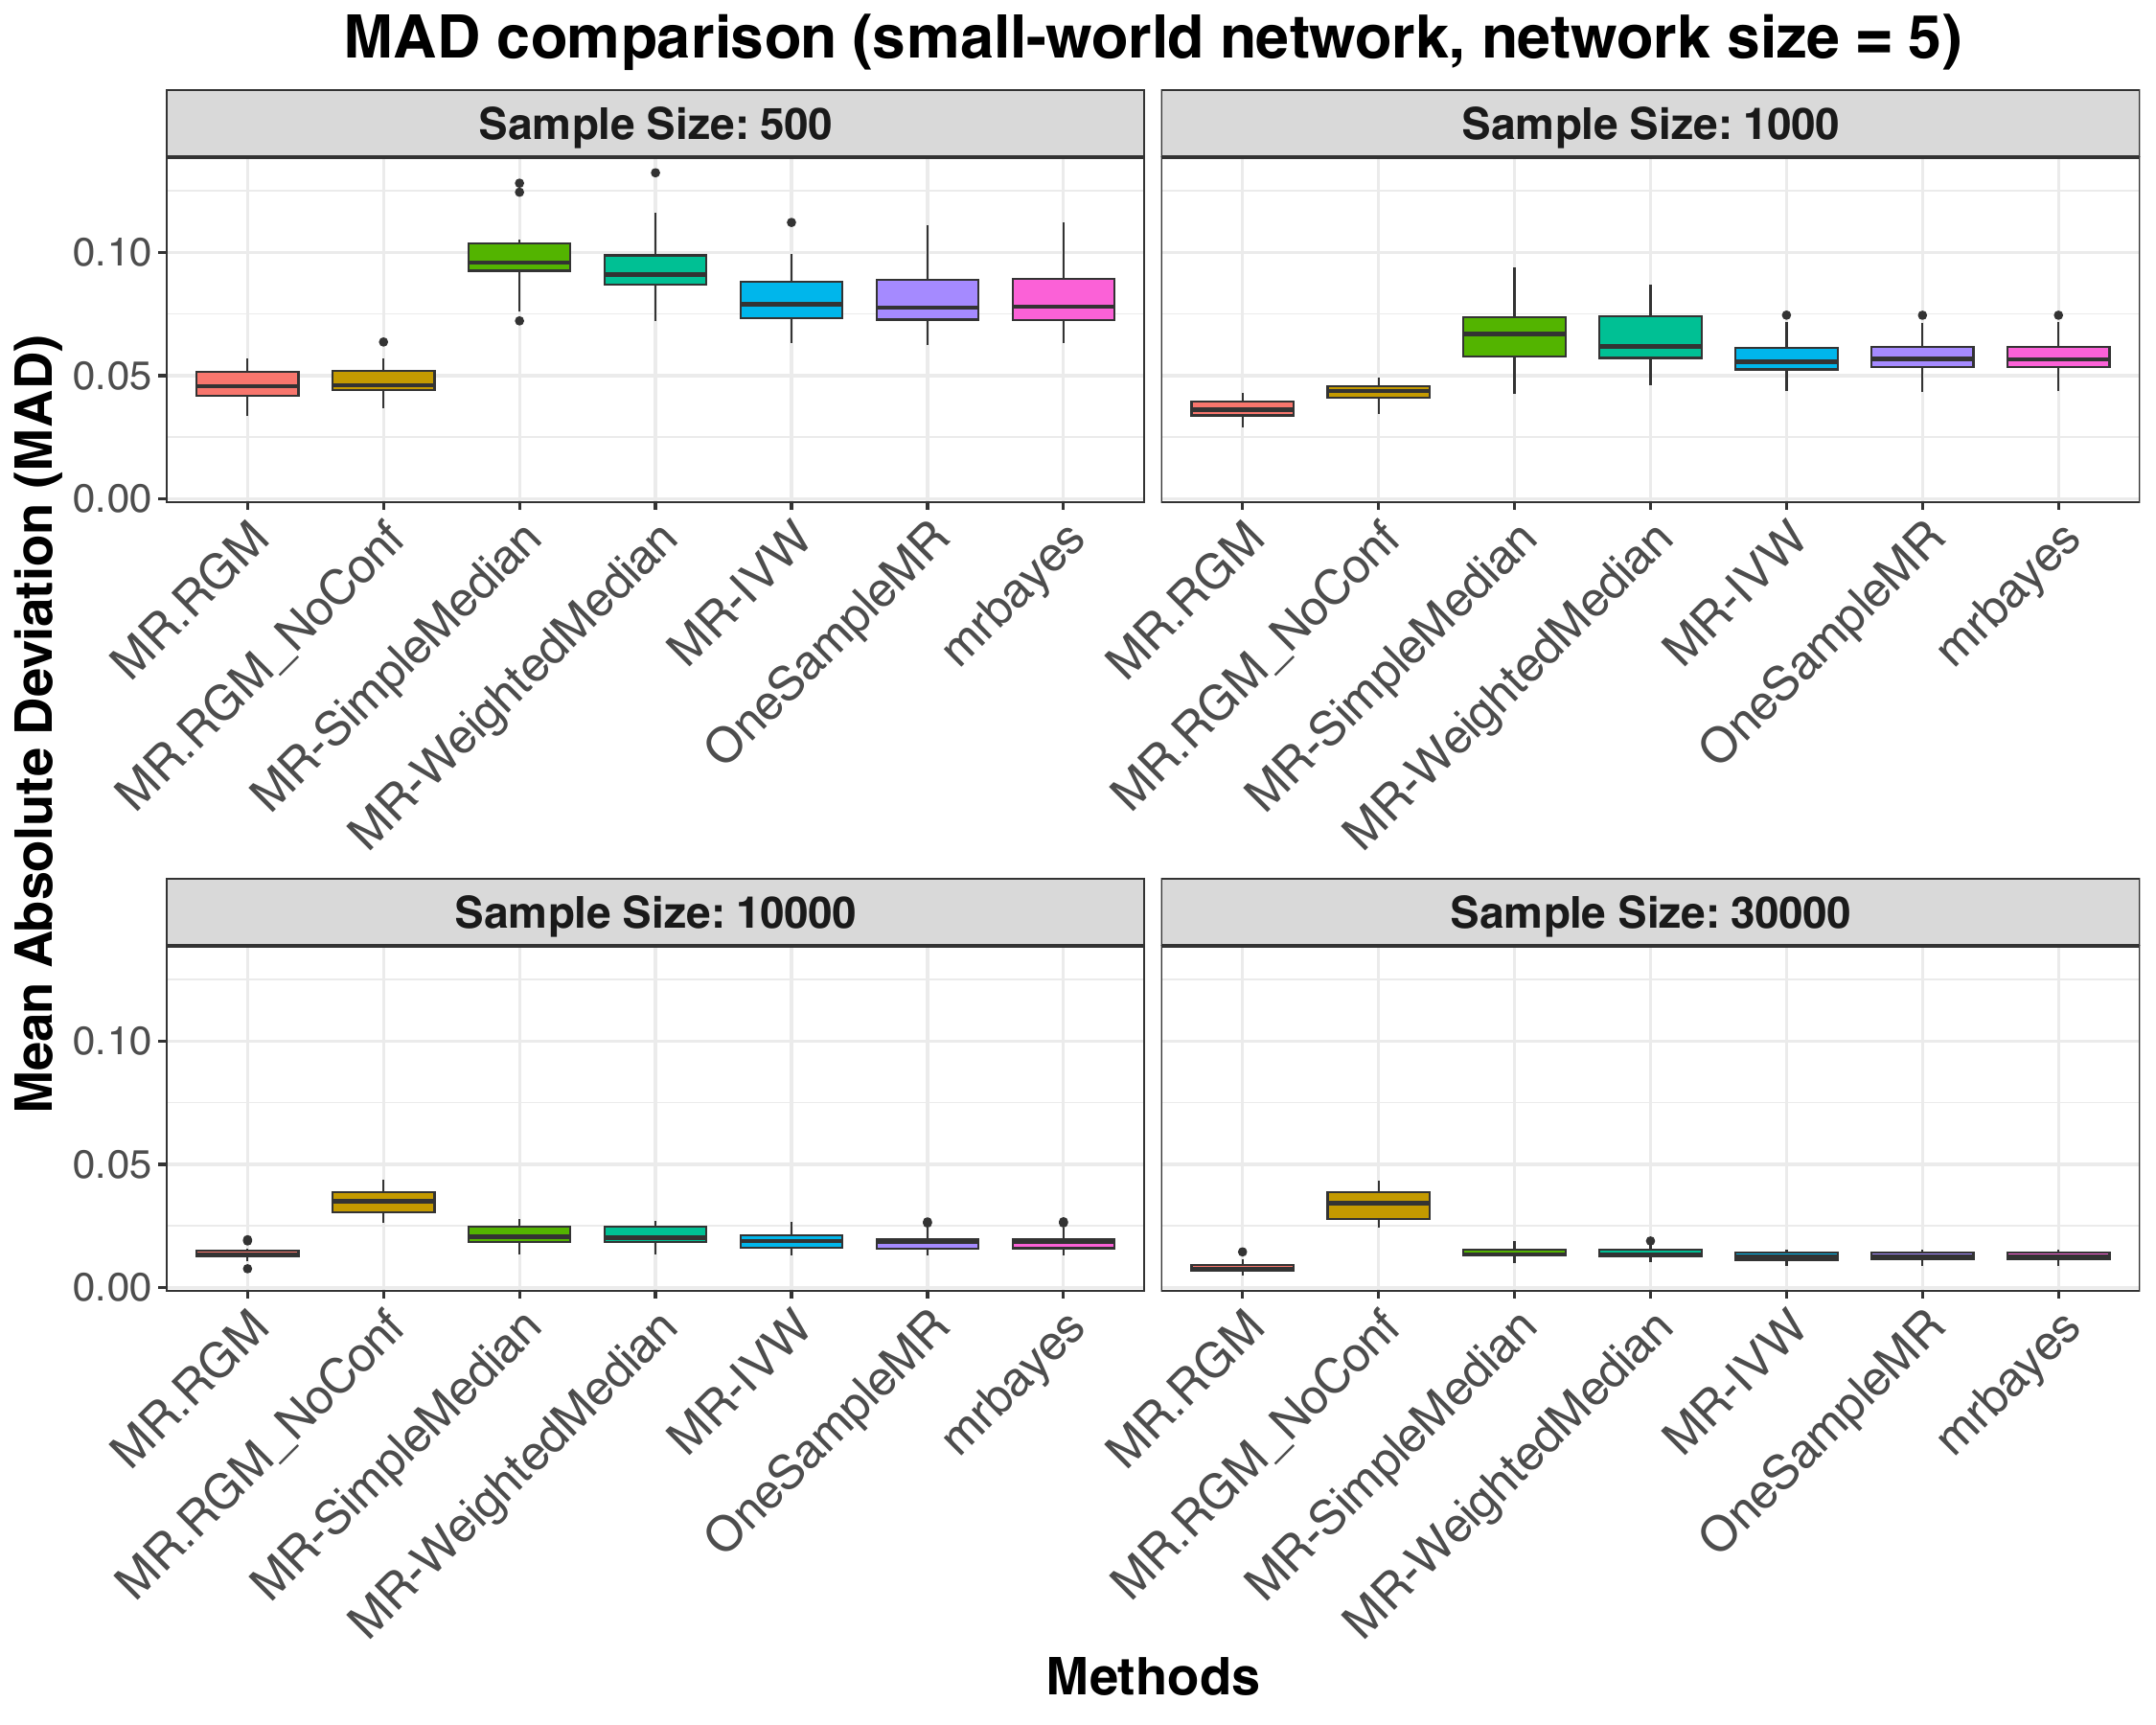}
    \caption{Causal effect estimation performance in a small-world network with feedback loops and
    unmeasured confounding, with network size \(p{=}5\). Boxplots of mean absolute deviation (MAD) by method (x-axis) and sample size (facets; \(n \in \{500,1000,10000,30000\}\)). 
    % Lower values indicate smaller estimation error.
    }
    \label{fig:sw_mad_p5}
\end{figure}

\begin{table}[htb]
\centering
\tiny
\caption{Causal effect estimation performance in a small-world network with feedback loops and unmeasured confounding, with network size \(p{=}5\).}
\label{tab:feedback_causal_effect_smallworld_90_p=5}
\begin{tabular}{|c|c|c|c|c|}
\hline
\textbf{Setting} & \textbf{Method} & \textbf{MaxAbsDev} & \textbf{MeanAbsDev} & \textbf{MeanSqDev} \\
\hline
% \multicolumn{5}{|c|}{\textbf{p = 5, Variance Explained = 90\%}} \\
\hline
n = 500     & \texttt{MR.RGM}           & 0.127 (0.022) & 0.045 (0.007) & 0.003 (0.001) \\
            & \texttt{MR.RGM\_NoConf}   & 0.140 (0.033) & 0.048 (0.006) & 0.004 (0.001) \\
            % & \texttt{GRIVET}        & 0.135 (0.043) & 0.044 (0.007) & 0.005 (0.001) \\
            & \texttt{MR-SimpleMedian}  & 0.259 (0.048) & 0.097 (0.013) & 0.015 (0.004) \\
            & \texttt{MR-WeightedMedian}& 0.253 (0.041) & 0.094 (0.013) & 0.014 (0.003) \\
            & \texttt{MR-IVW}           & 0.222 (0.042) & 0.081 (0.012) & 0.010 (0.003) \\
            % & \texttt{MR-Egger}       & 3.930 (2.420) & 0.854 (0.311) & 2.160 (2.097) \\
            % & \texttt{MR-Intercept}   & 3.811 (2.449) & 0.851 (0.318) & 2.101 (2.104) \\
            & \texttt{OneSampleMR}      & 0.216 (0.041) & 0.081 (0.012) & 0.010 (0.003) \\
            & \texttt{mrbayes}          & 0.217 (0.040) & 0.081 (0.012) & 0.010 (0.003) \\
\hline
n = 1000    & \texttt{MR.RGM}           & 0.106 (0.022) & 0.036 (0.004) & 0.002 (0.0004) \\
            & \texttt{MR.RGM\_NoConf}   & 0.134 (0.024) & 0.043 (0.004) & 0.003 (0.001) \\
            % & \texttt{GRIVET}        & 0.108 (0.019) & 0.039 (0.009) & 0.004 (0.001) \\
            & \texttt{MR-SimpleMedian}  & 0.167 (0.031) & 0.067 (0.013) & 0.007 (0.002) \\
            & \texttt{MR-WeightedMedian}& 0.160 (0.019) & 0.065 (0.011) & 0.006 (0.002) \\
            & \texttt{MR-IVW}           & 0.144 (0.030) & 0.057 (0.008) & 0.005 (0.001) \\
            % & \texttt{MR-Egger}       & 4.304 (2.877) & 1.102 (0.581) & 3.217 (5.231) \\
            % & \texttt{MR-Intercept}   & 4.444 (3.320) & 1.124 (0.618) & 3.548 (6.426) \\
            & \texttt{OneSampleMR}      & 0.148 (0.027) & 0.058 (0.008) & 0.005 (0.001) \\
            & \texttt{mrbayes}          & 0.148 (0.027) & 0.058 (0.008) & 0.005 (0.001) \\
\hline
n = 10000   & \texttt{MR.RGM}           & 0.045 (0.010) & 0.014 (0.003) & 0.0003 (0.0001) \\
            & \texttt{MR.RGM\_NoConf}   & 0.095 (0.016) & 0.035 (0.005) & 0.002 (0.0005) \\
            % & \texttt{GRIVET}        & 0.091 (0.022) & 0.032 (0.014) & 0.003 (0.002) \\
            & \texttt{MR-SimpleMedian}  & 0.057 (0.012) & 0.021 (0.004) & 0.001 (0.0003) \\
            & \texttt{MR-WeightedMedian}& 0.057 (0.012) & 0.021 (0.004) & 0.001 (0.0003) \\
            & \texttt{MR-IVW}           & 0.051 (0.010) & 0.019 (0.004) & 0.001 (0.0002) \\
            % & \texttt{MR-Egger}       & 3.996 (5.340) & 0.980 (0.630)  & 3.821 (10.558) \\
            % & \texttt{MR-Intercept}   & 4.026 (5.434) & 0.978 (0.630)  & 3.883 (10.894) \\
            & \texttt{OneSampleMR}      & 0.050 (0.009) & 0.019 (0.004) & 0.001 (0.0002) \\
            & \texttt{mrbayes}          & 0.050 (0.009) & 0.019 (0.004) & 0.001 (0.0002) \\
\hline
n = 30000   & \texttt{MR.RGM}           & 0.033 (0.029) & 0.008 (0.002) & 0.0002 (0.0002) \\
            & \texttt{MR.RGM\_NoConf}   & 0.089 (0.018) & 0.033 (0.006) & 0.002 (0.0004) \\
            % & \texttt{GRIVET}        & 0.088 (0.029) & 0.032 (0.016) & 0.003 (0.002) \\
            & \texttt{MR-SimpleMedian}  & 0.038 (0.010) & 0.014 (0.002) & 0.0003 (0.0001) \\
            & \texttt{MR-WeightedMedian}& 0.038 (0.009) & 0.014 (0.002) & 0.0003 (0.0001) \\
            & \texttt{MR-IVW}           & 0.037 (0.008) & 0.013 (0.002) & 0.0003 (0.0001) \\
            % & \texttt{MR-Egger}       & 6.145 (6.975) & 1.259 (0.678) & 6.541 (12.082) \\
            % & \texttt{MR-Intercept}   & 6.072 (6.853) & 1.259 (0.666) & 6.406 (11.632) \\
            & \texttt{OneSampleMR}      & 0.036 (0.008) & 0.013 (0.002) & 0.0003 (0.0001) \\
            & \texttt{mrbayes}          & 0.036 (0.008) & 0.013 (0.002) & 0.0003 (0.0001) \\
\hline
\end{tabular}
\end{table}

\begin{table}[htb]
\centering
\tiny
\caption{Causal effect estimation performance in a small-world network with feedback loops and unmeasured confounding, with network size \(p{=}10\).}
\label{tab:feedback_causal_effect_smallworld_90_p=10}
\begin{tabular}{|c|c|c|c|c|}
\hline
\textbf{Setting} & \textbf{Method} & \textbf{MaxAbsDev} & \textbf{MeanAbsDev} & \textbf{MeanSqDev} \\
\hline
% \multicolumn{5}{|c|}{\textbf{p = 10, Variance Explained = 90\%}} \\
\hline
n = 500     & \texttt{MR.RGM}           & 0.153 (0.034) & 0.036 (0.004) & 0.002 (0.001) \\
            & \texttt{MR.RGM\_NoConf}   & 0.175 (0.034) & 0.040 (0.004) & 0.003 (0.001) \\
            % & \texttt{GRIVET}        & 0.171 (0.058) & 0.026 (0.004) & 0.003 (0.001) \\
            & \texttt{MR-SimpleMedian}  & 0.336 (0.076) & 0.094 (0.011) & 0.014 (0.003) \\
            & \texttt{MR-WeightedMedian}& 0.325 (0.058) & 0.089 (0.012) & 0.013 (0.003) \\
            & \texttt{MR-IVW}           & 0.299 (0.064) & 0.081 (0.010) & 0.011 (0.003) \\
            % & \texttt{MR-Egger}       & 7.031 (4.259) & 1.102 (0.410) & 3.533 (3.534) \\
            % & \texttt{MR-Intercept}   & 7.030 (4.345) & 1.098 (0.394) & 3.452 (3.295) \\
            & \texttt{OneSampleMR}      & 0.302 (0.066) & 0.082 (0.009) & 0.011 (0.002) \\
            & \texttt{mrbayes}          & 0.302 (0.065) & 0.082 (0.009) & 0.011 (0.002) \\
\hline
n = 1000    & \texttt{MR.RGM}           & 0.031 (0.018) & 0.006 (0.001) & 0.0001 (0.00002) \\
            & \texttt{MR.RGM\_NoConf}   & 0.151 (0.026) & 0.035 (0.002) & 0.002 (0.0003) \\
            % & \texttt{GRIVET}        & 0.115 (0.020) & 0.023 (0.002) & 0.002 (0.0002) \\
            & \texttt{MR-SimpleMedian}  & 0.229 (0.034) & 0.066 (0.005) & 0.007 (0.001) \\
            & \texttt{MR-WeightedMedian}& 0.215 (0.025) & 0.063 (0.006) & 0.006 (0.001) \\
            & \texttt{MR-IVW}           & 0.194 (0.023) & 0.057 (0.006) & 0.005 (0.001) \\
            % & \texttt{MR-Egger}       & 7.465 (6.895) & 1.033 (0.380)  & 3.576 (5.254) \\
            % & \texttt{MR-Intercept}   & 7.288 (6.750) & 1.030 (0.368)  & 3.451 (4.990) \\
            & \texttt{OneSampleMR}      & 0.196 (0.022) & 0.058 (0.006) & 0.005 (0.001) \\
            & \texttt{mrbayes}          & 0.195 (0.022) & 0.058 (0.006) & 0.005 (0.001) \\
\hline
n = 10000   & \texttt{MR.RGM}           & 0.054 (0.007) & 0.012 (0.001) & 0.0003 (0.0001) \\
            & \texttt{MR.RGM\_NoConf}   & 0.105 (0.018) & 0.029 (0.003) & 0.002 (0.0002) \\
            % & \texttt{GRIVET}        & 0.090 (0.023) & 0.017 (0.006) & 0.001 (0.001) \\
            & \texttt{MR-SimpleMedian}  & 0.072 (0.008) & 0.022 (0.001) & 0.0007 (0.0001) \\
            & \texttt{MR-WeightedMedian}& 0.072 (0.008) & 0.021 (0.001) & 0.0007 (0.0001) \\
            & \texttt{MR-IVW}           & 0.062 (0.008) & 0.019 (0.001) & 0.0005 (0.0001) \\
            % & \texttt{MR-Egger}       & 5.717 (3.683) & 0.945 (0.265) & 2.180 (1.715) \\
            % & \texttt{MR-Intercept}   & 5.697 (3.648) & 0.943 (0.264) & 2.166 (1.704) \\
            & \texttt{OneSampleMR}      & 0.062 (0.008) & 0.018 (0.001) & 0.0005 (0.0001) \\
            & \texttt{mrbayes}          & 0.062 (0.008) & 0.018 (0.001) & 0.0005 (0.0001) \\
\hline
n = 30000   & \texttt{MR.RGM}           & 0.030 (0.018) & 0.006 (0.001) & 0.0001 (0.00002) \\
            & \texttt{MR.RGM\_NoConf}   & 0.096 (0.013) & 0.028 (0.003) & 0.001 (0.0001) \\
            % & \texttt{GRIVET}        & 0.087 (0.030) & 0.016 (0.007) & 0.001 (0.001) \\
            & \texttt{MR-SimpleMedian}  & 0.046 (0.007) & 0.012 (0.001) & 0.0003 (0.00004) \\
            & \texttt{MR-WeightedMedian}& 0.045 (0.007) & 0.012 (0.001) & 0.0002 (0.00004) \\
            & \texttt{MR-IVW}           & 0.039 (0.007) & 0.011 (0.001) & 0.0002 (0.00003) \\
            % & \texttt{MR-Egger}       & 8.006 (7.547) & 1.118 (0.483) & 5.048 (8.547) \\
            % & \texttt{MR-Intercept}   & 8.005 (7.592) & 1.119 (0.482) & 5.064 (8.651) \\
            & \texttt{OneSampleMR}      & 0.038 (0.005) & 0.011 (0.001) & 0.0002 (0.00003) \\
            & \texttt{mrbayes}          & 0.038 (0.005) & 0.011 (0.001) & 0.0002 (0.00003) \\
\hline
\end{tabular}
\end{table}

\begin{figure}[htb]
    \centering
    \includegraphics[width=.7\textwidth]{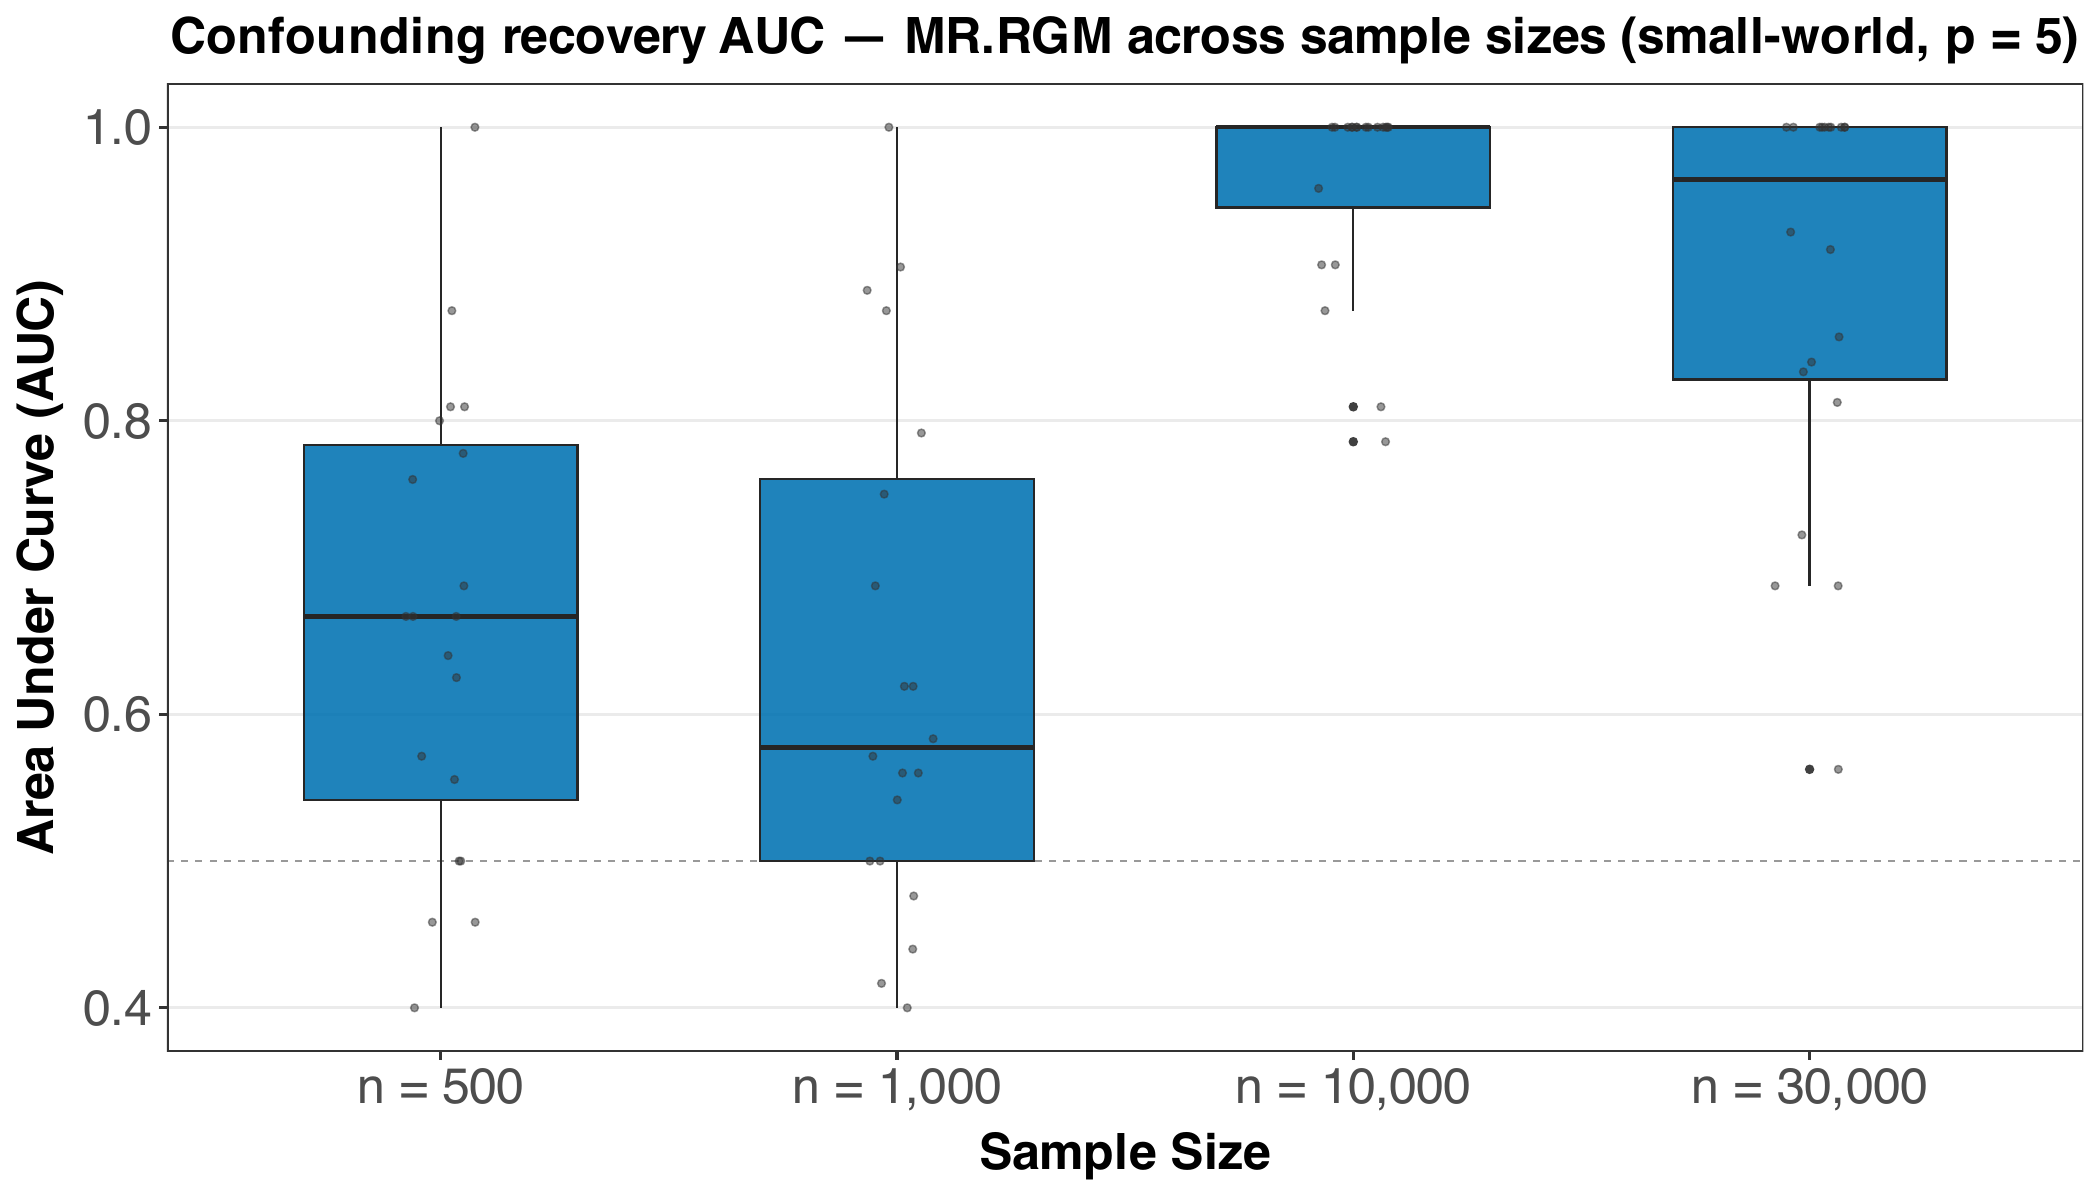}
    \caption{Confounding structure recovery performance using \texttt{MR.RGM} in a small-world network with
    feedback loops and unmeasured confounding, with network size \(p{=}5\). Boxplots of AUC across sample sizes (\(n \in \{500,1000,10000,30000\}\)).}
    \label{fig:sw_conf_p5}
\end{figure}

\begin{table}[htb]
\centering
\small
\caption{Confounding structure recovery performance using \texttt{MR.RGM} in a small-world network with feedback loops and unmeasured confounding, across network sizes \(p\in\{5,10\}\).}
\label{tab:feedback_conf_auc_smallworld_A}
\begin{tabular}{|c|c|c|c|c|c|}
\hline
\textbf{Setting} & \textbf{Sample Size} & \textbf{AUC} & \textbf{TPR} & \textbf{FDR} & \textbf{MCC} \\
\hline
% \hline
% \multirow{4}{*}{p = 5, Var = 97\%} 
%     & 500  & 0.677 & 0.479 & 0.741 & -0.202 \\
%     & 1000 & 0.667 & 0.560 & 0.724 & -0.178 \\
%     & 10000 & 0.744 & 0.497 & 0.665 & -0.020 \\
%     & 30000 & 0.807 & 0.617 & 0.648 & 0.060 \\
\hline
\multirow{4}{*}{p = 5} 
    & 500 & 0.661 (0.154) & 0.312 (0.290) & 0.363 (0.384) & 0.179 (0.369) \\
    & 1000 & 0.634 (0.173) & 0.480 (0.307) & 0.418 (0.300) & 0.216 (0.327) \\
    & 10000 & 0.962 (0.066) & 0.905 (0.148) & 0.321 (0.351) & 0.584 (0.290) \\
    & 30000 & 0.892 (0.133) & 0.990 (0.044) & 0.333 (0.354) & 0.651 (0.348) \\
% \hline
% \multirow{4}{*}{p = 10, Var = 97\%} 
%     & 500  & 0.597 & 0.354 & 0.638 & -0.129 \\
%     & 1000 & 0.576 & 0.375 & 0.659 & -0.181 \\
%     & 10000 & 0.684 & 0.394 & 0.605 & -0.053 \\
%     & 30000 & 0.835 & 0.562 & 0.558 & 0.078 \\
\hline
\multirow{4}{*}{p = 10} 
    & 500 & 0.687 (0.067) & 0.288 (0.083) & 0.262 (0.226) & 0.213 (0.135) \\
    & 1000 & 0.756 (0.067) & 0.402 (0.121) & 0.180 (0.191) & 0.349 (0.127) \\
    & 10000 & 0.983 (0.017) & 0.926 (0.068) & 0.152 (0.270) & 0.762 (0.219) \\
    & 30000 & 0.950 (0.102) & 0.998 (0.008) & 0.151 (0.289) & 0.847 (0.286) \\
\hline
\end{tabular}
\end{table}

\subsection{Case \texorpdfstring{$3$}{3}: Small-world network with feedback loops, unmeasured confounding, and horizontal pleiotropy}

\noindent\textit{Overview.} Figure (\ref{fig:swp_auc_p5}) reports graph-recovery AUC (boxplots) by method across sample sizes for network size $p=5$. Tables (\ref{tab:feedback_graph_structure_smallworld_horizontal_90_p=5}) and (\ref{tab:feedback_graph_structure_smallworld_horizontal_90_p=10}) summarize graph-recovery metrics (AUC, TPR, FDR, MCC; mean $\pm$ sd) for $p\in\{5,10\}$. Figure (\ref{fig:swp_mad_p5}) shows causal-effect estimation error (MeanAbsDev; boxplots) by method across sample sizes for $p=5$, while Tables (\ref{tab:feedback_causal_effect_smallworld_horizontal_90_p=5}) and (\ref{tab:feedback_causal_effect_smallworld_horizontal_horizontal_90_p=10}) report effect-estimation error metrics (MaxAbsDev, MeanAbsDev, MeanSqDev; mean $\pm$ sd) for $p\in\{5,10\}$. Figure (\ref{fig:swp_conf_p5}) presents confounding-structure recovery AUC (boxplots) across sample sizes for both \texttt{MR.RGM} and \texttt{MR.RGM+} at $p=5$, and Tables (\ref{tab:feedback_conf_auc_smallworld_horizontal_A}) and (\ref{tab:feedback_conf_auc_smallworld_horizontal_B}) compile confounding-structure recovery metrics (AUC, TPR, FDR, MCC; mean $\pm$ sd) for \texttt{MR.RGM} and \texttt{MR.RGM+} respectively at $p\in\{5,10\}$. Finally, Figure (\ref{fig:snp_auc_sw_p5}) displays instrument–trait selection AUC (boxplots) for \texttt{MR.RGM+} across sample sizes at $p=5$.

\begin{figure}[htb]
    \centering
    \includegraphics[width=.7\textwidth]{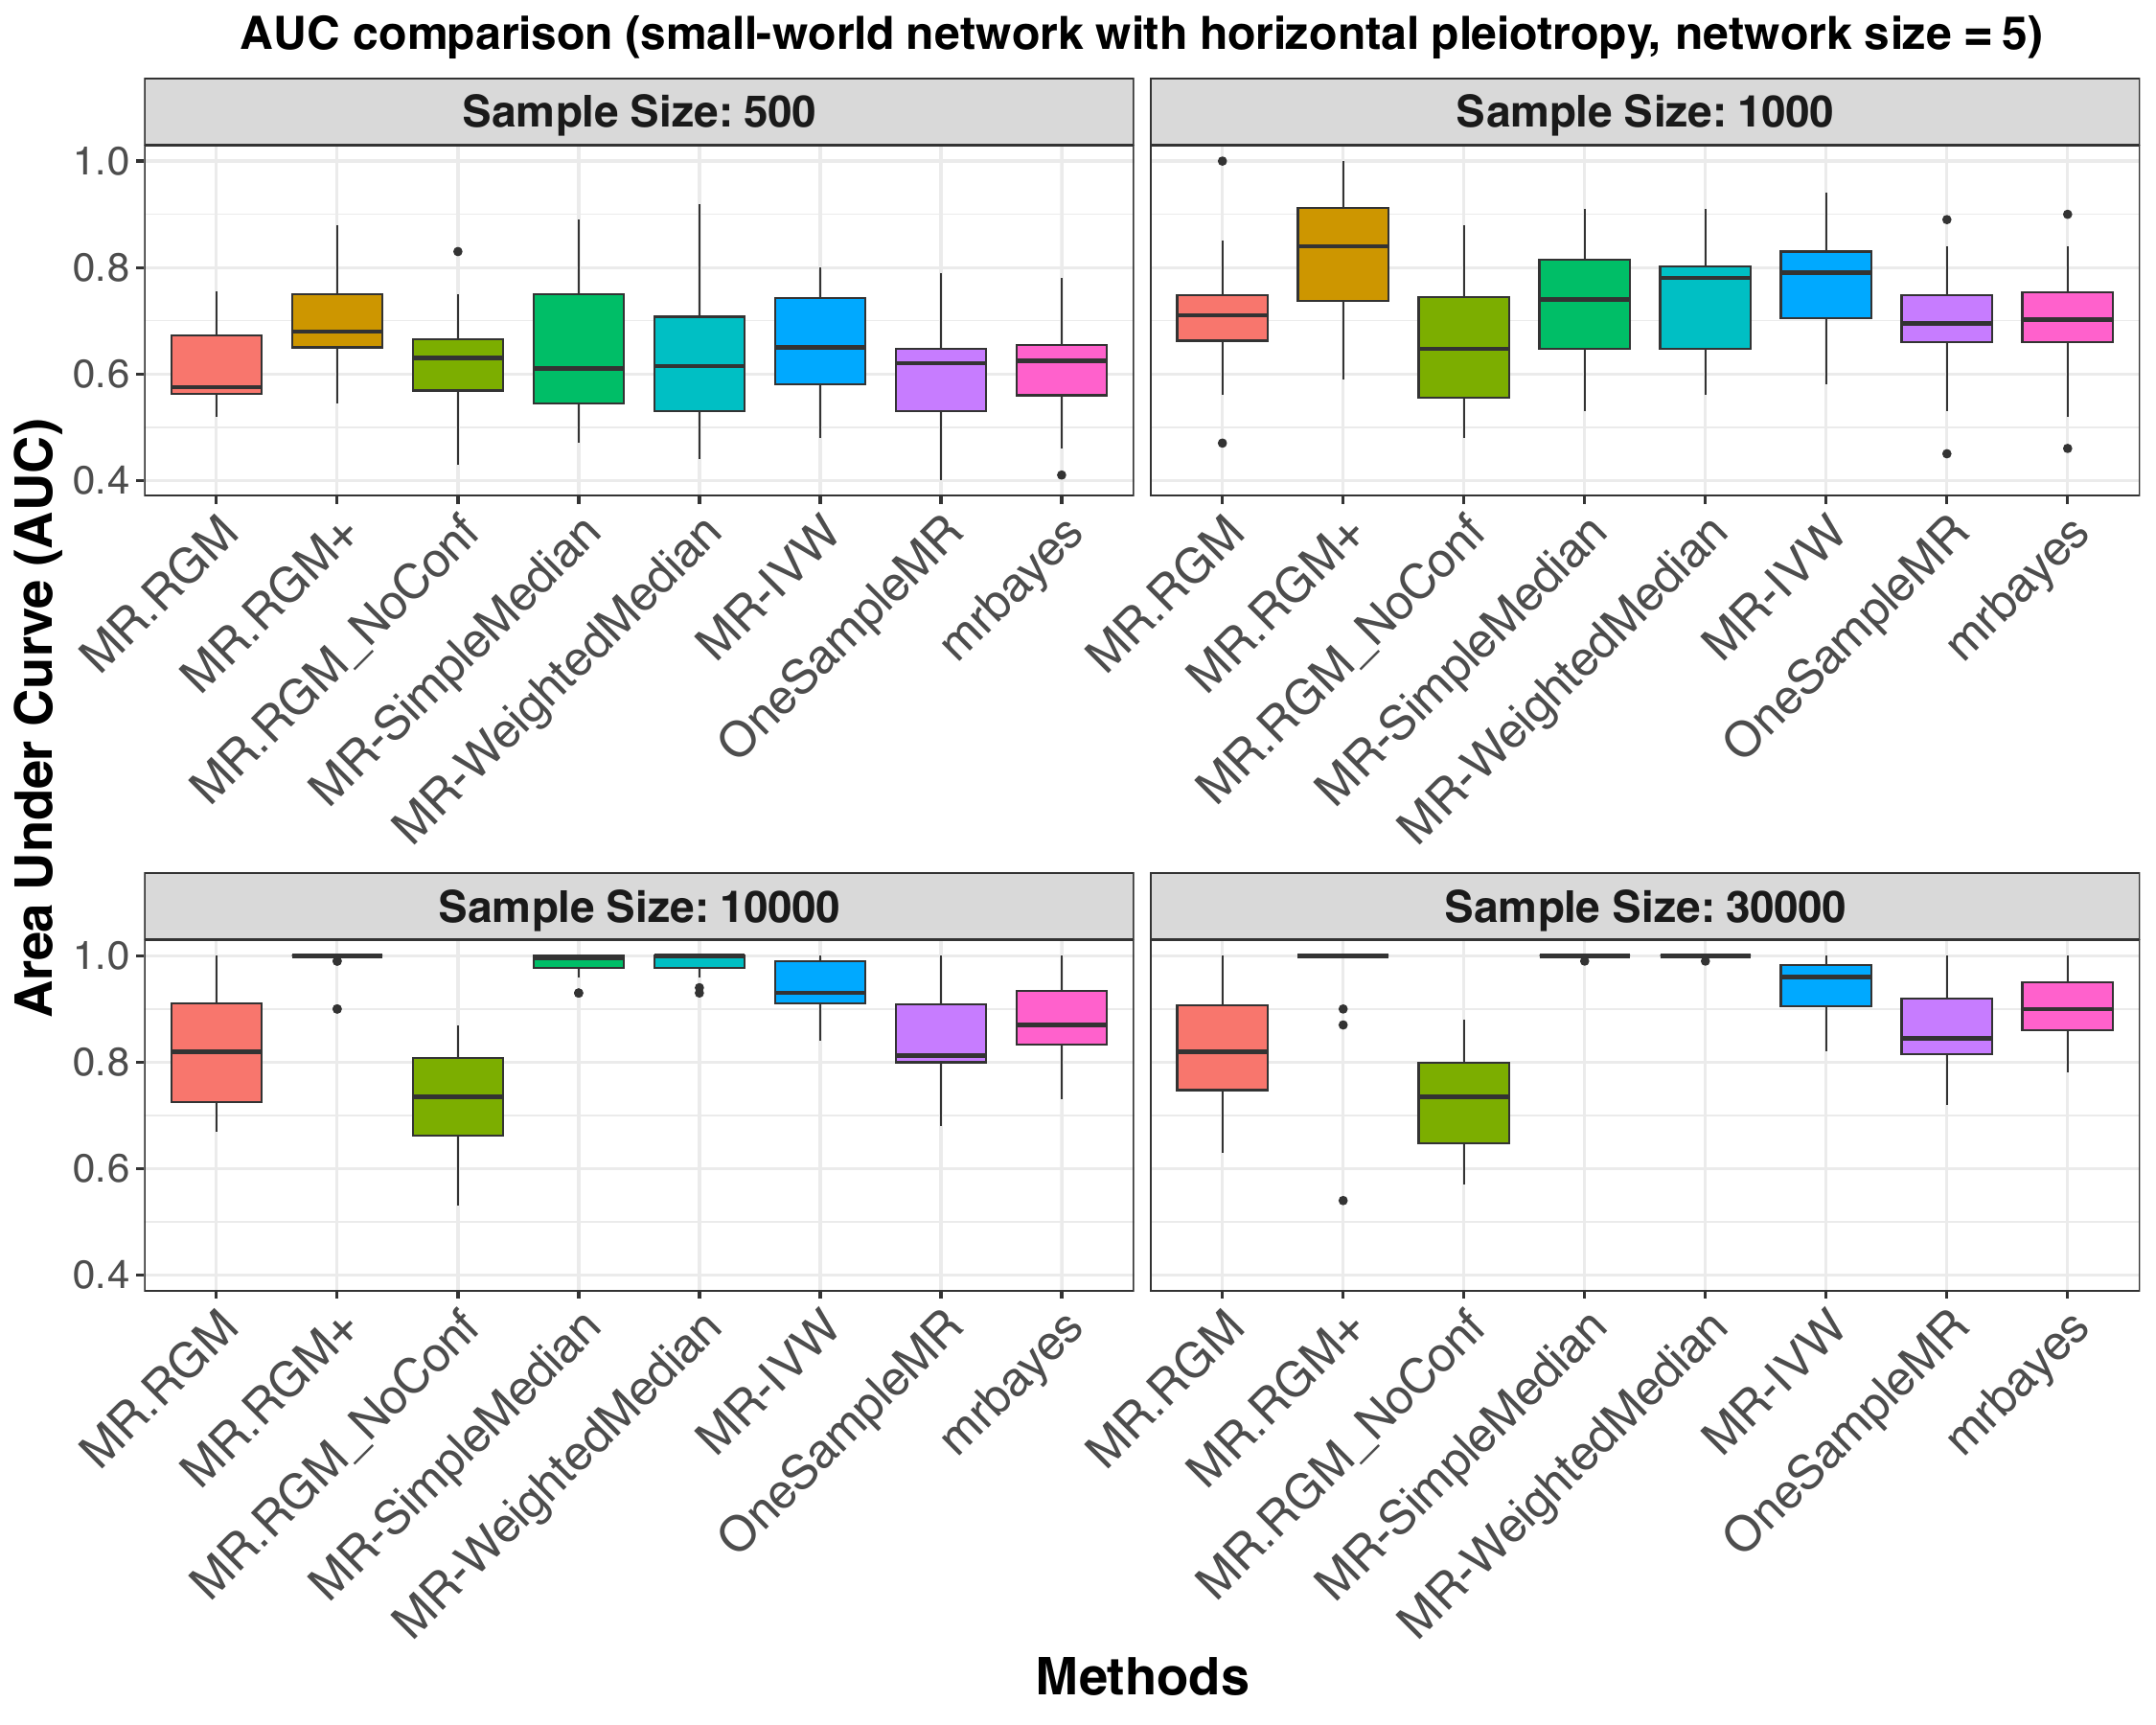}
    \caption{Graph recovery performance in a small-world network with feedback loops, unmeasured confounding, and horizontal pleiotropy, with network size \(p{=}5\). Boxplots of AUC by method (x-axis) and sample size (facets; \(n \in \{500,1000,10000,30000\}\)).}
    \label{fig:swp_auc_p5}
\end{figure}

\begin{table}[htb]
\centering
\tiny
\caption{Graph recovery performance in a small-world network with feedback loops, unmeasured confounding, and horizontal pleiotropy, with network size \(p{=}5\).}
\label{tab:feedback_graph_structure_smallworld_horizontal_90_p=5}
\begin{tabular}{|c|c|c|c|c|c|}
\hline
\textbf{Setting} & \textbf{Method} & \textbf{AUC} & \textbf{TPR} & \textbf{FDR} & \textbf{MCC} \\
\hline
% \multicolumn{6}{|c|}{\textbf{p = 5, Variance Explained = 90\%}} \\
\hline
n = 500     & \texttt{MR.RGM}           & 0.614 (0.072) & 0.483 (0.126) & 0.374 (0.134) & 0.192 (0.212) \\
            & \texttt{MR.RGM+}          & 0.697 (0.083) & 0.483 (0.146) & 0.256 (0.093) & 0.344 (0.160) \\
            & \texttt{MR.RGM\_NoConf}   & 0.621 (0.095) & 0.536 (0.123) & 0.392 (0.103) & 0.177 (0.181) \\
            % & \texttt{MR.RGM(Full D \& No Conf.)}  & 0.671 (0.085) & 0.543 (0.184) & 0.285 (0.136) & 0.327 (0.157) \\
            % & \texttt{GRIVET}         & 0.500 (0.000) & 0.000 (0.000) & 0.000 (0.000) & 0.000 (0.000) \\
            & \texttt{MR-SimpleMedian}  & 0.642 (0.120) & 0.080 (0.081) & 0.067 (0.226) & 0.131 (0.156) \\
            & \texttt{MR-WeightedMedian}& 0.629 (0.123) & 0.105 (0.074) & 0.117 (0.211) & 0.142 (0.144) \\
            & \texttt{MR-IVW}           & 0.650 (0.094) & 0.180 (0.087) & 0.163 (0.239) & 0.214 (0.179) \\
            % & \texttt{MR-Egger}       & 0.623 (0.086) & 0.065 (0.079) & 0.433 (0.429) & -0.023 (0.226) \\
            % & \texttt{MR-Intercept}   & 0.603 (0.083) & 0.065 (0.079) & 0.442 (0.432) & -0.035 (0.233) \\
            & \texttt{OneSampleMR}      & 0.595 (0.106) & 0.244 (0.112) & 0.410 (0.230) & 0.103 (0.215) \\
            & \texttt{mrbayes}          & 0.606 (0.094) & 0.244 (0.096) & 0.422 (0.165) & 0.085 (0.171) \\
\hline
n = 1000    & \texttt{MR.RGM}           & 0.714 (0.113) & 0.594 (0.122) & 0.286 (0.123) & 0.358 (0.196) \\
            & \texttt{MR.RGM+}          & 0.817 (0.114) & 0.528 (0.182) & 0.135 (0.140) & 0.481 (0.200) \\
            & \texttt{MR.RGM\_NoConf}   & 0.661 (0.117) & 0.663 (0.154) & 0.341 (0.099) & 0.319 (0.203) \\
            % & \texttt{MR.RGM(Full D $\&$ No Conf.)} & 0.714 (0.129) & 0.681 (0.181) & 0.291 (0.134) & 0.392 (0.234) \\
            % & \texttt{GRIVET}         & 0.500 (0.000) & 0.000 (0.000) & 0.000 (0.000) & 0.000 (0.000) \\
            & \texttt{MR-SimpleMedian}  & 0.738 (0.110) & 0.200 (0.138) & 0.070 (0.156) & 0.267 (0.159) \\
            & \texttt{MR-WeightedMedian}& 0.745 (0.109) & 0.235 (0.128) & 0.090 (0.158) & 0.293 (0.139) \\
            & \texttt{MR-IVW}           & 0.764 (0.097) & 0.275 (0.148) & 0.130 (0.231) & 0.312 (0.157) \\
            % & \texttt{MR-Egger}       & 0.600 (0.100) & 0.025 (0.054) & 0.550 (0.475) & -0.102 (0.170) \\
            % & \texttt{MR-Intercept}   & 0.591 (0.092) & 0.025 (0.054) & 0.554 (0.449) & -0.119 (0.139) \\
            & \texttt{OneSampleMR}      & 0.690 (0.102) & 0.394 (0.108) & 0.325 (0.099) & 0.222 (0.124) \\
            & \texttt{mrbayes}          & 0.690 (0.105) & 0.411 (0.124) & 0.323 (0.092) & 0.232 (0.124) \\
\hline
n = 10000   & \texttt{MR.RGM}           & 0.826 (0.099) & 0.939 (0.068) & 0.173 (0.078) & 0.746 (0.123) \\
            & \texttt{MR.RGM+}          & 0.988 (0.031) & 0.928 (0.087) & 0.006 (0.023) & 0.927 (0.084) \\
            & \texttt{MR.RGM\_NoConf}   & 0.730 (0.094) & 0.828 (0.115) & 0.336 (0.076) & 0.420 (0.189) \\
            % & \texttt{MR.RGM(Full D $\&$ No Conf.)} & 0.817 (0.113) & 0.778 (0.136) & 0.214 (0.108) & 0.551 (0.183) \\
            % & \texttt{GRIVET}         & 0.500 (0.000) & 0.000 (0.000) & 0.000 (0.000) & 0.000 (0.000) \\
            & \texttt{MR-SimpleMedian}  & 0.985 (0.022) & 0.935 (0.073) & 0.064 (0.080) & 0.869 (0.129) \\
            & \texttt{MR-WeightedMedian}& 0.986 (0.021) & 0.955 (0.067) & 0.063 (0.068) & 0.889 (0.103) \\
            & \texttt{MR-IVW}           & 0.943 (0.046) & 0.825 (0.099) & 0.069 (0.075) & 0.770 (0.127) \\
            % & \texttt{MR-Egger}       & 0.604 (0.100) & 0.075 (0.099) & 0.503 (0.437) & -0.060 (0.254) \\
            % & \texttt{MR-Intercept}   & 0.607 (0.097) & 0.075 (0.099) & 0.503 (0.437) & -0.065 (0.259) \\
            & \texttt{OneSampleMR}      & 0.831 (0.090) & 0.983 (0.037) & 0.191 (0.078) & 0.764 (0.098) \\
            & \texttt{mrbayes}          & 0.867 (0.071) & 0.978 (0.042) & 0.193 (0.072) & 0.757 (0.093) \\
\hline
n = 30000   & \texttt{MR.RGM}           & 0.823 (0.097) & 0.983 (0.037) & 0.152 (0.075) & 0.814 (0.113) \\
            & \texttt{MR.RGM+}          & 0.962 (0.109) & 0.989 (0.031) & 0.042 (0.080) & 0.942 (0.115) \\
            & \texttt{MR.RGM\_NoConf}   & 0.729 (0.091) & 0.867 (0.094) & 0.332 (0.066) & 0.458 (0.169) \\
            % & \texttt{MR.RGM(Full D $\&$ No Conf.)} & 0.771 (0.120) & 0.817 (0.112) & 0.244 (0.124) & 0.534 (0.153) \\
            % & \texttt{GRIVET}         & 0.500 (0.000) & 0.000 (0.000) & 0.000 (0.000) & 0.000 (0.000) \\
            & \texttt{MR-SimpleMedian}  & 0.999 (0.002) & 1.000 (0.000) & 0.062 (0.055) & 0.934 (0.060) \\
            & \texttt{MR-WeightedMedian}& 0.999 (0.002) & 1.000 (0.000) & 0.066 (0.060) & 0.930 (0.065) \\
            & \texttt{MR-IVW}           & 0.943 (0.052) & 0.840 (0.102) & 0.097 (0.087) & 0.752 (0.148) \\
            % & \texttt{MR-Egger}       & 0.635 (0.083) & 0.145 (0.092) & 0.551 (0.302) & -0.064 (0.227) \\
            % & \texttt{MR-Intercept}   & 0.631 (0.074) & 0.120 (0.081) & 0.583 (0.312) & -0.102 (0.213) \\
            & \texttt{OneSampleMR}      & 0.856 (0.081) & 1.000 (0.000) & 0.245 (0.079) & 0.705 (0.114) \\
            & \texttt{mrbayes}          & 0.906 (0.054) & 1.000 (0.000) & 0.247 (0.081) & 0.701 (0.117) \\
\hline
\end{tabular}
\end{table}

\begin{table}[htb]
\centering
\tiny
\caption{Graph recovery performance in a small-world network with feedback loops, unmeasured confounding, and horizontal pleiotropy, with network size \(p{=}10\).}
\label{tab:feedback_graph_structure_smallworld_horizontal_90_p=10}
\begin{tabular}{|c|c|c|c|c|c|}
\hline
\textbf{Setting} & \textbf{Method} & \textbf{AUC} & \textbf{TPR} & \textbf{FDR} & \textbf{MCC} \\
\hline
% \multicolumn{6}{|c|}{\textbf{p = 10, Variance Explained = 90\%}} \\
\hline
n = 500     & \texttt{MR.RGM}           & 0.720 (0.067) & 0.511 (0.101) & 0.553 (0.065) & 0.315 (0.090) \\
            & \texttt{MR.RGM+}          & 0.744 (0.067) & 0.514 (0.085) & 0.525 (0.047) & 0.342 (0.066) \\
            & \texttt{MR.RGM\_NoConf}   & 0.722 (0.075) & 0.563 (0.104) & 0.604 (0.061) & 0.283 (0.095) \\
            % & \texttt{GRIVET}         & 0.500 (0.000) & 0.000 (0.000) & 0.000 (0.000) & 0.000 (0.000) \\
            & \texttt{MR-SimpleMedian}  & 0.606 (0.067) & 0.095 (0.059) & 0.408 (0.293) & 0.144 (0.105) \\
            & \texttt{MR-WeightedMedian}& 0.613 (0.072) & 0.115 (0.059) & 0.480 (0.256) & 0.157 (0.110) \\
            & \texttt{MR-IVW}           & 0.626 (0.087) & 0.150 (0.082) & 0.516 (0.240) & 0.174 (0.148) \\
            % & \texttt{MR-Egger}       & 0.566 (0.052) & 0.058 (0.040) & 0.740 (0.175) & 0.024 (0.080) \\
            % & \texttt{MR-Intercept}   & 0.553 (0.055) & 0.048 (0.049) & 0.808 (0.192) & -0.004 (0.094) \\
            & \texttt{OneSampleMR}      & 0.627 (0.077) & 0.211 (0.081) & 0.575 (0.116) & 0.171 (0.100) \\
            & \texttt{mrbayes}          & 0.627 (0.078) & 0.211 (0.070) & 0.583 (0.116) & 0.164 (0.093) \\
\hline
n = 1000    & \texttt{MR.RGM}           & 0.797 (0.052) & 0.603 (0.127) & 0.449 (0.122) & 0.444 (0.140) \\
            & \texttt{MR.RGM+}          & 0.811 (0.062) & 0.567 (0.122) & 0.411 (0.099) & 0.458 (0.112) \\
            & \texttt{MR.RGM\_NoConf}   & 0.762 (0.043) & 0.686 (0.095) & 0.556 (0.029) & 0.387 (0.060) \\
            % & \texttt{GRIVET}         & 0.500 (0.000) & 0.000 (0.000) & 0.000 (0.000) & 0.000 (0.000) \\
            & \texttt{MR-SimpleMedian}  & 0.706 (0.071) & 0.200 (0.094) & 0.368 (0.228) & 0.264 (0.140) \\
            & \texttt{MR-WeightedMedian}& 0.694 (0.094) & 0.220 (0.094) & 0.327 (0.200) & 0.294 (0.120) \\
            & \texttt{MR-IVW}           & 0.734 (0.062) & 0.275 (0.097) & 0.352 (0.161) & 0.326 (0.122) \\
            % & \texttt{MR-Egger}       & 0.560 (0.041) & 0.068 (0.060) & 0.728 (0.225) & 0.036 (0.114) \\
            % & \texttt{MR-Intercept}   & 0.560 (0.052) & 0.058 (0.060) & 0.774 (0.184) & 0.012 (0.101) \\
            & \texttt{OneSampleMR}      & 0.736 (0.061) & 0.375 (0.124) & 0.448 (0.150) & 0.333 (0.151) \\
            & \texttt{mrbayes}          & 0.736 (0.062) & 0.383 (0.113) & 0.453 (0.137) & 0.333 (0.139) \\
\hline
n = 10000   & \texttt{MR.RGM}           & 0.951 (0.029) & 0.969 (0.041) & 0.161 (0.067) & 0.871 (0.060) \\
            & \texttt{MR.RGM+}          & 0.985 (0.027) & 0.958 (0.034) & 0.061 (0.088) & 0.932 (0.067) \\
            & \texttt{MR.RGM\_NoConf}   & 0.855 (0.027) & 0.850 (0.061) & 0.506 (0.054) & 0.512 (0.070) \\
            % & \texttt{GRIVET}         & 0.500 (0.000) & 0.000 (0.000) & 0.000 (0.000) & 0.000 (0.000) \\
            & \texttt{MR-SimpleMedian}  & 0.992 (0.013) & 0.970 (0.058) & 0.145 (0.053) & 0.883 (0.056) \\
            & \texttt{MR-WeightedMedian}& 0.993 (0.010) & 0.975 (0.056) & 0.147 (0.054) & 0.884 (0.055) \\
            & \texttt{MR-IVW}           & 0.958 (0.032) & 0.875 (0.086) & 0.167 (0.072) & 0.810 (0.084) \\
            % & \texttt{MR-Egger}       & 0.556 (0.052) & 0.040 (0.046) & 0.832 (0.223) & -0.061 (0.077) \\
            % & \texttt{MR-Intercept}   & 0.556 (0.044) & 0.040 (0.037) & 0.824 (0.218) & -0.057 (0.068) \\
            & \texttt{OneSampleMR}      & 0.956 (0.020) & 0.994 (0.016) & 0.283 (0.065) & 0.793 (0.051) \\
            & \texttt{mrbayes}          & 0.968 (0.014) & 0.994 (0.016) & 0.276 (0.062) & 0.798 (0.049) \\
\hline
n = 30000   & \texttt{MR.RGM}           & 0.950 (0.026) & 0.992 (0.019) & 0.139 (0.068) & 0.900 (0.050) \\
            & \texttt{MR.RGM+}          & 0.987 (0.023) & 0.989 (0.021) & 0.029 (0.075) & 0.973 (0.061) \\
            & \texttt{MR.RGM\_NoConf}   & 0.869 (0.025) & 0.895 (0.042) & 0.530 (0.029) & 0.510 (0.039) \\
            % & \texttt{GRIVET}         & 0.856 (0.048) & 0.875 (0.040) & 0.472 (0.060) & 0.559 (0.079) \\
            % & \texttt{GRIVET}         & 0.500 (0.000) & 0.000 (0.000) & 0.000 (0.000) & 0.000 (0.000) \\
            & \texttt{MR-SimpleMedian}  & 0.999 (0.0003) & 1.000 (0.000) & 0.170 (0.065) & 0.883 (0.048) \\
            & \texttt{MR-WeightedMedian}& 0.999 (0.0003) & 1.000 (0.000) & 0.172 (0.066) & 0.882 (0.049) \\
            & \texttt{MR-IVW}           & 0.960 (0.032) & 0.893 (0.071) & 0.196 (0.058) & 0.800 (0.057) \\
            % & \texttt{MR-Egger}       & 0.535 (0.048) & 0.108 (0.064) & 0.803 (0.107) & -0.014 (0.081) \\
            % & \texttt{MR-Intercept}   & 0.533 (0.047) & 0.110 (0.064) & 0.799 (0.109) & -0.010 (0.082) \\
            & \texttt{OneSampleMR}      & 0.966 (0.016) & 1.000 (0.000) & 0.336 (0.066) & 0.752 (0.055) \\
            & \texttt{mrbayes}          & 0.977 (0.010) & 1.000 (0.000) & 0.335 (0.065) & 0.753 (0.054) \\
\hline
\end{tabular}
\end{table}

\begin{figure}[htb]
    \centering
    \includegraphics[width=.7\textwidth]{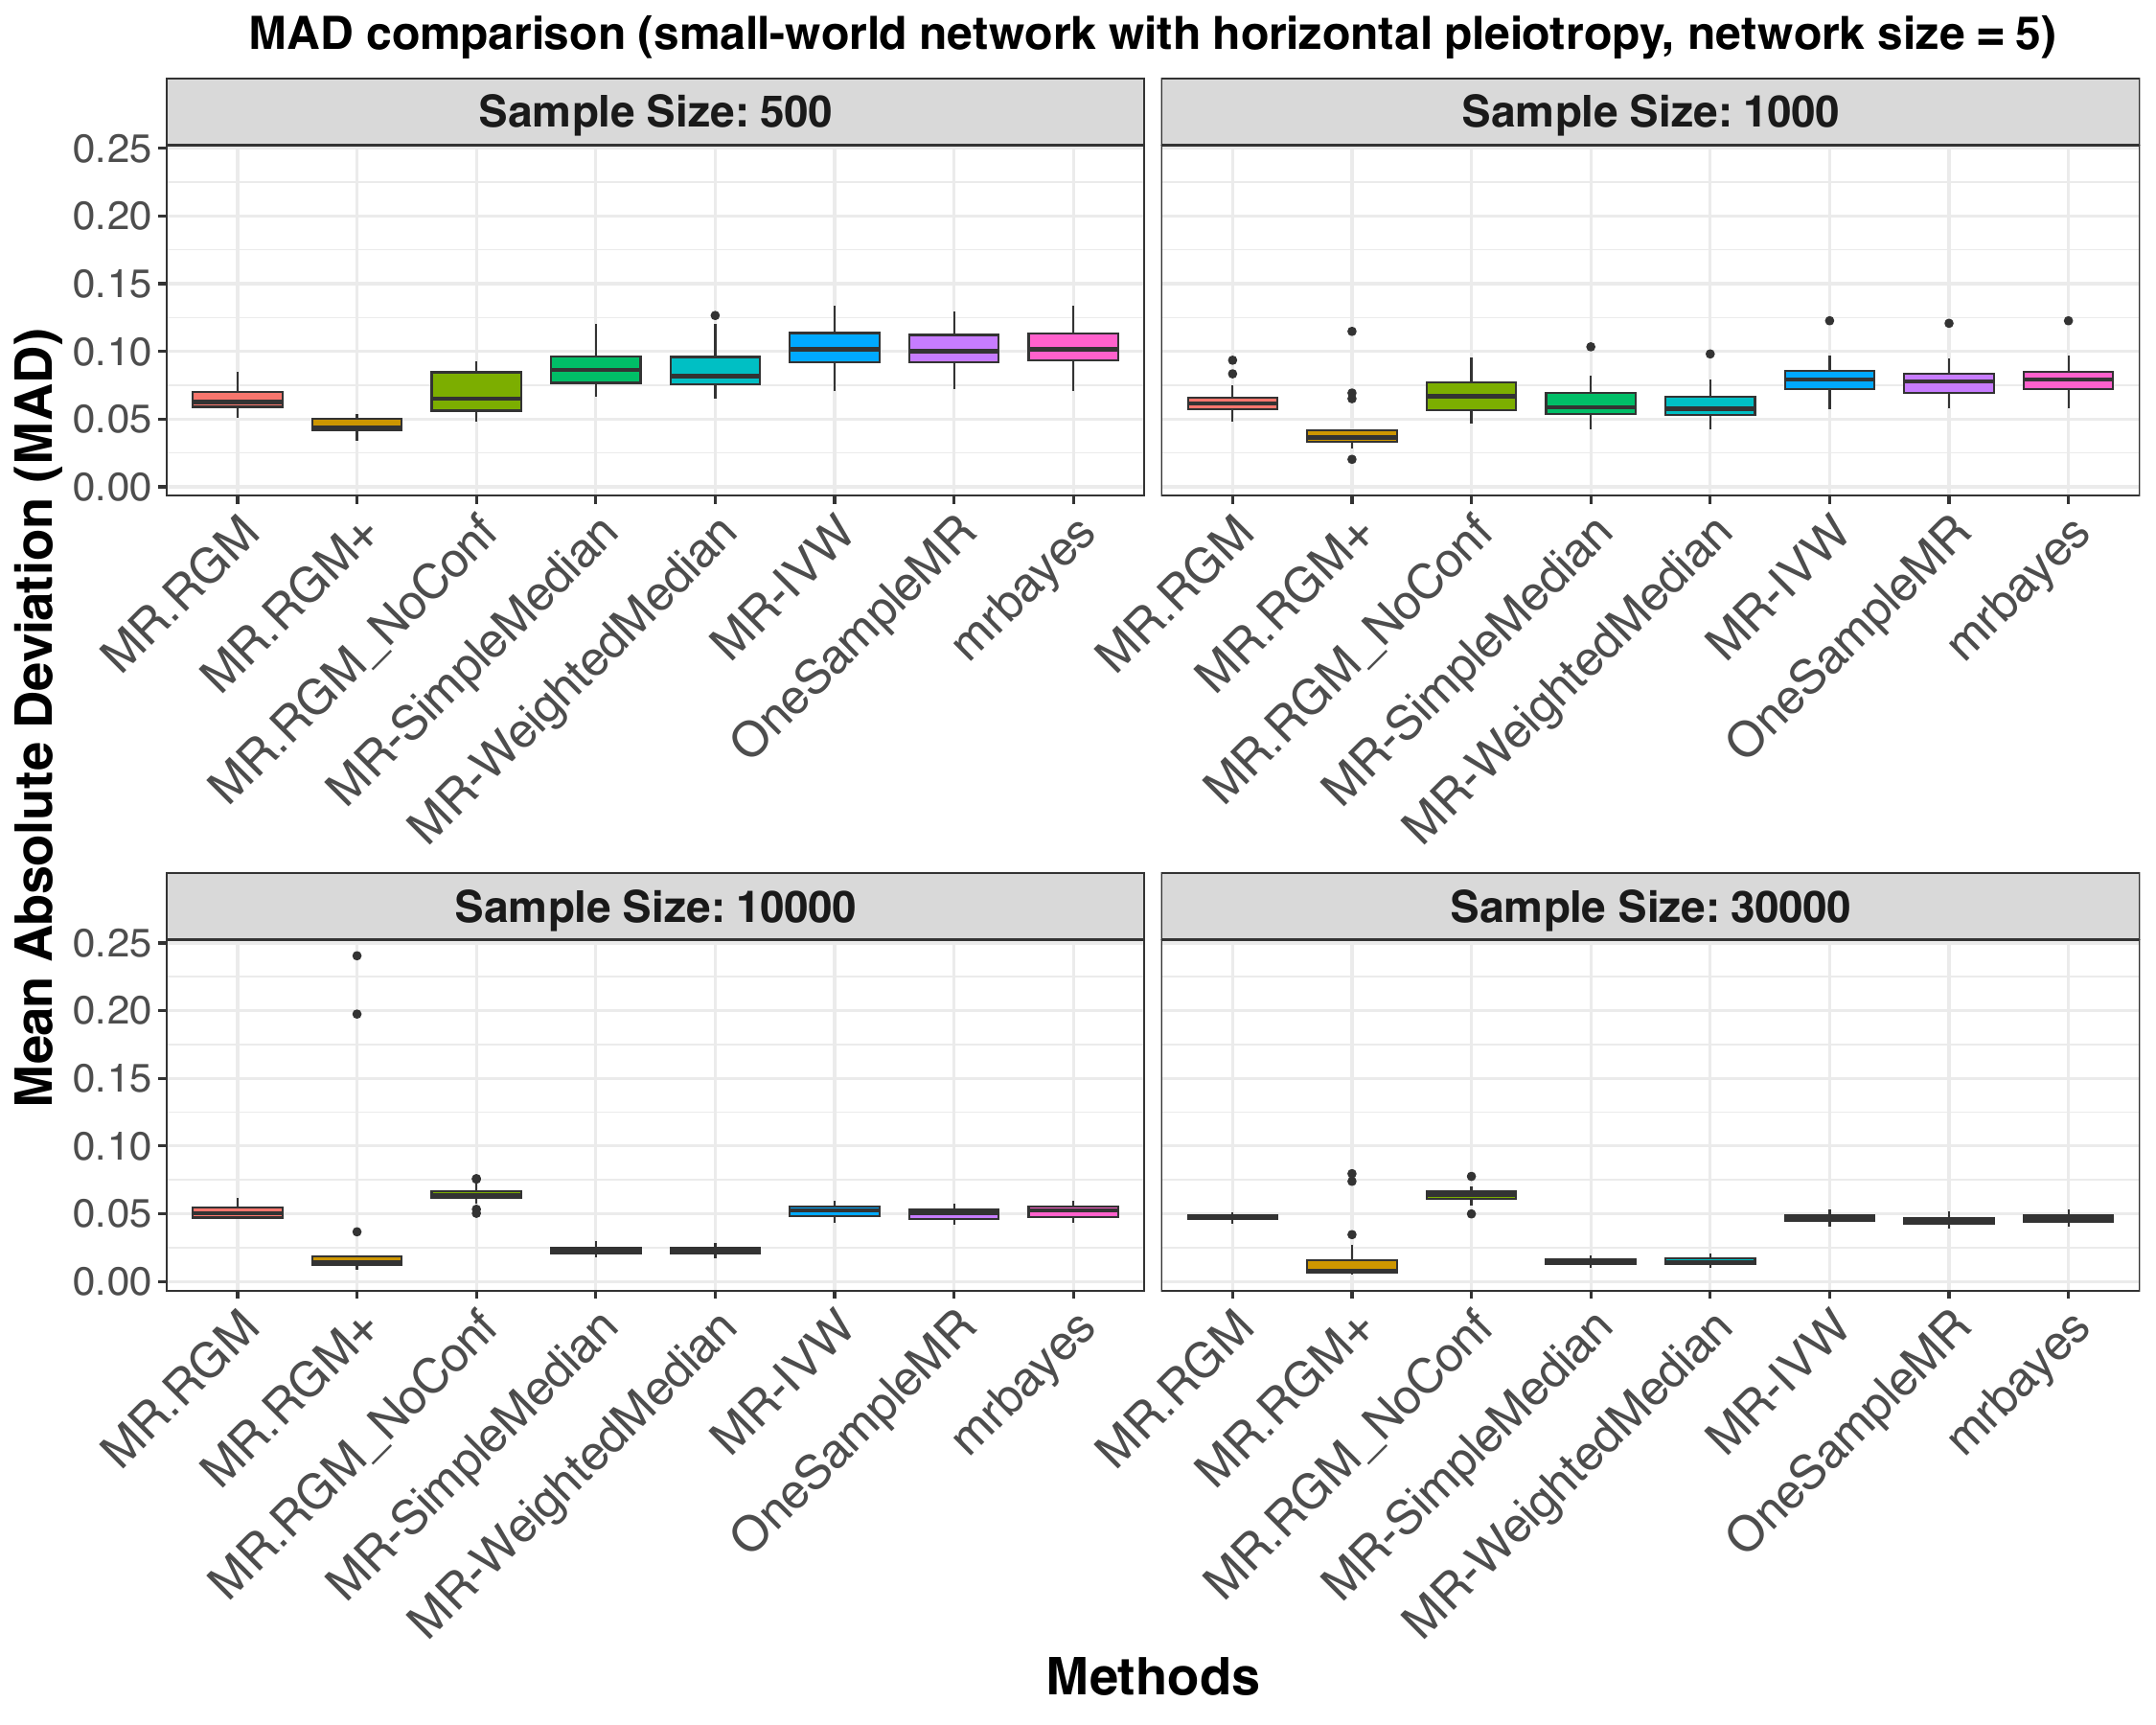}
    \caption{Causal effect estimation performance in a small-world network with feedback loops, unmeasured confounding, and horizontal pleiotropy, with network size \(p{=}5\). Boxplots of mean absolute deviation (MAD) by method (x-axis) and sample size (facets; \(n \in \{500,1000,10000,30000\}\)).}
    \label{fig:swp_mad_p5}
\end{figure}

\begin{table}[htb]
\centering
\tiny
\caption{Causal effect estimation performance in a small-world network with feedback loops, unmeasured confounding, and horizontal pleiotropy, with network size \(p{=}5\).}
\label{tab:feedback_causal_effect_smallworld_horizontal_90_p=5}
\begin{tabular}{|c|c|c|c|c|}
\hline
\textbf{Setting} & \textbf{Method} & \textbf{MaxAbsDev} & \textbf{MeanAbsDev} & \textbf{MeanSqDev} \\
\hline
% \multicolumn{5}{|c|}{\textbf{p = 5, Variance Explained = 90\%}} \\
\hline
n = 500     & \texttt{MR.RGM}         & 0.232 (0.076) & 0.065 (0.008) & 0.008 (0.003) \\
            & \texttt{MR.RGM+}        & 0.129 (0.044) & 0.045 (0.005) & 0.003 (0.001) \\
            & \texttt{MR.RGM\_NoConf} & 0.231 (0.082) & 0.070 (0.015) & 0.009 (0.004) \\
            % & \texttt{GRIVET} & 0.129 (0.034) & 0.043 (0.008) & 0.004 (0.001) \\
            & \texttt{MR-SimpleMedian}   & 0.247 (0.051) & 0.089 (0.016) & 0.013 (0.004) \\
            & \texttt{MR-WeightedMedian} & 0.228 (0.057) & 0.087 (0.017) & 0.012 (0.005) \\
            & \texttt{MR-IVW}            & 0.310 (0.065) & 0.101 (0.017) & 0.017 (0.005) \\
            & \texttt{OneSampleMR}       & 0.298 (0.053) & 0.100 (0.016) & 0.016 (0.005) \\
            & \texttt{mrbayes}           & 0.316 (0.062) & 0.102 (0.017) & 0.017 (0.005) \\
\hline
n = 1000    & \texttt{MR.RGM}         & 0.276 (0.057) & 0.063 (0.011) & 0.009 (0.003) \\
            & \texttt{MR.RGM+}        & 0.179 (0.207) & 0.043 (0.021) & 0.007 (0.016) \\
            & \texttt{MR.RGM\_NoConf} & 0.214 (0.051) & 0.068 (0.014) & 0.009 (0.004) \\
            % & \texttt{GRIVET} & 0.115 (0.050) & 0.038 (0.011) & 0.004 (0.002) \\
            & \texttt{MR-SimpleMedian}   & 0.183 (0.067) & 0.062 (0.014) & 0.007 (0.003) \\
            & \texttt{MR-WeightedMedian} & 0.188 (0.069) & 0.061 (0.013) & 0.006 (0.003) \\
            & \texttt{MR-IVW}            & 0.292 (0.069) & 0.081 (0.014) & 0.013 (0.005) \\
            & \texttt{OneSampleMR}       & 0.279 (0.058) & 0.079 (0.014) & 0.012 (0.004) \\
            & \texttt{mrbayes}           & 0.292 (0.063) & 0.081 (0.014) & 0.013 (0.005) \\
\hline
n = 10000   & \texttt{MR.RGM}         & 0.305 (0.039) & 0.051 (0.004) & 0.010 (0.001) \\
            & \texttt{MR.RGM+}        & 0.306 (0.665) & 0.038 (0.065) & 0.040 (0.111) \\
            & \texttt{MR.RGM\_NoConf} & 0.209 (0.027) & 0.064 (0.007) & 0.008 (0.001) \\
            % & \texttt{GRIVET} & 0.091 (0.021) & 0.032 (0.014) & 0.003 (0.002) \\
            & \texttt{MR-SimpleMedian}   & 0.065 (0.015) & 0.023 (0.003) & 0.001 (0.0003) \\
            & \texttt{MR-WeightedMedian} & 0.065 (0.013) & 0.023 (0.003) & 0.001 (0.0002) \\
            & \texttt{MR-IVW}            & 0.268 (0.019) & 0.052 (0.005) & 0.009 (0.001) \\
            & \texttt{OneSampleMR}       & 0.256 (0.018) & 0.050 (0.005) & 0.008 (0.001) \\
            & \texttt{mrbayes}           & 0.269 (0.019) & 0.052 (0.005) & 0.009 (0.001) \\
\hline
n = 30000   & \texttt{MR.RGM}         & 0.300 (0.023) & 0.047 (0.002) & 0.010 (0.001) \\
            & \texttt{MR.RGM+}        & 0.164 (0.253) & 0.018 (0.022) & 0.006 (0.014) \\
            & \texttt{MR.RGM\_NoConf} & 0.206 (0.028) & 0.064 (0.006) & 0.008 (0.001) \\
            % & \texttt{GRIVET} & 0.089 (0.026) & 0.031 (0.015) & 0.003 (0.002) \\
            & \texttt{MR-SimpleMedian}   & 0.044 (0.009) & 0.015 (0.003) & 0.0004 (0.0001) \\
            & \texttt{MR-WeightedMedian} & 0.044 (0.009) & 0.015 (0.003) & 0.0004 (0.0001) \\
            & \texttt{MR-IVW}            & 0.264 (0.018) & 0.047 (0.003) & 0.008 (0.0008) \\
            & \texttt{OneSampleMR}       & 0.251 (0.017) & 0.045 (0.003) & 0.008 (0.001) \\
            & \texttt{mrbayes}           & 0.263 (0.018) & 0.047 (0.003) & 0.008 (0.001) \\
\hline
\end{tabular}
\end{table}

\begin{table}[htb]
\centering
\tiny
\caption{Causal effect estimation performance in a small-world network with feedback loops, unmeasured confounding, and horizontal pleiotropy, with network size \(p{=}10\).}
\label{tab:feedback_causal_effect_smallworld_horizontal_horizontal_90_p=10}
\begin{tabular}{|c|c|c|c|c|}
\hline
\textbf{Setting} & \textbf{Method} & \textbf{MaxAbsDev} & \textbf{MeanAbsDev} & \textbf{MeanSqDev} \\
\hline
% \multicolumn{5}{|c|}{\textbf{p = 10, Variance Explained = 90\%}} \\
\hline
n = 500     & \texttt{MR.RGM}         & 0.317 (0.063) & 0.045 (0.005) & 0.005 (0.001) \\
            & \texttt{MR.RGM+}        & 0.201 (0.197) & 0.037 (0.005) & 0.003 (0.004) \\
            & \texttt{MR.RGM\_NoConf} & 0.273 (0.062) & 0.049 (0.005) & 0.005 (0.001) \\
            % & \texttt{GRIVET} & 0.149 (0.040) & 0.024 (0.004) & 0.002 (0.0004) \\
            & \texttt{MR-SimpleMedian}   & 0.293 (0.037) & 0.088 (0.006) & 0.012 (0.002) \\
            & \texttt{MR-WeightedMedian} & 0.293 (0.034) & 0.088 (0.006) & 0.012 (0.002) \\
            & \texttt{MR-IVW}            & 0.388 (0.057) & 0.087 (0.007) & 0.013 (0.002) \\
            & \texttt{OneSampleMR}       & 0.367 (0.044) & 0.087 (0.006) & 0.013 (0.002) \\
            & \texttt{mrbayes}           & 0.383 (0.051) & 0.088 (0.007) & 0.013 (0.002) \\
\hline
n = 1000    & \texttt{MR.RGM}         & 0.315 (0.047) & 0.042 (0.003) & 0.005 (0.001) \\
            & \texttt{MR.RGM+}        & 0.285 (0.367) & 0.035 (0.013) & 0.007 (0.013) \\
            & \texttt{MR.RGM\_NoConf} & 0.219 (0.030) & 0.045 (0.003) & 0.004 (0.001) \\
            % & \texttt{GRIVET} & 0.136 (0.036) & 0.022 (0.003) & 0.002 (0.0003) \\
            & \texttt{MR-SimpleMedian}   & 0.222 (0.034) & 0.064 (0.006) & 0.007 (0.001) \\
            & \texttt{MR-WeightedMedian} & 0.209 (0.032) & 0.063 (0.006) & 0.006 (0.001) \\
            & \texttt{MR-IVW}            & 0.332 (0.040) & 0.066 (0.005) & 0.008 (0.001) \\
            & \texttt{OneSampleMR}       & 0.316 (0.042) & 0.066 (0.005) & 0.008 (0.001) \\
            & \texttt{mrbayes}           & 0.334 (0.041) & 0.067 (0.005) & 0.008 (0.001) \\
\hline
n = 10000   & \texttt{MR.RGM}         & 0.321 (0.019) & 0.028 (0.002) & 0.005 (0.0004) \\
            & \texttt{MR.RGM+}        & 0.531 (0.806) & 0.023 (0.021) & 0.017 (0.033) \\
            & \texttt{MR.RGM\_NoConf} & 0.218 (0.018) & 0.042 (0.003) & 0.004 (0.0004) \\
            % & \texttt{GRIVET} & 0.093 (0.015) & 0.016 (0.006) & 0.002 (0.001) \\
            & \texttt{MR-SimpleMedian}   & 0.074 (0.015) & 0.021 (0.002) & 0.001 (0.0001) \\
            & \texttt{MR-WeightedMedian} & 0.074 (0.014) & 0.021 (0.002) & 0.001 (0.0001) \\
            & \texttt{MR-IVW}            & 0.296 (0.014) & 0.032 (0.002) & 0.004 (0.0003) \\
            & \texttt{OneSampleMR}       & 0.282 (0.015) & 0.031 (0.002) & 0.004 (0.0003) \\
            & \texttt{mrbayes}           & 0.296 (0.015) & 0.032 (0.002) & 0.004 (0.0003) \\
\hline
n = 30000   & \texttt{MR.RGM}         & 0.324 (0.015) & 0.024 (0.002) & 0.005 (0.0005) \\
            & \texttt{MR.RGM+}        & 0.351 (0.812) & 0.013 (0.020) & 0.012 (0.033) \\
            & \texttt{MR.RGM\_NoConf} & 0.214 (0.018) & 0.042 (0.003) & 0.004 (0.0002) \\
            % & \texttt{GRIVET} & 0.093 (0.015) & 0.016 (0.007) & 0.001 (0.001) \\
            & \texttt{MR-SimpleMedian}   & 0.044 (0.006) & 0.013 (0.002) & 0.0003 (0.0001) \\
            & \texttt{MR-WeightedMedian} & 0.044 (0.006) & 0.013 (0.002) & 0.0003 (0.0001) \\
            & \texttt{MR-IVW}            & 0.283 (0.014) & 0.026 (0.001) & 0.004 (0.0002) \\
            & \texttt{OneSampleMR}       & 0.268 (0.013) & 0.025 (0.001) & 0.004 (0.0002) \\
            & \texttt{mrbayes}           & 0.282 (0.014) & 0.026 (0.001) & 0.004 (0.0002) \\
\hline
\end{tabular}
\end{table}

\begin{figure}[htb]
    \centering
    \includegraphics[width=.7\textwidth]{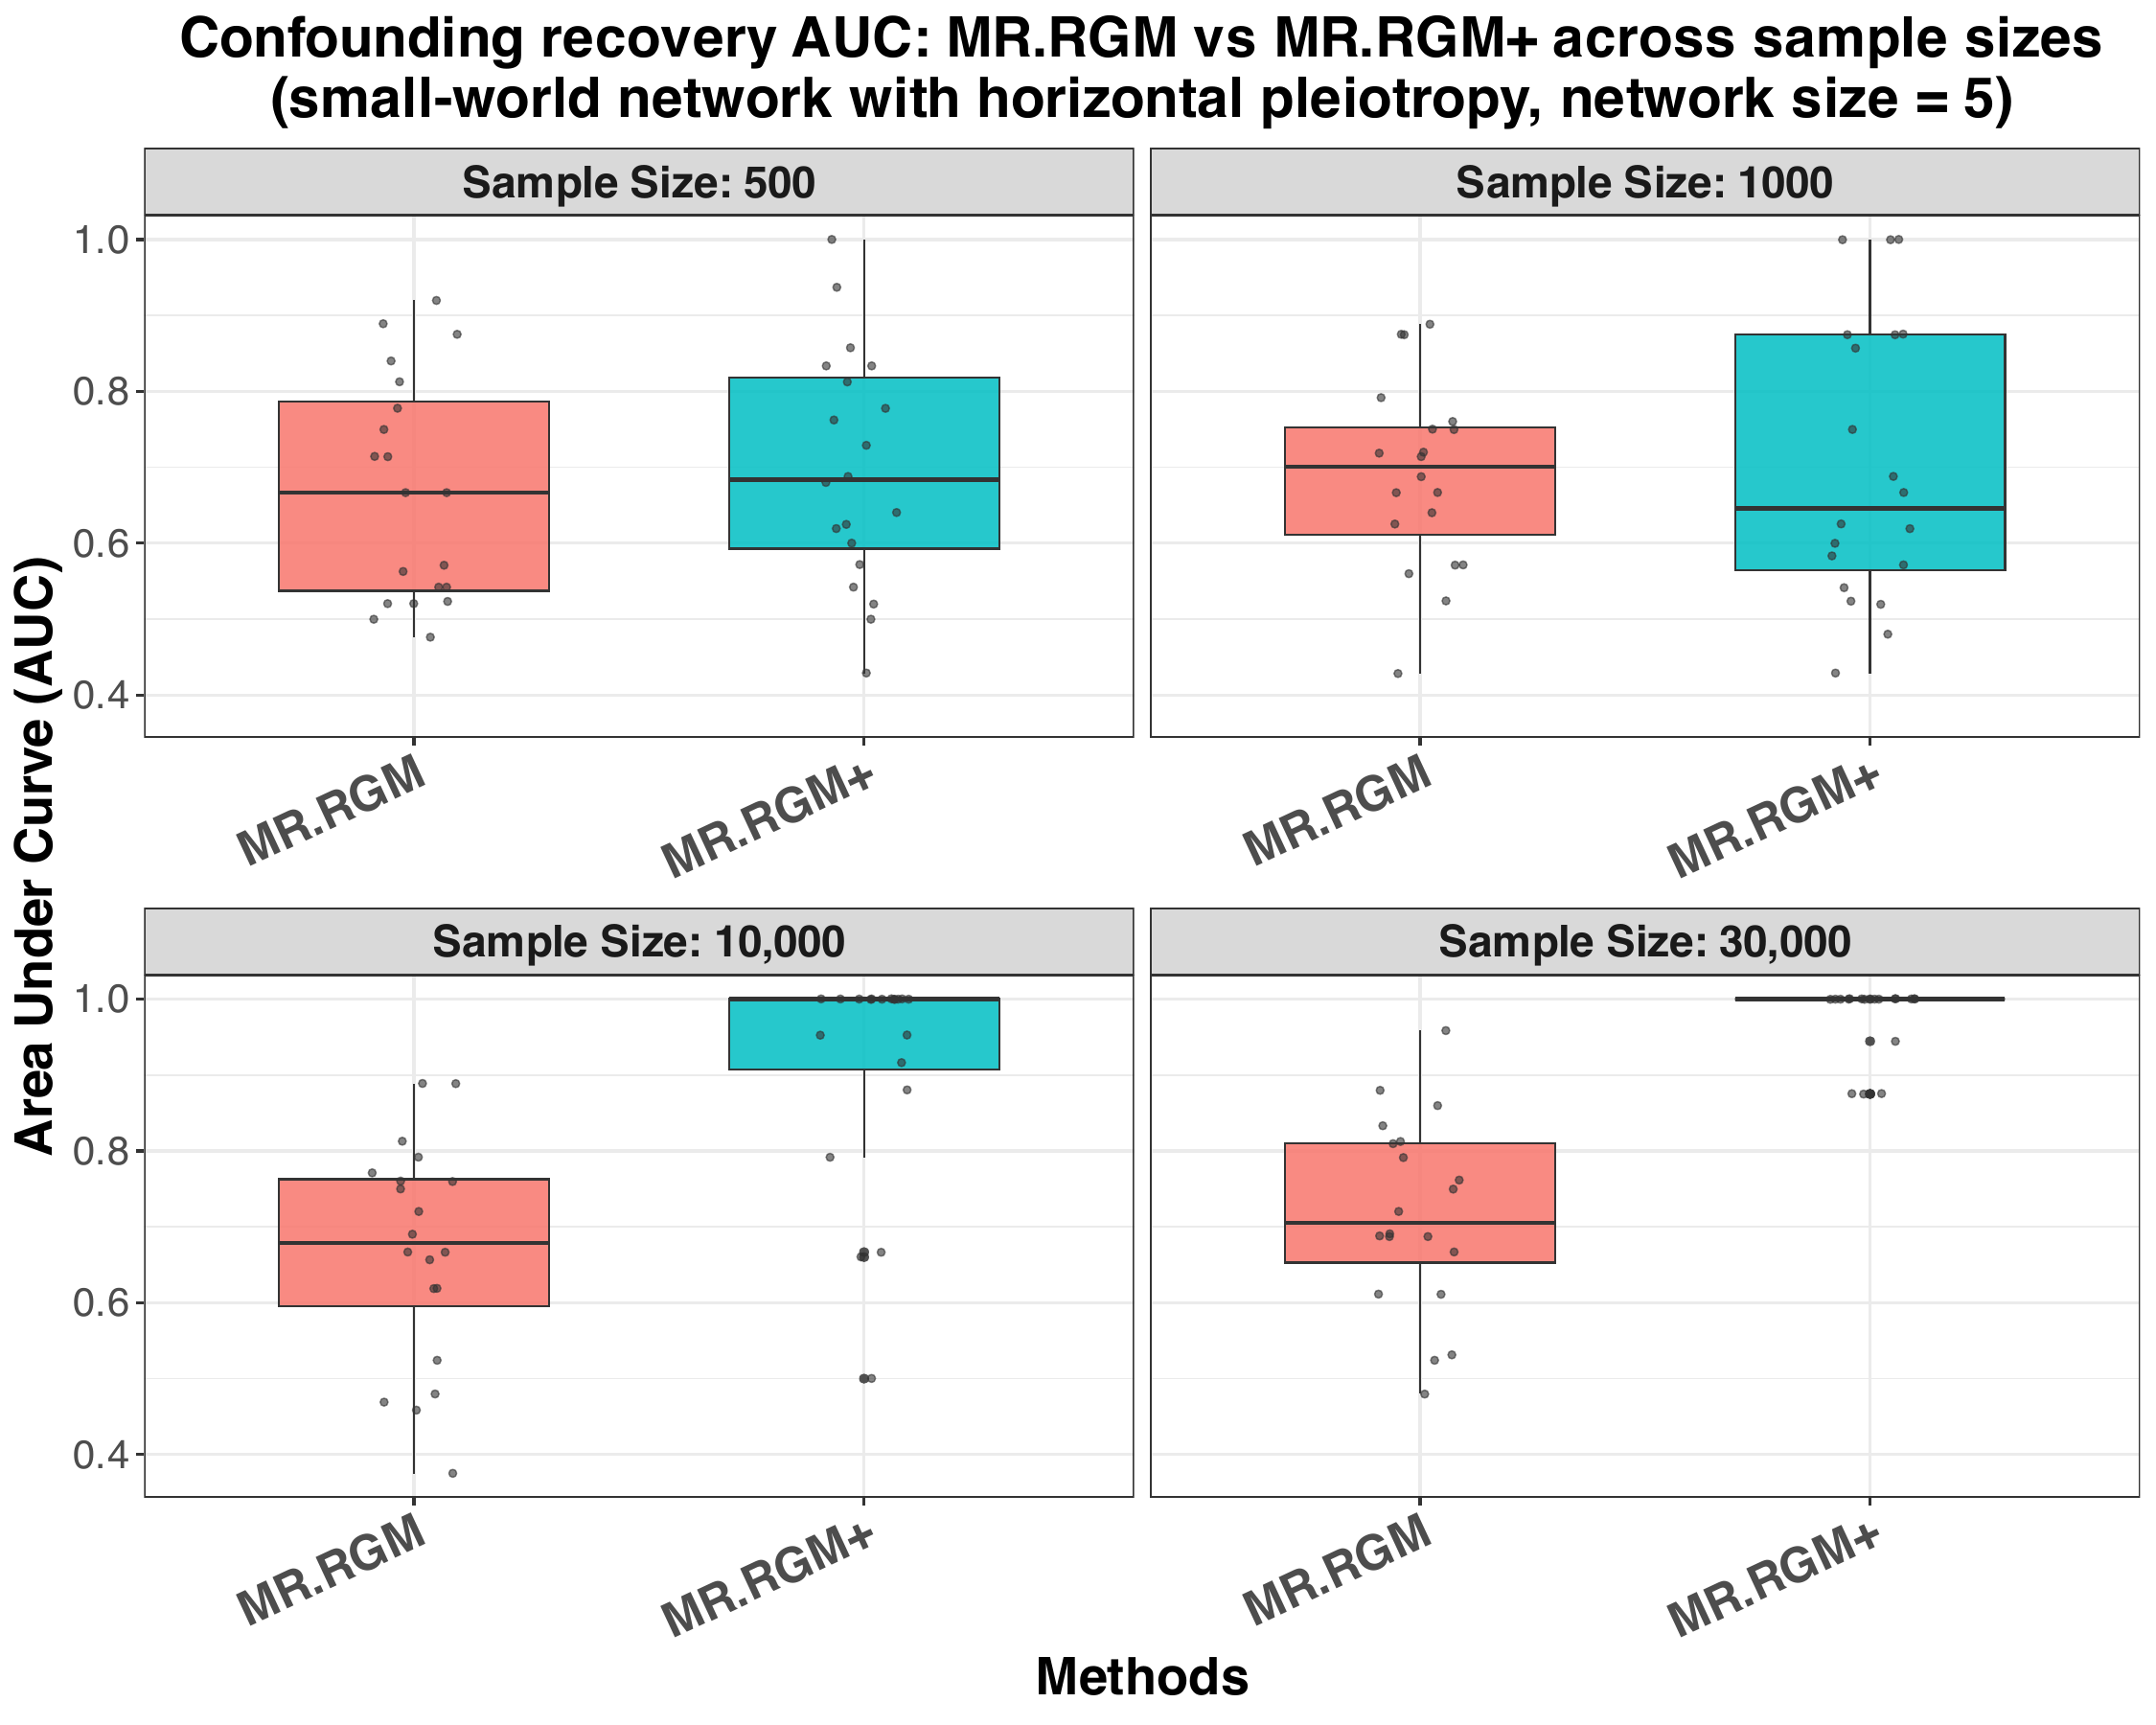}
    \caption{Confounding structure recovery performance using \texttt{MR.RGM} and \texttt{MR.RGM+} in a small-world network with feedback loops, unmeasured confounding, and horizontal pleiotropy, with network size \(p{=}5\). Boxplots of AUC by method (x-axis) and sample size (facets; \(n \in \{500,1000,10000,30000\}\)).}
    \label{fig:swp_conf_p5}
\end{figure}

\begin{table}[htb]
\centering
\small
\caption{Confounding structure recovery performance using \texttt{MR.RGM} in a small-world network with feedback loops, unmeasured confounding, and horizontal pleiotropy, across network sizes \(p\in\{5,10\}\).}
\label{tab:feedback_conf_auc_smallworld_horizontal_A}
\begin{tabular}{|c|c|c|c|c|c|}
\hline
\textbf{Setting} & \textbf{Sample Size} & \textbf{AUC} & \textbf{TPR} & \textbf{FDR} & \textbf{MCC}\\
\hline
% \multirow{4}{*}{p = 5, Var = 97\%} 
%     & 500  & 0.675 & 0.546 & 0.706 & -0.067 \\
%     & 1000 & 0.665 & 0.551 & 0.755 & -0.280 \\
%     & 10000 & 0.621 & 0.543 & 0.710 & -0.121 \\
%     & 30000 & 0.628 & 0.674 & 0.681 & 0.023 \\
\hline
\multirow{4}{*}{p = 5} 
    & 500 & 0.669 (0.143) & 0.415 (0.307) & 0.537 (0.296) & 0.082 (0.336) \\
    & 1000 & 0.689 (0.119) & 0.505 (0.292) & 0.526 (0.253) & 0.105 (0.357) \\
    & 10000 & 0.668 (0.142) & 0.888 (0.166) & 0.470 (0.278) & 0.351 (0.278) \\
    & 30000 & 0.718 (0.123) & 0.919 (0.143) & 0.473 (0.283) & 0.371 (0.297) \\
% \hline
% \multirow{4}{*}{p = 10, Var = 97\%} 
%     & 500  & 0.568 & 0.313 & 0.662 & -0.183 \\
%     & 1000 & 0.584 & 0.380 & 0.662 & -0.187 \\
%     & 10000 & 0.621 & 0.420 & 0.630 & -0.111 \\
%     & 30000 & 0.738 & 0.600 & 0.585 & 0.041 \\
\hline
\multirow{4}{*}{p = 10} 
    & 500 & 0.618 (0.095) & 0.306 (0.121) & 0.365 (0.213) & 0.136 (0.129) \\
    & 1000 & 0.677 (0.053) & 0.432 (0.074) & 0.320 (0.187) & 0.222 (0.086) \\
    & 10000 & 0.841 (0.055) & 0.890 (0.086) & 0.255 (0.225) & 0.564 (0.173) \\
    & 30000 & 0.860 (0.065) & 0.952 (0.055) & 0.289 (0.233) & 0.577 (0.194) \\
\hline
\end{tabular}
\end{table}

\begin{table}[htb]
\centering
\small
\caption{Confounding structure recovery performance using \texttt{MR.RGM+} in a small-world network with feedback loops, unmeasured confounding, and horizontal pleiotropy, across network sizes \(p\in\{5,10\}\).}
\label{tab:feedback_conf_auc_smallworld_horizontal_B}
\begin{tabular}{|c|c|c|c|c|c|}
\hline
\textbf{Setting} & \textbf{Sample Size} & \textbf{AUC} & \textbf{TPR} & \textbf{FDR} & \textbf{MCC}\\
\hline
% \hline
% \multirow{4}{*}{p = 5, Var = 97\%} 
%     & 500  & 0.657 & 0.639 & 0.698 & -0.044 \\
%     & 1000 & 0.746 & 0.577 & 0.757 & -0.278 \\
%     & 10000 & 0.685 & 0.494 & 0.678 & -0.001 \\
%     & 30000 & 0.824 & 0.547 & 0.564 & 0.149 \\
\hline
\multirow{4}{*}{p = 5} 
    & 500 & 0.698 (0.149) & 0.327 (0.288) & 0.403 (0.402) & 0.203 (0.347) \\
    & 1000 & 0.704 (0.181) & 0.506 (0.290) & 0.360 (0.305) & 0.292 (0.283) \\
    & 10000 & 0.916 (0.142) & 0.881 (0.178) & 0.321 (0.327) & 0.574 (0.270) \\
    & 30000 & 0.978 (0.045) & 1.000 (0.000) & 0.311 (0.358) & 0.694 (0.351) \\
% \hline
% \multirow{4}{*}{p = 10, Var = 97\%} 
%     & 500  & 0.587 & 0.296 & 0.667 & -0.190 \\
%     & 1000 & 0.581 & 0.380 & 0.653 & -0.164 \\
%     & 10000 & 0.721 & 0.362 & 0.582 & -0.037 \\
%     & 30000 & 0.813 & 0.480 & 0.564 & 0.034 \\
\hline
\multirow{4}{*}{p = 10} 
    & 500 & 0.685 (0.096) & 0.233 (0.116) & 0.236 (0.208) & 0.205 (0.138) \\
    & 1000 & 0.733 (0.066) & 0.352 (0.102) & 0.183 (0.177) & 0.315 (0.107) \\
    & 10000 & 0.938 (0.085) & 0.866 (0.086) & 0.174 (0.259) & 0.660 (0.243) \\
    & 30000 & 0.950 (0.097) & 0.994 (0.020) & 0.162 (0.290) & 0.824 (0.297) \\
\hline
\end{tabular}
\end{table}

\begin{figure}[htb]
    \centering
    \includegraphics[width=.7\textwidth]{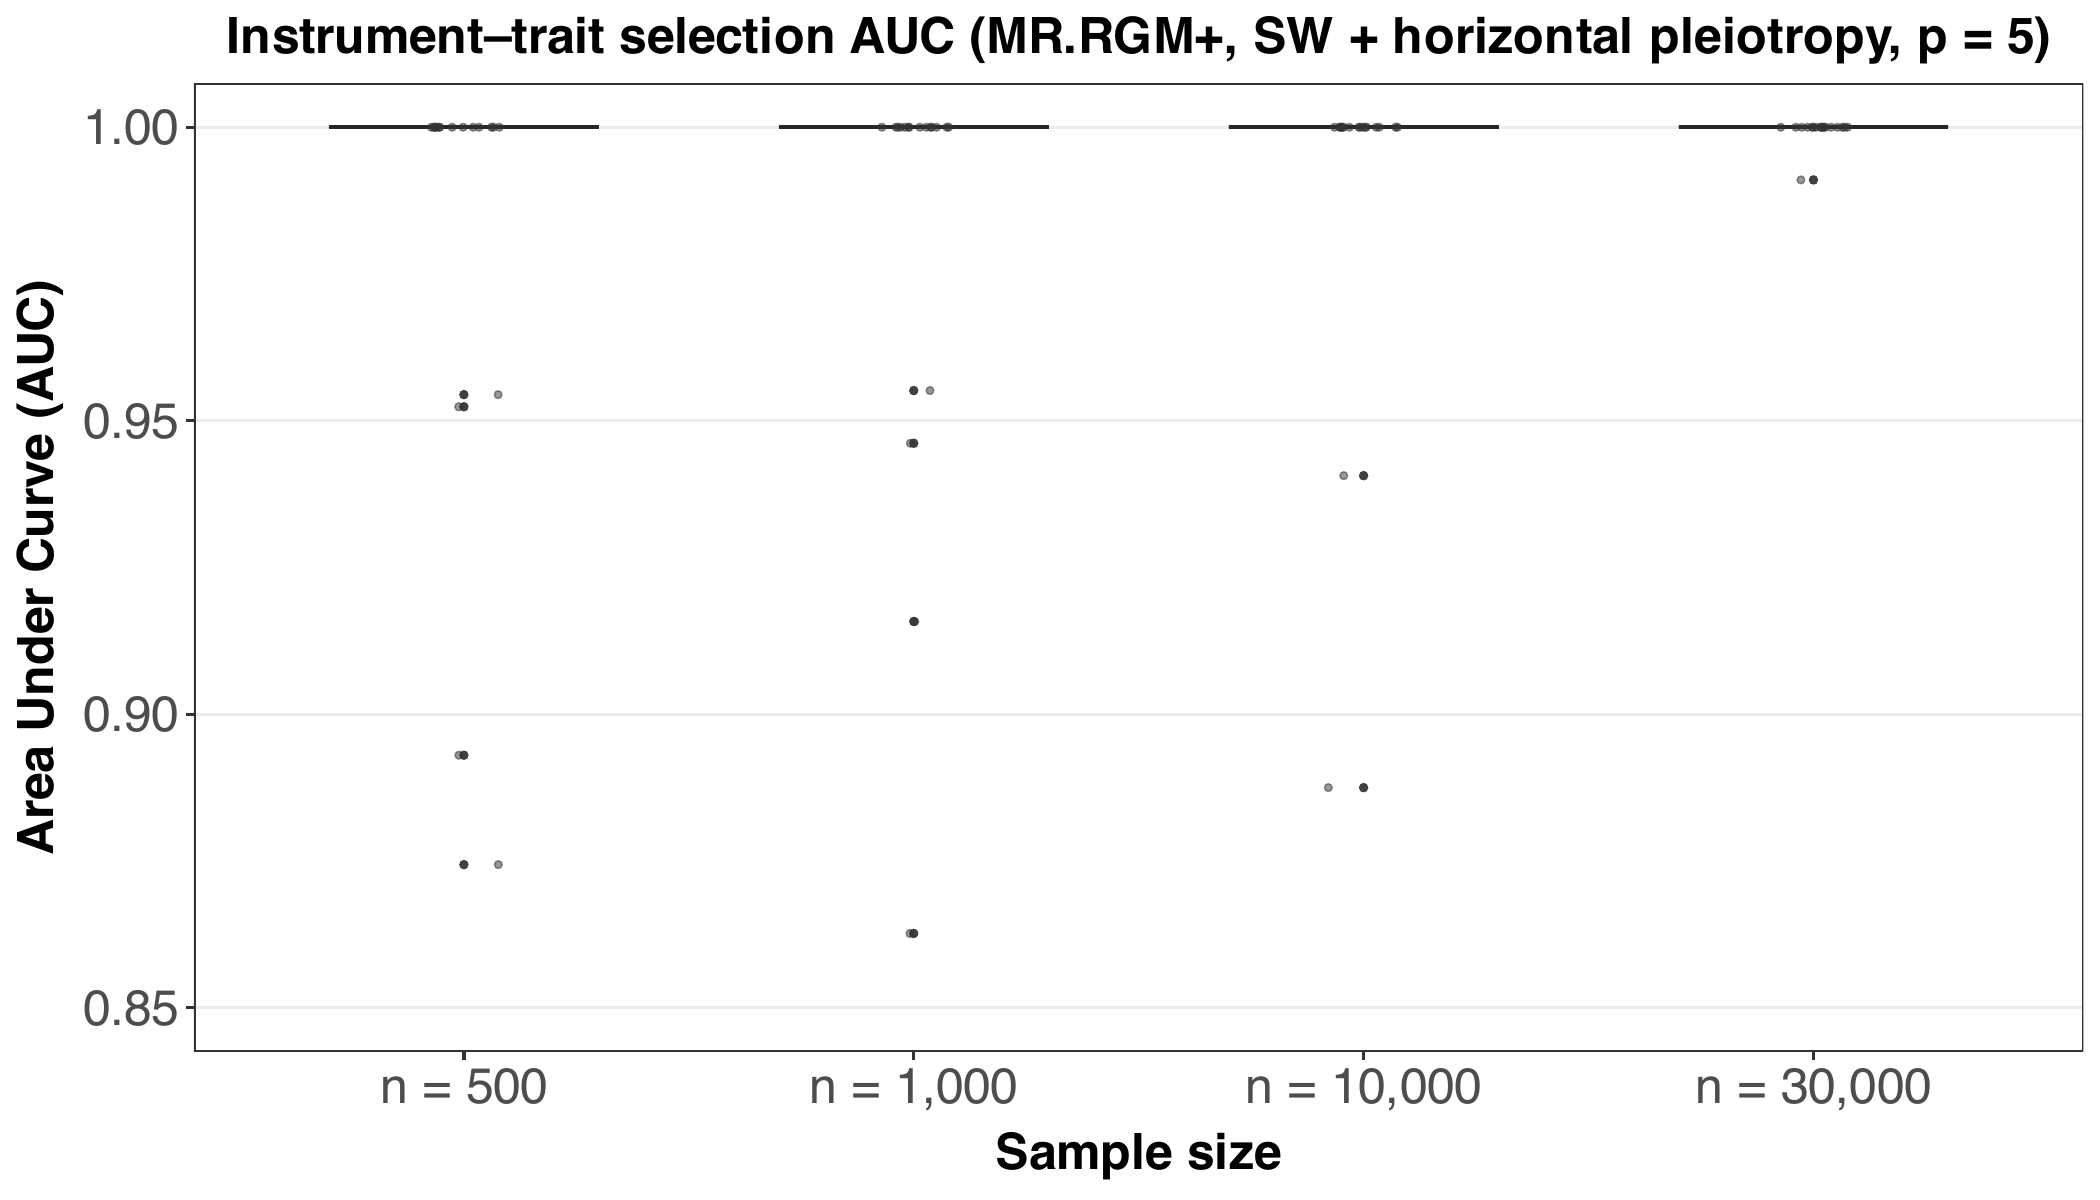}
    \caption{Instrument-trait selection performance using \texttt{MR.RGM+} in a small-world network with feedback loops, unmeasured confounding, and horizontal pleiotropy, with network size \(p{=}5\).
    Boxplots of AUC across sample sizes (\(n \in \{500,1000,10000,30000\}\)).}
    \label{fig:snp_auc_sw_p5}
\end{figure}

\FloatBarrier
\bibliographystyle{plain}  % or use unsrt, apalike, etc.
\bibliography{Bibliography-MM-MC}  % without the .bib extension

\end{document}
